# Supplementary material for: Rapid Vector-based Any-angle Path Planning with Non-convex Obstacles
Source: arXiv:2408.05806 source file (2024-08-11)
Supplement: Supplementary file 1 [file _tex_suppr2p.tex]

\onecolumn
% \section{Supplementary Material: \rtwop{}}
\chapter{Implementation for \rtwop{}}
\label{chap:suppr2p}
\setcounter{algorithm}{0}

\setcounter{equation}{0}
\setcounter{figure}{0}
\setcounter{table}{0}
\makeatletter
\renewcommand\paragraph{\@startsection{paragraph}{4}{\z@}
                         {2ex \@plus .1ex \@minus .2ex}%
                         {.1ex \@plus .0ex}%1.5ex \@plus .2ex}%
                         {\normalfont\normalsize\itshape}}
\setcounter{secnumdepth}{4}% Number up to paragraphs
\makeatother

% \tableofcontents

\section{Introduction}
This supplementary material attempts to describe the implementation details of \rtwop{}.

\subsection{Pseudocode Convention}
The pseudocode is Python-like and all objects are passed by reference.
Class objects are usually represented by tuples $(\cdot)$. If an object is a collection of other objects, they are usually represented by ordered sets $\{\cdot\}$ unless otherwise specified.
To access a member of an object, the emboldened period operator ($\mdot$) is used.
If an object is an ordered set, its elements can be accessed with the square bracket operator $[\cdot]$, with 1 begin the first element.

The reader may need to keep in mind any memory invalidation that can occur, such as iterator invalidations, when an object is removed from a set in the pseudocode.
The reader is encouraged to cache repeated calculations.

%%%%%%%%%%%%%%%%%%%%%%%%%%%% COMMON NOMENCLATURE %%%%%%%%%%%%%%%%%%%%%%%%%%%%%%%%%%%%%%%%%%%%%
\subsection{Common Nomenclature}
\rtwop{} is an any-angle 2D path planner that finds the shortest path between two points, the \textbf{start} and \textbf{goal} points.
\rtwop{} searches from the start point, and returns the shortest path if it exists.
The shortest path is a set of coordinates that begins from the goal point and ends at the start point. Intermediate points are turning points of the any-angle path, and may include colinear points.

\rtwop{} relies on two trees of nodes in the search process. 
The \textbf{source-tree} ($S$-tree) is rooted at the start node, which lies on the start point, while the \textbf{target-tree} ($T$-tree) is rooted at the goal node, which lies on the goal point.
Each tree branches from its root node, and is ``joined" to each other at their leaf nodes.

A link is a branch on the tree that connects two nodes. 
For efficient memory management, a link points to only one node (\textbf{anchored} at a node).
A link can be connected to other links anchored at other nodes, indirectly connecting the nodes.
While a node forms a vertex of an examined path, a link forms a segment of the path.
By storing information specific to a path being expanded, a link reduces duplicate line-of-sight checks between nodes of overlapping paths.

A \textbf{query} is used to describe an intermediate expansion. The query has an associated path cost estimate and can be queued into the open-list.
In A*, a query can be thought of as an iteration, which expands a node and examines the neighboring nodes.
In \rtwop{}, a query expands a link, performing a line-of-sight check over the link (\textbf{casting query}, or \textbf{cast}), or traces an obstacle contour beginning from the link (\textbf{tracing query}, or \textbf{trace}).
The link that is being expanded is anchored on a leaf node (\textbf{leaf link}) of the $S$-tree or $T$-tree.
A query and its expanded leaf link point to each other. As such, a query can be found between a pair of connected leaf nodes.

The \textbf{source-direction} refers to the direction leading to the start node along the path formed by the links and nodes, while the \textbf{target-direction} refers to the direction leading to the goal node. 
The terms are applied to objects when describing their location in relation to other objects.
For example, a link indirectly connects two nodes. The node leading to the start node is called the \textbf{source node} of the link, while the node leading to the goal node is called the \textbf{target node}.
Let $\mtdir \in \{S,T\}$ be the tree-direction where $S=-1$ and $T=1$ denote the source and target-direction respectively.
Nodes in the source tree (\textbf{source-tree nodes}) lie in the source direction of a query, while nodes in the the target tree (\textbf{target-tree nodes}) lie in the target direction of a query.
A \textbf{parent} node or link of an object lies closer to the root node of a tree than the object. 
For example, a parent node or link of a source-tree node lies in the source-direction of the source-tree node.
A \textbf{child} node lies further away from the root node.
For example, a child node or link of a target-tree node lies in the source-direction of the target-tree node.

When a cast collides with an obstacle, a \textbf{left} and \textbf{right} trace occurs from the left and right side of the collision point respectively. 
The traces trace the obstacle's contour, placing nodes along the contours. 
A node has a side that is the same as the trace that found it -- a left-sided node is placed by a left trace, etc.
Let $\mside \in \{L,R\}$ be the side where $L=-1$ and $R=1$ denote the left and right side respectively.

% Fig. \ref{suppfig:tree} illustrates the trees, nodes, links, and queries. 

%%%%%%%%%%%%%%%%%%%%%%%%%%%% DATA STRUCTURES AND METHODS %%%%%%%%%%%%%%%%%%%%%%%%%%%%%%%%%%%%%%%%%%%%%
\section{Data Structures and Methods}
\setcounter{algorithm}{0}

This section describes the objects, or data structures, used in \rtwop{}.
The subsections contain functions which are sorted into three categories.
The first category contains helper functions, denoted by a single letter, to access members or owners of an object.
The second category contains a constructor or initializer, which is prefixed with \textit{Get} or \textit{Create}.
The third category contains functions that interface with other objects. 
The material includes only noteworthy functions, and the functions are non-exhaustive.

%%%%%%%%%%%%%%%%%%%%%%%%%%%% POSITION & BEST %%%%%%%%%%%%%%%%%%%%%%%%%%%%%%%%%%%%%%%%%%%%%
\subsection{Position and Best Objects}
A position object $\mpos$ describes the best cost and direction to reach a position, and owns any nodes placed at the location.
It is described by
\begin{equation}
\mpos = (\mx, \mnodes, \mbest_S, \mbest_T),
\end{equation}
where $\mx$ is the pair of coordinates, and $\mnodes$ is a set containing nodes.
$\mbest_S$ and $\mbest_T$ contain information about the best cost and direction to $\mx$ from the source and target direction respectively, and are described by
\begin{equation}
    \mbest = (\mcost, \mnodebest, \mxpar).
\end{equation}
$\mcost$ is the smallest cost known so far to reach the current position $\mpos$. 
For $\mbest_S$, the cost is cost-to-come, and for $\mbest_T$, the cost is cost-to-go.
$\mnodebest$ indicates the node $\mnode$ at the current location which has the shortest, unobstructed path to the root node. The root node is the start or goal node for $\mbest_S$ or $\mbest_T$ respectively.
For $\mbest_S$, $\mxbest$ is the location of the source node along the path. 
For $\mbest_T$, $\mxbest$ is the location of the target node along the path.

%%%%%%%%%%%%%%%%%%%%%%%%%%%%%%%% FBEST %%%%%%%%%%%%%%%%%%%%%%%%%%%%%%%%%%
\subsubsection{\textproc{$\fbest$}: \textit{Gets a Best Member Object of a Position Object}}
The helper function $\fbest$ (Alg. \ref{suppalg:fbest}) returns $\mbest_S$ or $\mbest_T$ depending on the tree-direction $\mtdir\in\{S,T\}$.
\begin{algorithm}[!ht]
\begin{algorithmic}[1]
\caption{$\fbest$: gets Best property of Position object.}
\label{suppalg:fbest}
\Function{$\fbest$}{$\mtdir, \mpos$}
    \State \Return $\mpos\mdot\mbest_S$ \textbf{if} $\mtdir = S$ \textbf{else} $\mpos\mdot\mbest_T$
\EndFunction
\end{algorithmic}
\end{algorithm}

%%%%%%%%%%%%%%%%%%%%%%%%%%%%%%%% GETPOS %%%%%%%%%%%%%%%%%%%%%%%%%%%%%%%%%%
\subsubsection{\textproc{GetPos}: \textit{Retrieves or Constructs a Position Object}}
The function \textproc{GetPos} (Alg. \ref{suppalg:getpos}) returns $\mpos$ if it exists at a corner at $\mx$. Otherwise, it creates a new $\mpos$ at $\mx$ and returns it.

\begin{algorithm}[!ht]
\begin{algorithmic}[1]
\caption{\textproc{GetPos}: gets or creates Position object.}
\label{suppalg:getpos}
\Function{GetPos}{$\mx$}
    \State Try getting $\mpos = (\mx, \cdots )$ from a corner at $\mx$. 
    \If {$\mpos$ does not exist}
        \State Create $ \mpos = (\mx, \{\}, \infty, \varnothing, \infty, \varnothing)$ \Comment{$\mx_g$ and $\mx_h$ can be initialised to any value.}
    \EndIf
    \State \Return $\mpos$
\EndFunction
\end{algorithmic}
\end{algorithm}

%%%%%%%%%%%%%%%%%%%%%%%%%%%% NODE %%%%%%%%%%%%%%%%%%%%%%%%%%%%%%%%%%%%%%%%%%%%%
\subsection{Node and Node Types}
A node $\mnode$ is described by
\begin{equation}
\mnode = ( \mntype, \msidenode, \mtdirnode, \mlinks_\mnode ),
\end{equation}
which has a side $\msidenode \in \{L, R\}$ that has the same side as the trace that placed it. 
The node is a \textbf{source-tree node} or a \textbf{target-tree node} if $\mtdirnode = S$ or $\mtdirnode = T$ respectively. 
$\mlinks_\mnode$ refers to an unordered set of links anchored at the node $\mnode$. 

The node types for \rtwop{} are $\mntype \in \{ \mnvy, \mnvu, \mney, \mneu, \mnun, \mnoc, \mntm \}$, and are different from the node types used in \rtwo{}. 
The node types are described in Table \ref{r2p:tab:nodetypes}. 
Table \ref{supptab:nodetypes2} indicate if two nodes can be indirectly connected with a link. 
The connections are derived from the algorithm's logic, and \rtwop{} does not follow any explicit rule to connect nodes.

Any node with \textbf{cumulative visibility} to another node has an unobstructed path between them. As only the cumulative visibility to the start node or goal node is important, the definition of cumulative visibility is overloaded in the text for brevity --
if a source-tree node or target-tree node has \textbf{cumulative visibility}, then the node has cumulative visibility to the start node or goal node respectively.

\begin{table*}[!ht]
\centering
\caption{Node types and possible parent types.}
\begin{tabular}{ c | c c c c c c c c | p{7cm} }
\diagbox{$\mntype$}{$\mntype_\mtdir$} & $\mnvy$ & $\mnvu$ & $\mney$ & $\mneu$ & $\mnun$ & $\mnoc$ & $\mntm$ & \multirow{9}{7cm}{
\footnotesize
Alphabet(s) $S$ and/or $T$ are placed if a node of type $\mntype$ and a parent node of type $\mntype_\mtdir$ can be connected to each other with a link. $S$ is placed if both nodes are in the source tree and the nodes can be connected, $T$ if both nodes are in the target tree and the nodes can be connected. For example, a $\mnvy$ node and a parent $\mnvy$ node can connect regardless of the tree they lie in, and a $\mnvu$ node and a parent $\mnun$ node can be connected only if they are in the target tree. The connections are derived from the algorithm, and \rtwop{} does not follow any explicit connection rule.
}
\\
\cline{1-8}
$\mnvy$ & $S,T$ & -- & -- & -- & -- & -- & -- & -- & \\
\cline{1-8}
$\mnvu$ & $S,T$ & $S,T$ & -- & -- & $T$ & $T$ & $T$ & \\
\cline{1-8}
$\mney$ & $S,T$ & -- & $S,T$ & -- & -- & -- & -- &\\
\cline{1-8}
$\mneu$ & -- & -- & $S$ & $S$ & -- & -- & -- & \\
\cline{1-8}
$\mnun$ & $T$ & $T$ & -- & -- & -- & -- & $T$  &\\
\cline{1-8}
$\mnoc$ & $T$ & $T$ & $T$ & -- & $T$ & -- & $T$  &\\
\cline{1-8}
% $\mnph$ & $T$ & $T$ & $T$ & -- & $T$ & $T$ & $T$ & $T$ & \\
\cline{1-8}
$\mntm$ & $T$ & $T$ & $T$ & -- & $T$ & $T$ & $T$ & \\

\end{tabular}
\label{supptab:nodetypes2}
\end{table*}

%%%%%%%%%%%%%%%%%%%%%%%%%%%%%%%%% ALG: FPOS %%%%%%%%%%%%%%%%%%%%%%%%%%%%%%%%%%%%%
\subsubsection{\textproc{$\fpos$}: \textit{Gets Position Object that Owns a Node}}
\textproc{$\fpos$} (Alg. \ref{suppalg:fpos}) returns the position object owning the node $\mnode$ .
\begin{algorithm}[!ht]
\begin{algorithmic}[1]
\caption{$\fpos$: gets Position object containing node.}
\label{suppalg:fpos}
\Function{$\fpos$}{$\mnode$}
    \State \Return $\mpos$ where $\mnode \in \mpos\mdot\mnodes$
\EndFunction
\end{algorithmic}
\end{algorithm}

%%%%%%%%%%%%%%%%%%%%%%%%%%%%%%%%% ALG: FX %%%%%%%%%%%%%%%%%%%%%%%%%%%%%%%%%%%%%
\subsubsection{\textproc{$\fx$}: \textit{Gets Coordinates of a Node}}
\textproc{$\fx$} (Alg. \ref{suppalg:fx}) returns the coordinates of $\mnode$.
\begin{algorithm}[!ht]
\begin{algorithmic}[1]
\caption{$\fx$: gets coordinates of a node.}
\label{suppalg:fx}
\Function{$\fx$}{$\mnode$}
    \State \Return \Call{$\fpos$}{$\mnode$}$\mdot\mx$
\EndFunction
\end{algorithmic}
\end{algorithm}

%%%%%%%%%%%%%%%%%%%%%%%%%%%%%%%%% ALG: GETNODE %%%%%%%%%%%%%%%%%%%%%%%%%%%%%%%%%%%%%
\subsubsection{\textproc{GetNode}: \textit{Retrieves or Constructs a Node}}
The function \textproc{GetNode} (Alg. \ref{suppalg:getnode}) gets a matching node with type $\mntype$, side $\mside_\mnode$ and tree $\mtdir_\mnode$ from a corner at $\mx$ if it exists. 
Otherwise, a new node is created.
\begin{algorithm}[!ht]
\begin{algorithmic}[1]
\caption{\textproc{GetNode}: gets or creates existing node.}
\label{suppalg:getnode}
\Function{GetNode}{$\mx$, $\mntype$, $\mside_\mnode$, $\mtdir_\mnode$}
    \State $\mpos \gets $ \Call{GetPos}{$\mx$}
    \State Try finding $\mnode = (\mntype, \mside_\mnode, \mtdir_\mnode, \cdots)$ from $\mpos \mdot \mnodes$.
    \If{ $\mnode$ does not exist}
        \State Create $\mnode = (\mntype, \mside_\mnode, \mtdir_\mnode, \{\})$
    \EndIf
    \State \Return $\mnode$
\EndFunction
\end{algorithmic}
\end{algorithm}

%%%%%%%%%%%%%%%%%%%%%%%%%%%% LINK %%%%%%%%%%%%%%%%%%%%%%%%%%%%%%%%%%%%%%%%%%%%%
\subsection{Link}
A link $\mlink$ is described by
\begin{equation}
\mlink = ( \mlinks_S, \mlinks_T, \mcost, \mray_L, \mray_R ),
\end{equation}
where $\mlinks_S$ and $\mlinks_T$ are unordered sets containing links in the source and target-direction of the link respectively. 
$\mcost$ is the cost-to-come if the link's anchored node is a source-tree node, or cost-to-go if the anchored node is a target-tree node. 
$\mray_L$ is the left sector-ray, and $\mray_R$ is the right sector-ray.

%%%%%%%%%%%%%%%%%%%%%%%%%%%%%%%%% ALG: FX %%%%%%%%%%%%%%%%%%%%%%%%%%%%%%%%%%%%%
\subsubsection{\textproc{$\fnode$}: \textit{Gets Anchored Node of a Link}}
\textproc{$\fnode$} (Alg. \ref{suppalg:fnode}) returns the anchored node of a link $\mlink$.
\begin{algorithm}[!ht]
\begin{algorithmic}[1]
\caption{$\fnode$: gets the anchored node of a link.}
\label{suppalg:fnode}
\Function{$\fnode$}{$\mlink$}
    \State \Return $\mnode$ where $\mlink \in \mnode\mdot\mlinks_\mnode$
\EndFunction
\end{algorithmic}
\end{algorithm}

%%%%%%%%%%%%%%%%%%%%%%%%%%%%%%%%% ALG: FRAY %%%%%%%%%%%%%%%%%%%%%%%%%%%%%%%%%%%%%
\subsubsection{\textproc{$\fray$}: \textit{Gets Sector-ray of a Link}}
\textproc{$\fray$} (Alg. \ref{suppalg:fray}) returns the $\mside$-sided ($\mside\in\{L, R\}$) sector-ray of a link $\mlink$.
\begin{algorithm}[!ht]
\begin{algorithmic}[1]
\caption{$\fray$: gets a sector-ray stored in a link.}
\label{suppalg:fray}
\Function{$\fray$}{$\mside, \mlink$}
    \State \Return $\mlink\mdot\mray_L$ \textbf{if} $\mside = L$ \textbf{else} $\mlink\mdot\mray_R$
\EndFunction
\end{algorithmic}
\end{algorithm}

%%%%%%%%%%%%%%%%%%%%%%%%%%%%%%%%% ALG: FLINKS %%%%%%%%%%%%%%%%%%%%%%%%%%%%%%%%%%%%%
\subsubsection{\textproc{$\flinks$}: \textit{Gets a Set of Connected Links}}
\textproc{$\flinks$} (Alg. \ref{suppalg:flinks}) returns the set of $\mtdir$-direction links ($\mtdir \in \{S,T\}$) of a link $\mlink$.
\begin{algorithm}[!ht]
\begin{algorithmic}[1]
\caption{$\flinks$: gets the set of source or target links of a link.}
\label{suppalg:flinks}
\Function{$\flinks$}{$\mtdir, \mlink$}
    \State \Return $\mlink\mdot\mlinks_L$ \textbf{if} $\mside = L$ \textbf{else} $\mlink\mdot\mlinks_R$
\EndFunction
\end{algorithmic}
\end{algorithm}

%%%%%%%%%%%%%%%%%%%%%%%%%%%%%%%%% ALG: FLINK %%%%%%%%%%%%%%%%%%%%%%%%%%%%%%%%%%%%%
\subsubsection{\textproc{$\flink$}: \textit{Gets a Connected Link}}
\textproc{$\flink$} (Alg. \ref{suppalg:flink}) returns \textit{any one} link in the $\mtdir$-direction. \textproc{$\flink$}$(\cdot)$ is commonly used to access the parent node of a link. 
As most links only point to one parent link, the function is also commonly used.
\begin{algorithm}[!ht]
\begin{algorithmic}[1]
\caption{$\flink$: gets any one source or target link of a link.}
\label{suppalg:flink}
\Function{$\flink$}{$\mtdir, \mlink$}
    \State Any one link in \Call{$\flinks$}{$\mtdir, \mlink$}
\EndFunction
\end{algorithmic}
\end{algorithm}

%%%%%%%%%%%%%%%%%%%%%%%%%%%%%%%%% ALG: FQUERY %%%%%%%%%%%%%%%%%%%%%%%%%%%%%%%%%%%%%
\newpage
\subsubsection{\textproc{$\fquery$}: \textit{Gets an associated Queued Query}}
\textproc{$\fquery$} returns a queued query (see Sec. \ref{suppsec:queuedquery}) that is associated with a link $\mlink$, if any.
\begin{algorithm}[!ht]
\begin{algorithmic}[1]
\caption{$\fquery$: gets queued query of a link.}
\label{suppalg:fquery}
\Function{$\fquery$}{$\mlink$}
    \State \Return $\mquery$ \textbf{if} there exists a $\mquery$ such that $\mlink = \mquery\mdot\mlink_\mquery$ \textbf{else} $\varnothing$
\EndFunction
\end{algorithmic}
\end{algorithm}

%%%%%%%%%%%%%%%%%%%%%%%%%%%%%%%%% ALG: CREATELINK %%%%%%%%%%%%%%%%%%%%%%%%%%%%%%%%%%%%%
\subsubsection{\textproc{CreateLink}: \textit{Creates a Link}}
The function \textproc{CreateLink} (Alg. \ref{suppalg:createlink}) creates a new link object, anchors it at a node $\mnode$, and returns it.
\begin{algorithm}[!ht]
\begin{algorithmic}[1]
\caption{\textproc{CreateLink}: creates a new link.}
\label{suppalg:createlink}
\Function{CreateLink}{$\mnode$}
    \State Create $\mlink = (\{\}, \{\}, \infty, \varnothing, \varnothing)$
    \State \Call{Anchor}{$\mlink, \mnode$}
    \State \Return $\mlink$
\EndFunction
\end{algorithmic}
\end{algorithm}

%%%%%%%%%%%%%%%%%%%%%%%%%%%%%%%%% ALG: ANCHOR  %%%%%%%%%%%%%%%%%%%%%%%%%%%%%%%%%%%%%
\subsubsection{\textproc{Anchor}: \textit{Anchors a link at a Node}}
The \textproc{Anchor} function (Alg. \ref{suppalg:anchor}) re-anchors a link $\mlink$ from its anchor node to a new node $\mnode_\mnew$. 
\vspace{-0.2cm}
\begin{algorithm}[!ht]
\begin{algorithmic}[1]
\caption{\textproc{Anchor}: transfers link ownership to a node.}
\label{suppalg:anchor}
\Function{Anchor}{$\mlink$, $\mnode_\mnew$} 
    \IfThen{$\fnode(\mlink) \ne \varnothing$} {Remove $\mlink$ from $\fnode(\mlink) \mdot \mlinks_\mnode$}
    \State Add $\mlink$ to $\mnode_\mnew \mdot \mlinks_\mnode$
\EndFunction
\end{algorithmic}
\end{algorithm}

%%%%%%%%%%%%%%%%%%%%%%%%%%%%%%%%% ALG: CONNECT %%%%%%%%%%%%%%%%%%%%%%%%%%%%%%%%%%%%%
\subsubsection{\textproc{Connect}: \textit{Connects Two Links}}
The \textproc{Connect} function  (Alg. \ref{suppalg:connect}) connects two links by adding pointers to each other.
\vspace{-0.2cm}
\begin{algorithm}[!ht]
\begin{algorithmic}[1]
\caption{\textproc{Connect}: Connects two links.}
\label{suppalg:connect}
\Function{Connect}{$\mtdir$, $\mlink$, $\mlink_\mtdir$}
    \State Add $\mlink_\mtdir$ to $\flinks_\mtdir(\mlink)$ 
    \State Add $\mlink$ to $\flinks_{-\mtdir}(\mlink_\mtdir)$ 
\EndFunction
\end{algorithmic}
\end{algorithm}

%%%%%%%%%%%%%%%%%%%%%%%%%%%%%%%%% ALG: DISCONNECT %%%%%%%%%%%%%%%%%%%%%%%%%%%%%%%%%%%%%
\newpage
\subsubsection{\textproc{Disconnect}: \textit{Disconnects Two Links}}
The \textproc{Disconnect} function  (Alg. \ref{suppalg:disconnect}) disconnects two links by removing their pointers from each other.
\begin{algorithm}[!ht]
\begin{algorithmic}[1]
\caption{\textproc{Disconnect}: Disconnects two links.}
\label{suppalg:disconnect}
\Function{Disconnect}{$\mtdir$, $\mlink$, $\mlink_\mtdir$}
    \State Remove $\mlink_\mtdir$ from $\flinks_\mtdir(\mlink)$ 
    \State Remove $\mlink$ from $\flinks_{-\mtdir}(\mlink_\mtdir)$ 
\EndFunction
\end{algorithmic}
\end{algorithm}

%%%%%%%%%%%%%%%%%%%%%%%%%%%%%%%%% ALG: MERGERAY  %%%%%%%%%%%%%%%%%%%%%%%%%%%%%%%%%%%%%
\subsubsection{\textproc{MergeRay}: \textit{Merges a Sector-Ray into a Link}}
The \textproc{MergeRay} function (Alg. \ref{suppalg:mergeray}) replaces the $\mside$-side ray of a link $\mlink$ with $\mray_\mnew$ if the resulting angular-sector becomes smaller.
\begin{algorithm}[!ht]
\begin{algorithmic}[1]
\caption{\textproc{MergeRay}: merges a ray if it shrinks a link's angular-sector.}
\label{suppalg:mergeray}
\Function{MergeRay}{$\mside, \mlink, \mray_\mnew$} 
    \State $\mray_\mathrm{old} \gets \fray(\mside, \mlink)$
    \If {$\mray_\mathrm{old} = \varnothing$}
        \State $\fray(\mside, \mlink) \gets \mray_\mnew$ \Comment{Replace the ray}
    \Else
        \State $\mv_\mathrm{rayOld} \gets \mray_\mathrm{old}\mdot\mx_T - \mray_\mathrm{old}\mdot\mx_S$
        \State $\mv_\mathrm{rayNew} \gets \mray_\mnew\mdot\mx_T - \mray_\mnew\mdot\mx_S$
        \If {$\mside(\mv_\mathrm{rayOld}, \mv_\mathrm{rayNew}) \ge 0$}        
            \State $\fray(\mside, \mlink) \gets \mray_\mnew$ \Comment{Replace the ray}
        \EndIf
    \EndIf
\EndFunction
\end{algorithmic}
\end{algorithm}

%%%%%%%%%%%%%%%%%%%%%%%%%%%%%%%%% ALG: MINCOST %%%%%%%%%%%%%%%%%%%%%%%%%%%%%%%%%%%%%
\subsubsection{\textproc{MinCost}: \textit{Returns the Minimum Cost of Connect Links}}
The function \textproc{MinCost} (Alg. \ref{suppalg:mincost}) finds and returns the minimum cost of a link's ($\mlink$) source or target ($\mtdir \in \{S, T\}$) links. 
The minimum cost does not include the length of the link.
\rtwop{} guarantees that all $\mtdir$ links lie on the same tree when \textproc{MinCost} is used.
\begin{algorithm}[!ht]
\begin{algorithmic}[1]
\caption{\textproc{MinCost}: finds the minimum cost of a link's source or target links.}
\label{suppalg:mincost}
\Function{MinCost}{$\mtdir, \mlink$}
    \State $c_{\min} \gets \infty$
    \For {$\mlink_\mtdir \in \flinks(\mtdir, \mlink)$}
        \If{$c_{\min} > \mlink_\mtdir \mdot c$}
            \State $c_{\min} \gets \mlink_\mtdir \mdot c$
        \EndIf
    \EndFor
    \State \Return $c_{\min}$
\EndFunction
\end{algorithmic}
\end{algorithm}

%%%%%%%%%%%%%%%%%%%%%%%%%%%%%%%%% ALG: COST  %%%%%%%%%%%%%%%%%%%%%%%%%%%%%%%%%%%%%
\subsubsection{\textproc{Cost}: \textit{Returns Cost of a Link}}
The function \textproc{Cost}  (Alg. \ref{suppalg:cost}) finds and reutrns the cost of a link $\mlink$ by adding the minimum cost of the parent links to the length of the link, which is between the link's anchored node and its parent node.
\rtwop{} guarantees that all links lie on the same tree when \textproc{Cost} is used. If $\mlink$ is anchored on an $S$-tree node or $T$-tree node, the cost is cost-to-come or cost-to-go respectively.
\begin{algorithm}[!ht]
\begin{algorithmic}[1]
\caption{\textproc{Cost}: finds the cost of a link.}
\label{suppalg:cost}
\Function{Cost}{$\mlink$}
    \State $\mnode \gets \fnode(\mlink)$
    \State $\mnodepar \gets \fnode(\flink(\mnode\mdot\mtdirnode, \mlink))$
    \State \Return $\lVert \fx(\mnode) - \fx(\mnodepar) \rVert$ + \Call{MinCost}{$\fnode(\mlink), \mlink$} \Comment{$\lVert \cdot \rVert$ denotes the Euclidean L2-norm}
\EndFunction
\end{algorithmic}
\end{algorithm}

%%%%%%%%%%%%%%%%%%%%%%%%%%%%%%%%% ALG: COPYLINK  %%%%%%%%%%%%%%%%%%%%%%%%%%%%%%%%%%%%%
\subsubsection{\textproc{CopyLink}: \textit{Duplicates a Link and its Connections}}
The \textproc{CopyLink} function (Alg.\ref{suppalg:copylink}) duplicates a link $\mlink$ and anchors the duplicated link at a new node $\mnode_\mnew$ if $\mnode_\mnew \ne \varnothing$. 
If $\mnode_\mnew = \varnothing$, $\mnode_\mnew$ defaults to $\fnode(\mlink)$.
The duplicated link is connected to the link's source or target links depending on $\mtdirs$. If $\mtdirs = \{S,T\}$ all links are connected. If $\mtdirs=\{S\}$ or $\mtdirs=\{T\}$ only the source or target links are connected respectively.
\begin{algorithm}[!ht]
\begin{algorithmic}[1]
\caption{\textproc{CopyLink}: copies a link.}
\label{suppalg:copylink}
\Function{CopyLink}{$\mlink, \mnode_\mnew, \mtdirs$}
    \Comment{$\mtdirs \in \{\{S,T\}, \{S\}, \{T\}\}$}
    \If {$\mnode_\mnew = \varnothing$}
        \State $\mnode_\mnew \gets \fnode(\mlink)$
    \EndIf
    \State $\mlink_\mnew \gets $ \Call{CreateLink}{$\mnode_\mnew$}
    \State $\mlink_\mnew\mdot c \gets \mlink\mdot c$
    \State $\mlink_\mnew\mdot\mray_L \gets \mlink\mdot\mray_L$
    \State $\mlink_\mnew\mdot\mray_R \gets \mlink\mdot\mray_R$
    \For {$\mtdir \in \mtdirs$}
        \For {$\mlink_\mtdir \in \flinks(\mtdir, \mlink)$}
            \State \Call{Connect}{$\mtdir, \mlink_\mnew, \mlink_\mtdir$}
        \EndFor
    \EndFor
    \State \Return $\mlink_\mnew$
\EndFunction
\end{algorithmic}
\end{algorithm}

%%%%%%%%%%%%%%%%%%%%%%%%%%%%%%%%% ALG: ISOLATE  %%%%%%%%%%%%%%%%%%%%%%%%%%%%%%%%%%%%%
\subsubsection{\textproc{Isolate}: \textit{Isolates a Link Connection}}
The \textproc{Isolate} function  (Alg. \ref{suppalg:isolate}) tries to isolate the connection between a link $\mlink$ and a $\mtdir$-direction ($\mtdir\in\{S,T\}$) link $\mlink_\mtdir$.
If $\mlink$ is connected to only $\mlink_\mtdir$ in the $\mtdir$-direction, $\mlink$ is returned.
If $\mlink$ is connected to multiple links in the $\mtdir$-direction including $\mlink_\mtdir$, a new link is created that connects only to $\mlink_\mtdir$, and the connection between $\mlink$ and $\mlink_\mtdir$ is removed.
The function helps \rtwop{} to avoid data races between different queries.

$\mnode_\mnew$ is the new anchor node after the isolation. If $\mlink$ is not copied, $\mlink$ is re-anchored at $\mnode_\mnew$. If $\mlink$ is copied, the new link is anchored at $\mnode_\mnew$ instead.
If $\mnode_\mnew$ is not set ($\mnode_\mnew = \varnothing$ ), $\mnode_\mnew$ is defaulted to $\fnode(\mlink)$.
\begin{algorithm}[!ht]
\begin{algorithmic}[1]
\caption{\textproc{Isolate}: isolates a connection between two links.}
\label{suppalg:isolate}
\Function{Isolate}{$\mtdir$, $\mlink$, $\mlink_\mtdir$, $\mnode_\mnew$} \Comment{Note, if $\mlink_\mtdir \ne \varnothing$ then $\mlink_\mtdir \in \flinks_{\mtdir}(\mlink)$}
    \State $numLinks \gets \lvert \flinks_{\mtdir}(\mlink) \rvert$ \Comment{$numLinks$ is the number of links that are in $\mtdir$ direction of $\mlink$}
    \If {($numLinks = 0$ \An $\mlink_\mtdir = \varnothing$) 
        \Or ($numLinks = 1$ \An $\mlink_\mtdir \ne \varnothing$)} 
        \State $\mlink_\mnew \gets \mlink$ \Comment{Nothing to isolate}
    \Else    \Comment{Copy and isolate $(\mlink$, $\mlink_\mtdir)$ connection}
        % \State $\mlink_\mnew \gets (\{\}, \{\}, \mlink \mdot c, \mlink \mdot \mray_L, \mlink \mdot \mray_R)$
        % \State Add $\mlink_\mnew$ to $\fnode(\mlink) \mdot \mlinks_n$
        
        \State $\mlink_\mnew \gets $ \Call{CreateLink}{$\fnode(\mlink)$}
        \State $\mlink_\mnew\mdot c \gets \mlink\mdot c$
        \State $\mlink_\mnew\mdot\mray_L \gets \mlink\mdot\mray_L$
        \State $\mlink_\mnew\mdot\mray_R \gets \mlink\mdot\mray_R$
        
        \For {$\mlink_{-\mtdir} \in \flinks(-\mtdir, \mlink)$}
            \State \Call{Connect}{$-\mtdir$, $\mlink_\mnew$, $\mlink_{-\mtdir}$}
        \EndFor
        \If {$\mlink \ne \varnothing$}
            \State \Call{Connect}{$\mtdir$, $\mlink_\mnew$, $\mlink_\mtdir$}
            \State \Call{Disconnect}{$\mtdir$, $\mlink$, $\mlink_\mtdir$}
        \EndIf
    \EndIf
    \If {$\mnode_\mnew \ne \varnothing$}
        \State \Call{Anchor}{$\mlink_\mnew, \mnode_\mnew$}
    \EndIf
    \State \Return $\mlink_\mnew$
\EndFunction
\end{algorithmic}
\end{algorithm}

%%%%%%%%%%%%%%%%%%%%%%%%%%%%%%%%% ALG: ERASETREE  %%%%%%%%%%%%%%%%%%%%%%%%%%%%%%%%%%%%%
\subsubsection{\textproc{EraseTree}: \textit{Deletes Dangling Links}}
The \textproc{EraseTree} function (Alg. \ref{suppalg:erasetree}) erases a link $\mlink$ is dangling and does not connect to links in the $(-\mtdir)$-direction. 
The removal of $\mlink$ can cause the $\mtdir$-direction links to dangle, which the function subsequently erases.
If any dangling link is pointing to a queued query, the query is removed from the open-list and deleted.
\begin{algorithm}[!ht]
\begin{algorithmic}[1]
\caption{\textproc{EraseTree}: erases a dangling branch of links.}
\label{suppalg:erasetree}
\Function{EraseTree}{$\mtdir$, $\mlink$} 
    \If{$\flinks(-\mtdir, \mlink) \ne \{\}$}
        \State \Return
    \ElsIf{$\fquery(\mlink) \ne \varnothing$}
        \State Unqueue $\fquery(\mlink)$ from open-list
    \EndIf
    \For {$\mlink_\mtdir \in \flinks(\mtdir, \mlink)$}
        \State \Call{Disconnect}{$\mtdir$, $\mlink$, $\mlink_\mtdir$}
        \Call{EraseTree}{$\mtdir$, $\mlink$}
    \EndFor
\EndFunction
\end{algorithmic}
\end{algorithm}

%%%%%%%%%%%%%%%%%%%%%%%%%%%% RAY %%%%%%%%%%%%%%%%%%%%%%%%%%%%%%%%%%%%%%%%%%%%%
\newpage
\subsection{Sector-ray}
A sector-ray has the following form
\begin{equation}
    \mray = (\mrtype, \mx_S, \mx_T, \mx_L, \mx_R),
\end{equation}
which records a cast from $\mx_S$ to $\mx_T$ and any collision information $\mx_L$ and $\mx_R$.
The ray type $\mrtype \in \{\mrvy, \mrvu, \mrvn\}$ indicates visibility between $\mx_S$ and $\mx_T$.
If $\mx_S$ and $\mx_T$ are visible to each other, $\mrtype = \mrvy$. If they are not visible to each other, $\mrtype= \mrvn$. If the ray is not yet cast and visibility is unknown, $\mrtype = \mrvu$.

When a ray collides with an obstacle's edge and $\mrtype=\mrvn$, $\mx_L$ and $\mx_R$ record the first corner encountered after tracing left and right from the collision point respectively.  
If the ray is $\mrvy$-typed, it can be \textbf{projected} in the direction $\mora{\mx_S,\mx_T}$ from $\mx_T$. 
The projected ray may collide and $\mx_L$ and $\mx_R$ records the collision of the projected ray. 
Note that, in \rtwop{}, projections always collide and never goes out of the map.

%%%%%%%%%%%%%%%%%%%%%%%%%%%%%%%%% ALG: FXCOL %%%%%%%%%%%%%%%%%%%%%%%%%%%%%%%%%%%%%
\subsubsection{\textproc{$\fxcol$}: \textit{Returns a Corner Beside the Collision Point}}
\textproc{$\fxcol$} (Alg. \ref{suppalg:fxcol}) returns first corner on the $\mside$-side ($\mside\in\{L,R\}$) of the collision point of a ray $\mray$. 
\begin{algorithm}[!ht]
\begin{algorithmic}[1]
\caption{$\fxcol$: gets the first corner on one side of a ray's collision point.}
\label{suppalg:fxcol}
\Function{$\fxcol$}{$\mside, \mray$}
    \State \Return $\mray\mdot\mx_L$ \textbf{if} $\mside = L$ \textbf{else} $\mray\mdot\mx_R$
\EndFunction
\end{algorithmic}
\end{algorithm}

%%%%%%%%%%%%%%%%%%%%%%%%%%%%%%%%% ALG: GETRAY  %%%%%%%%%%%%%%%%%%%%%%%%%%%%%%%%%%%%%
\subsubsection{\textproc{GetRay}: \textit{Retrieves or Constructs a Sector-ray}} 
The function \textproc{GetRay} (Alg. \ref{suppalg:getray}) finds a matching ray from $\mx_S$ to $\mx_T$ ifit exists and returns it.
If it does not exist, a new ray is created and returned.
\begin{algorithm}[!ht]
\begin{algorithmic}[1]
\caption{\textproc{GetRay}: gets or creates a ray.}
\label{suppalg:getray}
\Function{GetRay}{$\mx_S$, $\mx_T$}
    \State Try finding $\mray = (\cdots, \mx_S, \mx_T, \cdots)$.
    \If{ $\mray$ does not exist}
        \State Create $\mray = (\mrvu, \mx_S, \mx_T, \varnothing, \varnothing)$
    \EndIf
    \State \Return $\mray$
\EndFunction
\end{algorithmic}
\end{algorithm}

%%%%%%%%%%%%%%%%%%%%%%%%%%%%%%%% QUEUED QUERY %%%%%%%%%%%%%%%%%%%%%%%%%%%%%%%%%%%%%%%%%%%
\subsection{Queued Query and Open-list} \label{suppsec:queuedquery}
A query, when queued to the open-list, has the form
\begin{equation}
    \mquery = (\mqtype, f, \mlink_\mquery),
\end{equation}
where $\mqtype \in \{ \mqcast, \mqtrace \}$ is used to denote if the query is a casting or tracing query. 
$f$ is the sum of the minimum cost-to-go and cost-to-come of a link $\mlink_\mquery$, which is anchored on a leaf node \textproc{$\fnode$}($\mlink_\mquery$). 

% When a casting query is \textit{polled} from the open-list, line-of-sight is checked  between the two nodes indirectly connected by the link. When line-of-sight is checked, a ray is cast from the node that is in the source direction to the node that is in the target direction.

% When a tracing query is \textit{polled} from the open-list, a trace begins from $\fx(\mlink)$. The anchored node $\fnode(\mlink)$ is a source leaf node. Before the trace begins, $\mtrace$ is created. $\mlink$ is transferred to $\mtrace\mdot\mnode_S$ and its target links transferred to $\mtrace\mdot\mnode_T$.

The \textbf{open-list} is a priority queue that sorts queries based on a query's cost $f$,
which serves the same purpose as the A*'s open-list.
The default sorting algorithm of the open-list is insert-sort which is fast if the number of queries are small. The number of queries are small if the path is expected to have few turning points. 
A more efficient sorting algorithm may have higher overheads, but can improve solving times if the path is expected to have many turning points, especially in maps with highly non-convex obstacles or many disjoint obstacles.

%%%%%%%%%%%%%%%%%%%%%%%%%%%%%%%%% ALG: QUEUE  %%%%%%%%%%%%%%%%%%%%%%%%%%%%%%%%%%%%%
\subsubsection{\textproc{Queue}: \textit{Queues a Query into the Open-list}}
The function \textproc{Queue} (Alg. \ref{suppalg:queue}) creates a query $\mquery$, and
sorts it into the open-list based on its cost $\mquery\mdot f$.
\begin{algorithm}[!ht]
\begin{algorithmic}[1]
\caption{\textproc{Queue}: queues a new query to the open-list.}
\label{suppalg:queue}
\Function{Queue}{$\mqtype, f, \mlink_\mquery$}
    \State $\mquery \gets (\mqtype, f, \mlink_\mquery)$
    \State Insert $\mquery$ into open-list and sort $\mquery$ based on $\mquery\mdot f$
\EndFunction
\end{algorithmic}
\end{algorithm}

%%%%%%%%%%%%%%%%%%%%%%%%%%%%%%%%% ALG: UNQUEUE  %%%%%%%%%%%%%%%%%%%%%%%%%%%%%%%%%%%%%
\subsubsection{\textproc{Unqueue}: \textit{Removes a Queued Query from the Open-list}}
The function \textproc{Unqueue} (Alg. \ref{suppalg:unqueue}) removes a query $\mquery$ from the open-list.
\begin{algorithm}[!ht]
\begin{algorithmic}[1]
\caption{\textproc{Unqueue}: unqueues a query from the open-list.}
\label{suppalg:unqueue}
\Function{Unqueue}{$\mquery$}
    \State Remove $\mquery$ from the open-list
\EndFunction
\end{algorithmic}
\end{algorithm}

%%%%%%%%%%%%%%%%%%%%%%%%%%%%%%%%% ALG: POLL  %%%%%%%%%%%%%%%%%%%%%%%%%%%%%%%%%%%%%
\subsubsection{\textproc{Poll}: \textit{Removes Cheapest Query from the Open-list}}
The function \textproc{Poll} (Alg. \ref{suppalg:poll}) finds the cheapest queued query and returns it after removing it from the open-list.
\begin{algorithm}[!ht]
\begin{algorithmic}[1]
\caption{\textproc{Poll}: polls the cheapest query from the open-list.}
\label{suppalg:poll}
\Function{Poll}{\null}
    \State $\mquery \gets $ query that has smallest cost $\mquery\mdot f$ in open-list
    \State \Call{Unqueue}{$\mquery$}
    \State \Return $\mquery$
\EndFunction
\end{algorithmic}
\end{algorithm}

%%%%%%%%%%%%%%%%%%%%%%%%%%%%%%%% TRACING QUERY %%%%%%%%%%%%%%%%%%%%%%%%%%%%%%%%%%%%%%%%%%%
\subsection{Trace Object}
During a trace, any information or states related to the trace are captured in the Trace object
\begin{equation}
    \mtrace = ( \mxtrace, \msidetrace, \mtnode_S, \mtnode_T, \mnlets_S, \mnlets_T, \mnumcrns, \moverlap).
\end{equation}
$\mxtrace$ is the pair of coordinates for the corner being examined by the trace. $\msidetrace$ is the side of the trace. 
$\mtnode_S$ and $\mtnode_T$ are trace-nodes described in Sec. \ref{suppsec:tnodesandtlinks}.
$\mnlets_S$ and $\mnlets_T$ are ordered sets containing nodelets, described in Sec. \ref{suppsec:nodelets}.
$\mnumcrns$ is a counter for the number of corners traced, and $\moverlap$ is a Boolean flag indicating if the trace has found nodes that overlap with other queries.

%%%%%%%%%%%%%%%%%%%%%%%%%%%%%%%% ALG: FTNODE %%%%%%%%%%%%%%%%%%%%%%%%%%%%%%%%%%%%%%%%%%%
\newpage
\subsubsection{\textproc{$\ftnode$}: \textit{Gets a Trace-node from a Trace Object}}
\textproc{$\ftnode$} (Alg. \ref{suppalg:ftnode}) returns the $\mtdir$-direction ($\mtdir\in\{S,T\}$) trace-node $\mtnode_S$ or $\mtnode_T$ of a Trace object $\mtrace$.
\begin{algorithm}[!ht]
\begin{algorithmic}[1]
\caption{$\ftnode$: gets a trace-node from a Trace object.}
\label{suppalg:ftnode}
\Function{$\ftnode$}{$\mtdir, \mtrace$}
    \State \Return $\mtrace\mdot\mtnode_S$ \textbf{if} $\mtdir = S$ \textbf{else} $\mtrace\mdot\mtnode_T$
\EndFunction
\end{algorithmic}
\end{algorithm}

%%%%%%%%%%%%%%%%%%%%%%%%%%%%%%%% ALG: FNLETS %%%%%%%%%%%%%%%%%%%%%%%%%%%%%%%%%%%%%%%%%%%
\subsubsection{\textproc{$\fnlets$}: \textit{Gets a Set of Nodelets from a Trace Object}}
\textproc{$\fnlets$} (Alg. \ref{suppalg:fnlets}) returns the $\mtdir$-direction ($\mtdir\in\{S,T\}$) set of nodelets $\mnlets_S$ or $\mnlets_T$ of a Trace object $\mtrace$.
\begin{algorithm}[!ht]
\begin{algorithmic}[1]
\caption{$\fnlets$: gets a set of nodelets from a Trace object.}
\label{suppalg:fnlets}
\Function{$\fnlets$}{$\mtdir, \mtrace$}
    \State \Return $\mtrace\mdot\mnlets_S$ \textbf{if} $\mtdir = S$ \textbf{else} $\mtrace\mdot\mnlets_T$
\EndFunction
\end{algorithmic}
\end{algorithm}

%%%%%%%%%%%%%%%%%%%%%%%%%%%%%%%% ALG: FNLETS %%%%%%%%%%%%%%%%%%%%%%%%%%%%%%%%%%%%%%%%%%%
\subsubsection{\textproc{$\fnlet$}: \textit{Gets a Nodelet from a Trace Object}}
\textproc{$\fnlet$} (Alg. \ref{suppalg:fnlet}) returns the first nodelet from the $\mtdir$-direction ($\mtdir\in\{S,T\}$) set of nodelets $\mnlets_S$ or $\mnlets_T$. 
The nodelets belong to a Trace object $\mtrace$.
The function is useful since traces contain only one source nodelet at all times, and there may occasionally be only one target nodelet.
\begin{algorithm}[!ht]
\begin{algorithmic}[1]
\caption{$\fnlet$: gets the first source or target nodelet from a Trace object.}
\label{suppalg:fnlet}
\Function{$\fnlet$}{$\mtdir, \mtrace$}
    \State \Return $\mtrace\mdot\mnlets_S$[1] \textbf{if} $\mtdir = S$ \textbf{else} $\mtrace\mdot\mnlets_T$[1]
\EndFunction
\end{algorithmic}
\end{algorithm}

%%%%%%%%%%%%%%%%%%%%%%%%%%%%%%%%% ALG: CREATETRACE %%%%%%%%%%%%%%%%%%%%%%%%%%%%%%%%%%%%%
\subsubsection{\textproc{CreateTrace}: \textit{Creates a Trace Object}}
The function \textproc{CreateTrace} (Alg. \ref{suppalg:createtrace}) creates a new trace object and returns it.
\begin{algorithm}[!ht]
\begin{algorithmic}[1]
\caption{\textproc{CreateTrace}: creates a Trace object.}
\label{suppalg:createtrace}
\Function{CreateTrace}{$\mxtrace, \msidetrace$}
    \State $\mtrace \gets (\mxtrace, \msidetrace, \varnothing, \varnothing, \{\}, \{\}, 0, \mfalse)$
    \State $\mtrace \mdot \mnode_S \gets (\mntm, \msidetrace, S, \{\})$
    \State $\mtrace \mdot \mnode_T \gets (\mntm, \msidetrace, T, \{\})$
    \State \Return $\mtrace$
\EndFunction
\end{algorithmic}
\end{algorithm}

\subsection{Trace-nodes and Trace-links} \label{suppsec:tnodesandtlinks}
Trace objects contain temporary nodes (\textbf{trace-nodes}) $\mtnode_S$ and $\mtnode_T$, which follow the trace and are always located at $\mxtrace$, such that $\fx(\mtnode_S) = \fx(\mtnode_T) = \mxtrace$.
The trace-nodes are not part of the source-tree or target-tree. The trace-nodes anchor temporary links called \textbf{trace-links}. 
The parent node of a trace-link is located on the source-tree or target-tree if the trace-link is anchored at $\mtnode_S$ or $\mtnode_T$ respectively.
At the start of the trace, trace-links may have been re-anchored to the trace-nodes from nodes in the trees, or may have been duplicated from existing links.

Trace-links do not have child links, and are intentionally left \textbf{dangling} (not connected to any source link and/or target link) to facilitate pruning and placement.
When a trace stops, trace-links are re-anchored to the source-tree or target-tree nodes, and re-connected to other links if they are not discarded.
If the trace-links are discarded, they would be1 left dangling.

\subsection{Nodelets} \label{suppsec:nodelets}
Trace objects contain \textbf{nodelets} in ordered sets $\mnlets_S$ and $\mnlets_T$.
A nodelet describes a trace-link and its associated progression ray and winding counter:
\begin{equation}
\mnlet = ( \mtlink, \mvprog, \mcprog).
\end{equation}
where $\mtlink$ is a trace-link anchored on a trace-node. 
$\mvprog$ is the progression ray with respect to the parent node. $\mcprog \ge 0$ is the winding counter for the progression ray.

During a trace, the nodelets are examined in sequence, and may be removed or added.
At any one time during the trace, only \textit{one} source nodelet is examined, while at least one target nodelet is examined. 
The trace ends when there are no source or target nodelets left.

%%%%%%%%%%%%%%%%%%%%%%%%%%%%%%%%% ALG: CREATENODELET  %%%%%%%%%%%%%%%%%%%%%%%%%%%%%%%%%%%%%
\subsubsection{\textproc{CreateNodelet}: \textit{Creates a Nodelet}}
The function \textproc{CreateNodelet} (Alg. \ref{suppalg:createnodelet}) creates a new nodelet object, pushes it to the front or back ($pos = \{\mfront, \mback\}$) of $\mnlets$ and returns the nodelet object.
\begin{algorithm}[!ht]
\begin{algorithmic}[1]
\caption{\textproc{CreateNodelet}: creates a new nodelet.}
\label{suppalg:createnodelet}
\Function{CreateNodelet}{$\mtlink, \mvprog, pos, \mnlets$}
    \State $\mnlet \gets (\mtlink, \mvprog, 0)$
    \State Push $\mnlet$ to $pos$ of $\mnlets$
        \Comment{$pos \in \{\mfront, \mback\}$}
    \State \Return $\mnlet$
\EndFunction
\end{algorithmic}
\end{algorithm}

%%%%%%%%%%%%%%%%%%%%%%%%%%%%%%%%% OVERLAP-BUFFER  %%%%%%%%%%%%%%%%%%%%%%%%%%%%%%%%%%%%%
\subsection{Overlap-buffer}
The \textbf{overlap-buffer} is an unordered set containing Position objects. Each position object contains source-tree $\mnvu$ and/or $\mneu$ nodes. The nodes anchor links which are part of queries that overlap. 

During an iteration between two polls from the open-list, a few traces may occur.
The overlap-buffer is filled during the traces, if overlaps are identified.
The overlap-buffer is subsequently emptied and the links processed by the overlap rule after all traces in the iteration have stopped. 
% The source-tree $\mnvu$ and $\mneu$ nodes are identified at the position, and the overlap rule searches the links anchored on the nodes.
% Queries in the target-direction of the links are identified and removed from the open-list.
% The first source-tree $\mney$ or $\mnvy$ node in the source-direction of the links are subsequently identified.

%%%%%%%%%%%%%%%%%%%%%%%%%%%%%%%%% ALG: PUSHOVERLAP  %%%%%%%%%%%%%%%%%%%%%%%%%%%%%%%%%%%%%
\subsubsection{\textproc{PushOverlap}: \textit{Push a Position Object into Overlap-buffer}}
The function \textproc{PushOverlap} (Alg. \ref{suppalg:pushoverlap}) pushes a Position object $\mpos$ into the overlap-buffer. The overlap-buffer is a set of $\mpos$, and is filled at the end of a trace when overlapping paths are identified during the trace.
The reader may choose to avoid adding duplicate $\mpos$ into the overlap-buffer.

\begin{algorithm}[!ht]
\begin{algorithmic}[1]
\caption{\textproc{PushOverlap}: pushes a Position object into the overlap-buffer.}
\label{suppalg:pushoverlap}
\Function{PushOverlap}{$\mpos$}
    \State Insert $\mpos$ to overlap-buffer (an unordered set of $\mpos$).
\EndFunction
\end{algorithmic}
\end{algorithm}

%%%%%%%%%%%%%%%%%%%%%%%%%%%%%%%%% OCCUPANCY GRID %%%%%%%%%%%%%%%%%%%%%%%%%%%%%%%%%%%%%
\subsection{Occupancy Grid}
The current implementation of \rtwop{} operates on a binary occupancy grid.
Each cell is either occupied or free, and \rtwop{} finds an any-angle path on vertices, which are the corners of the cells.
The occupancy grid is implemented as a Boolean array. 
Hash tables or equivalent containers consume less memory but are slower to access for two-dimensional occupancy grids.

%%%%%%%%%%%%%%%%%%%%%%%%%%%%%%%%% ALG: BISECTOCSEC  %%%%%%%%%%%%%%%%%%%%%%%%%%%%%%%%%%%%%
\subsubsection{\textproc{Bisect}: \textit{Gets Bisecting Directional Vector of a Corner}} 
The \textproc{Bisect} function (Alg. \ref{suppalg:bisect}) returns the directional vector that bisects the occupied-sector of a corner at $\mx$. 
For an occupancy grid, the bisecting vector points in the ordinal (northeast, northwest, etc.) directions.

\begin{algorithm}[!ht]
\begin{algorithmic}[1]
\caption{\textproc{Bisect}: gets bisecting directional vector of a corner.}
\label{suppalg:bisect}
\Function{Bisect}{$\mx$} 
    \State \Return vector parallel to a directional vector that points into and bisects the occupied-sector at the corner at $\mx$.
\EndFunction
\end{algorithmic}
\end{algorithm}

%%%%%%%%%%%%%%%%%%%%%%%%%%%%%%%%% ALG: GETEDGE  %%%%%%%%%%%%%%%%%%%%%%%%%%%%%%%%%%%%%
\subsubsection{\textproc{GetEdge}: \textit{Gets Directional Vector of an Obstacle's Edge}} 
The \textproc{GetEdge} function (Alg. \ref{suppalg:getedge}) returns the directional vector of an edge on the $\mside$-side of a corner at $\mx$. 
The directional vector should be \textit{parallel} to $\mx_\mside$ - $\mx$, where $\mx_\mside$ is the corner at the other end of the $\mside$-side edge.

\begin{algorithm}[!ht]
\begin{algorithmic}[1]
\caption{\textproc{GetEdge}: gets the directional vector of a corner's adjacent edge.}
\label{suppalg:getedge}
\Function{GetEdge}{$\mx$, $\mside$} 
    \State \Return vector parallel to $\mside$-side edge adjacent to corner at $\mx$. \Comment{Vector points from $\mx$ to corner on the $\mside$-side.}
\EndFunction
\end{algorithmic}
\end{algorithm}

%%%%%%%%%%%%%%%%%%%%%%%%%%%%%%%%% ALG: TRACE %%%%%%%%%%%%%%%%%%%%%%%%%%%%%%%%%%%%%
\subsubsection{\textproc{Trace}: \textit{Traces to a Corner}} 
The function \textproc{Trace} (Alg. \ref{suppalg:trace} traces to any corner from a position $\mx$ along the $\mside$-side edge of $\mx$. 
$\mx$ must be located on an obstacle's edge.
Corners encountered by the algorithm should be cached as a graph of connected corners, to allow repeatedly traced corners to be identified in constant time by the function.

The intersection of an obstacle edge with the map boundary is considered a corner.
A trace that continues from the boundary corner will cause the function to return $\varnothing$ as the trace has gone out of map.
\begin{algorithm}[!ht]
\begin{algorithmic}[1]
\caption{\textproc{Trace}: traces to a corner.}
\label{suppalg:trace}
\Function{Trace}{$\mx$, $\mside_d$}
    \State $\mx_\mnext \gets$ which is position of the first corner at the $\mside$-side of $\mx$
    \State \Return $\mx_\mnext$ if in map, or $\varnothing$ if out of map.
\EndFunction
\end{algorithmic}
\end{algorithm}

%%%%%%%%%%%%%%%%%%%%%%%%%%%%%%%%% ALG: LOS  %%%%%%%%%%%%%%%%%%%%%%%%%%%%%%%%%%%%%
\subsubsection{\textproc{LOS}: \textit{Collision Line Algorithm}}
The function \textproc{LOS} (Alg. \ref{suppalg:los}) casts or projects a ray using a line algorithm that can detect collisions.
If the occupancy grid is used, the Bresenham line algorithm can be implemented but should be modified to allow all cells intersected by the ray to be identified.
If a collision occurs, the function finds the first left or right corner from the collision point.

In \rtwop{}, a projected ray can never go out of a rectangular map, or a map with a convex shape. 
For completeness, the reader may choose to implement an out-of-map check when a projection occurs.

\rtwop{} depends on $\mx_L$ and $\mx_R$ to check if a trace has crossed a collision point of a sector-ray. Careful positioning of $\mx_L$ and $\mx_R$ is required to break ties in discrete, special cases. 
The cases can include a trace being parallel to a sector ray, or the start node lying on a corner or an edge, etc.
\begin{algorithm}[!ht]
\begin{algorithmic}[1]
\caption{\textproc{LOS}: ray tracer and collision finder.}
\label{suppalg:los}
\Function{LOS}{$cast, \mray = (\mrtype, \mx_S, \mx_T, \mx_L, \mx_R)$}
    \State $\mv_\mathrm{ray} \gets \mx_T - \mx_S$
    \If {$cast = \mtrue$}
        \State Do line algorithm in direction $\mv_\mathrm{ray}$ from $\mx_S$ until collision or $\mx_T$ is reached.
    \Else
    \Comment{Project}
        \State Do line algorithm in direction $\mv_\mathrm{ray}$ from $\mx_T$ until collision. 
    \EndIf
    \If {a collision occurs at some $\mx_\mathrm{col}$}
        \State $\mray\mdot\mrtype \gets \mrvn$
        \If {$\mx_\mathrm{col}$ is at a corner}
            \State $\mray\mdot\mx_L \gets \mx_\mcol$
            \State $\mray\mdot\mx_R \gets \mx_\mcol$
            \State $\mv_\mathrm{crn} \gets $ \Call{Bisect}{$\mx_\mcol$}
            \State $u = \mv_\mathrm{crn} \times \mv_\mathrm{ray}$
            \If {$u < 0$}
            \Comment{Ray points to right of $\mv_\mathrm{crn}$}
                \State $\mray\mdot\mx_R \gets$ \Call{Trace}{$\mx_\mathrm{col}$, $R$}
            \ElsIf {$u > 0$}
                \Comment{Ray points to left of $\mv_\mathrm{crn}$}
                \State $\mray\mdot\mx_L \gets$ \Call{Trace}{$\mx_\mathrm{col}$, $L$}
            \EndIf
        \Else 
        \Comment{$\mx_\mathrm{col}$ is on an edge}
            \State $\mray\mdot\mx_L \gets $ \Call{Trace}{$\mx_\mathrm{col}, L$}
            \State $\mray\mdot\mx_R \gets $ \Call{Trace}{$\mx_\mathrm{col}, R$}
        \EndIf
    \Else \Comment{No collision, occurs only when $cast = \mtrue$}
        \State $\mray\mdot\mrtype \gets \mrvy$ 
    \EndIf
\EndFunction
\end{algorithmic}
\end{algorithm}

%%%%%%%%%%%%%%%%%%%%%%%%%%%%%%%%% ALG: CAST  %%%%%%%%%%%%%%%%%%%%%%%%%%%%%%%%%%%%%
\subsubsection{\textproc{Cast}: \textit{Casts a Ray}}
The function \textproc{Cast} (Alg. \ref{suppalg:cast}) wraps the function \textproc{LOS}, and returns immediately if the ray has been cast. 
\vspace{-0.3cm}
\begin{algorithm}[!ht]
\begin{algorithmic}[1]
\caption{\textproc{Cast}: casts a ray.}
\label{suppalg:cast}
\Function{Cast}{$\mray = (\mrtype, \mx_S, \mx_T, \mx_L, \mx_R)$}
    \IfThen {$\mrtype = \mrvu$} { \Call{LOS}{$\mtrue, \mray$} }
\EndFunction
\end{algorithmic}
\end{algorithm}

%%%%%%%%%%%%%%%%%%%%%%%%%%%%%%%%% ALG: PROJECT  %%%%%%%%%%%%%%%%%%%%%%%%%%%%%%%%%%%%%
\subsubsection{\textproc{Project}: \textit{Projects a Ray}}
The function \textproc{Project} (Alg. \ref{suppalg:project}) wraps the function \textproc{LOS}, and returns immediately if the ray has been cast.
\vspace{-0.3cm}
\begin{algorithm}[!ht]
\begin{algorithmic}[1]
\caption{\textproc{Project}: projects a ray.}
\label{suppalg:project}
\Function{Project}{$\mray = (\mrtype, \mx_S, \mx_T, \mx_L, \mx_R)$}
    \IfThen {$\mx_L = \varnothing$}{ \Call{LOS}{$\mfalse, \mray$}}
\EndFunction
\end{algorithmic}
\end{algorithm}

\clearpage
%%%%%%%%%%%%%%%%%%%%%%%%%%%%%%%%% ALG: RUN  %%%%%%%%%%%%%%%%%%%%%%%%%%%%%%%%%%%%%
\section{Initializing \rtwop{}}
\setcounter{algorithm}{0}

This section details the \rtwop{} algorithm, and is constructed from the objects and methods listed in the prior sections.

\subsection{\textproc{Run}: main function of \rtwop{}.}
\begin{algorithm}[!ht]
\begin{algorithmic}[1]
\caption{\textproc{Run}: main \rtwop{} algorithm.}
\label{suppalg:run}
\Function{Run}{$\mxstart, \mxgoal$}
    \State $path \gets \{\}$
    \Comment{open-list, overlap-buffer, $path$, $\mxstart$ and $\mxgoal$ are accessible to all functions in R2*.}
    \If {\Call{InitialCaster}{\null} $ = \mfalse$} 
        \Comment{No direct path found.}
        \While{open-list is not empty}
            \State $\mquery \gets $ \Call{Poll}{\null}
            \If {$\mquery\mdot\mqtype = \mqtrace$}
                \State \Call{TracerFromLink}{$\mquery\mdot\mlink$}
            \ElsIf {\Call{Caster}{$\mquery\mdot\mlink$}}
                \State \Break \Comment{Path found.}
            \EndIf
            \If {overlap-buffer is not empty}
                \State \Call{ShrinkSourceTree}{\null} \Comment{Overlap rule for traces that overlap in this iteration.}
            \EndIf
        \EndWhile
    \EndIf

    \State \Return $path$

\EndFunction
\end{algorithmic}
\end{algorithm}

\subsection{Initial Casting and Tracing}
This section details initial functions used to initialize \rtwop{} and bring the algorithm into the main iteration between open-list polls.

%%%%%%%%%%%%%%%%%%%%%%%%%%%%%%%%% ALG: INITIALCASTER  %%%%%%%%%%%%%%%%%%%%%%%%%%%%%%%%%%%%%
\subsection{\textproc{InitialCaster}: \textit{First Cast}} \label{suppsec:initialcaster}
The first caster function \textproc{InitialCaster} (Alg. \ref{suppalg:initialcaster}) is a special casting-query function between the start and goal points. The function is used only once.

If there is line-of-sight between the start and goal points, \rtwop{} returns immediately with the path.
If the ray from the start to goal collides, \rtwop{} begins initialization, and two traces and a reversed ray are generated.

The reversed ray begins at the goal point and ends at the start point, which is opposite to the direction of the cast.
The reversed ray ensures that calculations with a start node's angular-sector are correct, primarily by dividing the start node into two nodes, each with a $180^\circ$ angular-sector.
The $180^\circ$ sectors are bounded by the forward ray (start to goal) and the reversed ray (goal to start), and ensures that all calculations with the cross-product are correct.

The goal node is initialized before being passed to the tracing queries.
\begin{algorithm}[!ht]
\begin{algorithmic}[1]
\caption{\textproc{InitialCaster}: initial casting query.}
\label{suppalg:initialcaster}
\Function{InitialCaster}{\null}
    \State $\mray \gets $ \Call{GetRay}{$\mxstart, \mxgoal$}
    \State \Call{Cast}{$\mray$}
    \If {$\mray\mdot\mrtype = \mrvy$}
        \Comment{Start and goal points have line-of-sight}
        \State $path \gets \{ \mxgoal, \mxstart \}$
        \State \Return $\mtrue$
    \EndIf
    
    \Comment{Cast collided, create nodes and begin tracing queries}
    \State $\mray_\mathrm{rev} \gets $ \Call{GetRay}{$\mxgoal, \mxstart$}
    \Comment{A special, reversed ray to ensure that the ang-sec. for start nodes are convex.}
    \State $\mnode_{T} \gets $ \Call{GetNode}{$\mxgoal, \mnvy, L, T$} 
    \Comment{Goal node can have any side.}

    \State \Call{InitialTrace}{$L, \mray, \mray_\mathrm{rev}, \mnode_T$}
    \State \Call{InitialTrace}{$R, \mray, \mray_\mathrm{rev}, \mnode_T$}

    \State \Return $\mfalse$
\EndFunction
\end{algorithmic}
\end{algorithm}

%%%%%%%%%%%%%%%%%%%%%%%%%%%%%%%%% ALG: INITIALTRACER  %%%%%%%%%%%%%%%%%%%%%%%%%%%%%%%%%%%%%
\subsection{\textproc{InitialTrace}: \textit{First Trace}}
When a cast from the start point to the goal point collides, the \textproc{InitialTrace} function (Alg. \ref{suppalg:initialcaster}) initializes links and two start nodes.
After initialization, a trace begins from one-side of the collision point. 
The function is used only twice, each for one side of the collision.

Two start nodes $\mnode_S$ and $\mnode_{SS}$ with sides $\msidetrace$ are created by the function, each with a $180^\circ$ angular-sector. 
For brevity, a \textit{start node} in the text refers to any one of the two, unless a distinction needs to be made.
Zero-length links $\mlink_S$ and $\mlink_{SS}$ are anchored at $\mnode_S$ and $\mnode_{SS}$ respectively. 
$\mlink_{SS}$ is the source link of $\mlink_S$, and $\mlink_S$ is the source link of the trace-link $\mtlink_S$ which is anchored on the source trace-node.
$\mtlink_S$ and $\mlink_S$ stores the $180^\circ$ angular-sectors of $\mnode_S$ and $\mnode_{SS}$ respectively.
When viewed from the start point, the angular-sector of $\mnode_S$ is the \textit{first} $180^\circ$ angular sector, which rotates in the $\mside$-direction from the forward ray to the reverse ray.
The angular-sector of $\mnode_{SS}$ is the \textit{second} $180^\circ$ angular sector, which rotates from the reverse ray to the forward ray.

% Fig. \ref{suppfig:initialtracer} illustrates the sectors and nodes.

The goal link is initialized in the tracing query instead of in \textproc{InitialCaster} like the goal node.
If the goal link is initialized in \textproc{InitialCaster}, it may be deleted by the first call to \textproc{InitialTracer} and before the second call is made, as the first trace can go out-of-map.

Note that as more collisions occur, more links will be connected to the goal link, and the set of source link pointers $\mlinks_S$ in the goal link can become anomalously large, particularly in maps with highly non-convex obstacles or many disjoint obstacles.
For example, while the majority of links may have connections numbering less than ten, the goal link may have over a few thousand connections.
The reader may choose to use a container with constant time insertion or deletion (note that $\mlinks_S$ is unordered), but as the number of links are usually very small, a contiguous data structure with linear time insertion or deletion may be more efficient.
If \rtwop{} is expected to perform on maps with highly non-convex obstacles or with many disjoint obstacles, a container with constant time insertion and deletion is recommended. 
Otherwise, a simple, contiguous data structure like an array will suffice, which is the default implementation of \rtwop{}.

\begin{algorithm}[!ht]
\begin{algorithmic}[1]
\caption{\textproc{InitialTrace}: initial tracing query.}
\label{suppalg:initialtrace}
\Function{InitialTrace}{$\msidetrace, \mray, \mray_\mathrm{rev}, \mnode_T$}
    \State $\mtrace \gets $ \Call{CreateTrace}{$\fxcol(\msidetrace, \mray), \msidetrace$}

    \Comment{Create source trace-link}
    \State $\mtlink_S \gets $ \Call{CreateLink}{$\mtrace\mdot\mtnode_S$}
    \State $\fray(\msidetrace, \mtlink_S) \gets \mray_\mathrm{rev}$
    \State $\fray(-\msidetrace, \mtlink_S) \gets \mray$
    \State $\mvray \gets \mray\mdot\mx_T - \mray\mdot\mx_S$

    \Comment{Create $\msidetrace$-side start node and link for first $180^\circ$ ang-sec.}
    \State $\mnode_S \gets $ \Call{GetNode}{$\mxstart, \mnvy, \msidetrace, S$}
    \State $\mlink_S \gets $ \Call{CreateLink}{$\mnode_S$}
    \State $\fray(\msidetrace, \mlink_S) \gets \mray$
    \State $\fray(-\msidetrace, \mlink_S) \gets \mray_\mathrm{rev}$
    \State $\mlink_S\mdot\mcost \gets 0$
    \State \Call{Connect}{$T, \mlink_S, \mtlink_S$}

    \Comment{Create link for second $180^\circ$ ang-sec of start node.}
    \State $\mlink_{SS} \gets $ \Call{CreateLink}{$\mnode_S$}
    \State $\mlink_{SS}\mdot\mcost \gets 0$
    \State \Call{Connect}{$T, \mlink_{SS}, \mlink_S$}

    \Comment{Create a link anchored at goal node and a target trace-link}
    \State $\mtlink_T \gets $ \Call{CreateLink}{$\mtrace\mdot\mtnode_T$}
    \State $\mlink_T \gets $ \Call{CreateLink}{$\mtnode_T$}
    \State $\mlink_T\mdot\mcost \gets 0$
    \State \Call{Connect}{$T, \mtlink_T, \mlink_T$}

    \State \Call{CreateNodelet}{$\mtlink_S, \mvray, \mback, \mtrace\mdot\mnlets_S$}
    \State \Call{CreateNodelet}{$\mtlink_T, -\mvray, \mback, \mtrace\mdot\mnlets_T$}
    \State \Call{Tracer}{$\mtrace$}

    \EndFunction
\end{algorithmic}
\end{algorithm}

\clearpage
\section{\textproc{Caster}: \textit{Handles a Casting Query}}
\setcounter{algorithm}{0}

The \textproc{Caster} function (Alg. \ref{suppalg:caster}) implements a casting query for a link $\mlink$.
A ray is cast from the source node of the link to the target node of the link.
The link can be anchored on either node, and is connected to one source link and at least one target link.
%%%%%%%%%%%%%%%%%%%%%%%%%%%%%%%%% ALG: CASTER  %%%%%%%%%%%%%%%%%%%%%%%%%%%%%%%%%%%%%
\begin{algorithm}[!ht]
\begin{algorithmic}[1]
\caption{\textproc{Caster}: handles a casting query.}
\label{suppalg:caster}
\Function{Caster}{$\mlink$}
    \State $\mnode_S \gets \fnode(\flink(S, \mlink))$
    \State $\mnode_T \gets \fnode(\flink(T, \mlink))$

    \State $\mray \gets $ \Call{GetRay}{$\fx(\mnode_S), \fx(\mnode_T)$}
    \State \Call{Cast}{$\mray$}

    \If {$\mray\mdot\mrtype = \mrvy$}
        \State \Return \Call{CastReached}{$\mray, \mlink$}
    \Else
        \State \Call{CastCollided}{$\mray, \mlink$}
        \State \Return $\mfalse$
    \EndIf
\EndFunction
\end{algorithmic}
\end{algorithm}

%%%%%%%%%%%%%%%%%%%%%%%%%%%%%%%%% ALG: CASTREACHED  %%%%%%%%%%%%%%%%%%%%%%%%%%%%%%%%%%%%%
\subsection{\textproc{CastReached}: \textit{Line-of-sight between Nodes of Cast}} 
The function \textproc{CastReached} (Alg. \ref{suppalg:castreached}) handles the case where a cast ray has line-of-sight.

In general, five cases occur when a cast reaches the target node from the source node.
\begin{enumerate}
    \item The shortest path is found when both nodes have cumulative visibility. This case is handled by the function \textproc{PathFound} (Alg. \ref{suppalg:pathfound}).
    \item The target node is an unreachable, $\mnun$-node. The caster query is discarded.
    \item The target node is a $\mntm$-node that is generated by an interrupted trace. The node may or may not be a valid turning point, and this case is handled by the function \textproc{ReachedTm} (Alg. \ref{suppalg:reachedtm}).
    \item Both nodes have unknown cumulative visibility. A new casting query for each target link of the link $\mlink$ is queued unless there are overlapping queries. This case is handled by the function \textproc{NoCumulativeVisibility} (Alg. \ref{suppalg:nocumulativevisibility}).
    \item Only the source node or target node has cumulative visibility. 
    If the source or target node has cumulative visibility, \rtwop{} proceeds to queue casting queries for the target links or source link respectively. This case is handled by the function \textproc{SingleCumulativeVisibility} (Alg. \ref{suppalg:singlecumulativevisibility}).
\end{enumerate}

% Fig. \ref{suppfig:castreached}.
\begin{algorithm}[!ht]
\begin{algorithmic}[1]
\caption{\textproc{CastReached}: cast has reached and ray has line-of-sight.}
\label{suppalg:castreached}
\Function{CastReached}{$\mray, \mlink$}
    \State $\mnode_S \gets \fnode(\flink(S, \mlink))$
    \State $\mnode_T \gets \fnode(\flink(T, \mlink))$
    
    \If{$\mnode_S\mdot\mntype = \mnvy $ \Or $\mnode_T\mdot\mntype = \mnvy$} 
        \Comment{Shortest path found.}
        \State \Call{PathFound}{$\mlink$}
        \State \Return $\mtrue$
    \ElsIf {$\mnode_T\mdot\mntype = \mnun$}
        \Comment{Discard if target node has type $\mnun$}
        \State \Call{DiscardReachedCast}{$\mlink$}   
    \ElsIf{$\mnode_T\mdot\mntype = \mntm$ }
        \Comment{Reached an interrupted trace.}
        \State \Call{ReachedTm}{$\mray, \mlink$}
    \ElsIf{$\mnode_S\mdot\mntype \notin \{\mnvy, \mney\}$ \An $\mnode_T\mdot\mntype \notin \{ \mnvy, \mney \}$}
        \Comment{$\mtrue$ if $\mnvu$ source node reached $\mnvu$ or $\mnoc$ target-tree node.}
        \State $(\mtdir_\mnext, \sim) \gets$ \Call{NoCumulativeVisibility}{$\mlink$}
        \State \Call{QueueReachedCast}{$\mtdir_\mnext, \mlink$}
    \Else
        \Comment{Either source or target node has cumulative visibility.}
        \State $(\mtdir_\mnext, \mnode_\mnext) \gets$ \Call{SingleCumulativeVisbility}{$\mray, \mlink$}
        \If {$\mnode_\mnext \ne \varnothing$}
            \State \Call{QueueReachedCast}{$\mtdir_\mnext, \mlink$}
        \EndIf
    \EndIf
    \State \Return $\mfalse$
\EndFunction
\end{algorithmic}
\end{algorithm}

%%%%%%%%%%%%%%%%%%%%%%%%%%%%%%%%% ALG: REACHEDTM  %%%%%%%%%%%%%%%%%%%%%%%%%%%%%%%%%%%%%
\newpage
\subsubsection{\textproc{ReachedTm}: \textit{Cast Reached for Target $\mntm$-node}}
The helper function \textproc{ReachedTm} handles cases when a cast reached a $\mntm$-node.
A $\mntm$-node is generated by an interrupted trace, which occurs when a number of corners is traced (Alg. \ref{suppalg:interrupt}), a recursive occupied-sector trace is called from the source node (Alg. \ref{suppalg:ocsecrule}), or a recursive angular-sector trace is called (Alg. \ref{suppalg:recurangsectrace}).
The $\mntm$-node has the same side as the interrupted trace that generated it.

As the $\mntm$-node can lie on any corner, \rtwop{} first checks if a turning point can be placed at the corner where the $\mntm$-node lies.
If a turning point cannot be placed at the corner, a trace resumes from the corner using the function \textproc{TracerFromLink} (Alg. \ref{suppalg:tracerfromlink}). 

If a turning point can be placed, the query proceeds by treating the target $\mntm$-node as a turning point.
If the source node has no cumulative visibility, 
the function \textproc{NoCumulativeVisibility} (Alg. \ref{suppalg:nocumulativevisibility}) is called.
If the source node has cumulative visibility, 
the function \textproc{SingleCumulativeVisibility} (Alg. \ref{suppalg:singlecumulativevisibility}) is called.

Even if a turning point can be placed, the target links of $\mlink$ may point into the occupied-sector of the target $\mntm$-node and are not castable.
A trace is generated for all non-castable links in \textproc{TraceFromTm} (Alg. \ref{suppalg:tracefromtm}), while a casting query is queued for each castable link in \textproc{CastFromTm} (Alg. \ref{suppalg:castfromtm}).

% Fig. \ref{suppfig:reachedtm}.

\begin{algorithm}[!ht]
\begin{algorithmic}[1]
\caption{\textproc{ReachedTm}: cast has reached a $\mntm$ node.}
\label{suppalg:reachedtm}
\Function{ReachedTm}{$\mray, \mlink$}
    \State $\mlink_S \gets \flink(S, \mlink)$
    \State $\mnode_S \gets \fnode(\flink(S, \mlink))$
    \State $\mnode_T \gets \fnode(\flink(T, \mlink))$
    \State $\mvray \gets \mray\mdot\mv_T - \mray\mdot\mv_S$
    \State $\mxtrace \gets \fx(\mnode_T)$
    \State $\msidetrace \gets \mnode_T\mdot\msidenode$
    \State $\mvnext \gets $ \Call{GetEdge}{$\msidetrace, \fx(\mnode_T)$}

    \Comment{Trace immediately if no turning point can be placed at $\mntm$ node.}
    \If {corner at $\mxtrace$ is non-convex \Or \Call{IsRev}{$\msidetrace, \mvray, \mvnext$} = $\mfalse$}
        \State \Call{TracerFromLink}{$\mlink$}
        \State \Return
    \EndIf

    \Comment{Try placing a turning point at $\mntm$ node.}
    \State $\mnode_\mnext \gets \varnothing$
    \If {$\mnode_S \notin \{\mnvy, \mney\}$}
        \State $(\sim, \mnode_\mnext) \gets $ \Call{NoCumulativeVisibility}{$\mlink$}
    \Else
        \State $(\sim, \mnode_\mnext) \gets $ \Call{SingleCumulativeVisibility}{$\mlink$}
        \If {$\mnode_\mnext = \varnothing$}  
            \State \Return
        \EndIf
    \EndIf

    \Comment{Queue castable links from new turning point.}
    \State $\hat{\mlinks}_\mathrm{newT} \gets $ \Call{CastFromTm}{$\mlink,  \mxtrace, \msidetrace, \mvnext$}
    
    \Comment{Continue tracing for non-castable links at new turning point.}
    \If {$\hat{\mlinks}_\mathrm{newT} \ne \{\}$}
        \State \Call{TraceFromTm}{$\mlink,  \mxtrace, \msidetrace, \mvnext, \hat{\mlinks}_\mathrm{newT}$}
    \EndIf
\EndFunction
\end{algorithmic}
\end{algorithm}

%%%%%%%%%%%%%%%%%%%%%%%%%%%%%%%% ALG: CASTROMTM %%%%%%%%%%%%%%%%%%%%%%%%%%%%%%%%%
\newpage
\subsubsection{\textproc{CastFromTm}: \textit{Try Casting From a Reached $\mntm$-node}}
The helper function \textproc{CastFromTm} (Alg. \ref{suppalg:castfromtm}) identifies castable target links of $\mlink$ and queues a casting query for each castable link.
Links that are not castable are pushed into an unordered set of links $\hat{\mlinks}_\mathrm{newT}$ and returned.
\begin{algorithm}[!ht]
\begin{algorithmic}[1]
\caption{\textproc{CastFromTm}: try casting from a new turning point at a reached $\mntm$ node.}
\label{suppalg:castfromtm}
\Function{CastFromTm}{$\mlink, \mxtrace, \msidetrace, \mvnext$}
    \State $\hat{\mlinks}_\mathrm{newT} \gets \{\}$
    \For {$\mlink_T \in \mlink\mdot\mlinks_T$}
        \State $\mnodepar \gets \fnode(\flink(T, \mlink_T))$
        \State $\mvpar \gets \mxtrace - \fx(\mnodepar)$
        % \If {$\mnodepar\mdot\mntype = \mnph$ \Or \Call{IsVis}{$\msidetrace, \mvpar, \mvnext$}$ = \mfalse$}
        %     \State Push $\mlink_T$ to back of $\hat{\mlinks}_\mathrm{newT}$
        %     \Comment{Trace from target node if next node is phantom point or not castable.}
        % \Else
        %     \Comment{Next node is castable and not phantom point.}
        %     \State $\mnode_\mnew \gets $ \Call{GetNode}{$\mxtrace, \mnvu, \msidetrace, T$}
        %     \State \Call{Anchor}{$\mlink_T, \mnode_\mnew$}
        %     \State \Call{Queue}{$\mqcast, \mlink\mdot\mcost + \mlink_T\mdot\mcost, \mlink_T$}
        % \EndIf
        \If {\Call{IsVis}{$\msidetrace, \mvpar, \mvnext$}}
            \Comment{Next node is castable and not phantom point.}
            \State $\mnode_\mnew \gets $ \Call{GetNode}{$\mxtrace, \mnvu, \msidetrace, T$}
            \State \Call{Anchor}{$\mlink_T, \mnode_\mnew$}
            \State \Call{Queue}{$\mqcast, \mlink\mdot\mcost + \mlink_T\mdot\mcost, \mlink_T$}
        \EndIf
    \EndFor
    \State \Return $\hat{\mlinks}_\mathrm{newT}$
\EndFunction
\end{algorithmic}
\end{algorithm}

%%%%%%%%%%%%%%%%%%%%%%%%%%%%%%%% ALG: TRACEFROMTM %%%%%%%%%%%%%%%%%%%%%%%%%%%%%%%%%
\newpage
\subsubsection{\textproc{TraceFromTm}: \textit{Try Tracing From a Reached $\mntm$-node}}
The helper function \textproc{TraceFromTm} (Alg. \ref{suppalg:tracefromtm}) generates a trace for all non-castable target links anchored on the target $\mntm$-node of a reached cast.
The links are contained in an unordered set $\hat{\mlinks}_\mathrm{newT}$, and are found by the function \textproc{CastFromTm} (Alg. \ref{suppalg:castfromtm}).
\begin{algorithm}[!ht]
\begin{algorithmic}[1]
\caption{\textproc{TraceFromTm}: try tracing from a new turning point at a reached $\mntm$ node.}
\label{suppalg:tracefromtm}
\Function{TraceFromTm}{$\mlink, \mxtrace, \msidetrace, \mvnext, \hat{\mlinks}_\mathrm{newT}$}
    \State $\mtrace \gets $ \Call{CreateTrace}{$\mxtrace, \msidetrace$}
    \State $\mtlink_\mathrm{newS} \gets $ \Call{CreateLink}{$\mtrace\mdot\mnode_S$}
    \State \Call{Connect}{$T, \mlink, \mtlink_\mathrm{newS}$}
    \State \Call{CreateNodelet}{$\mtlink_\mathrm{newS}, \mvnext, \mback, \mtrace\mdot\mnlets_S$}

    \For {$\mtlink_\mathrm{newT} \in \hat{\mlinks}_\mathrm{newT}$}
        \State $\mnode_\mathrm{newT} \gets \fnode(\flink(T, \mtlink_\mathrm{newT}))$
        \State \Call{Anchor}{$\mtlink_\mathrm{newT}, \mtrace\mdot\mnlets_T$}
        \State \Call{Disconnect}{$T, \mlink, \mtlink_\mathrm{newT}$}
        \State \Call{CreateNodelet}{$\mtlink_\mathrm{newT}, \mxtrace - \fx(\mnode_\mathrm{newT}), \mback, \mtrace\mdot\mnlets_T$}
    \EndFor

    \State $\mtrace\mdot\mxtrace \gets $ \Call{Trace}{$\mxtrace, \msidetrace$}
    \State \Call{Tracer}{$\mtrace$}
\EndFunction
\end{algorithmic}
\end{algorithm}

%%%%%%%%%%%%%%%%%%%%%%%%%%%%%%%% ALG: PATHFOUND %%%%%%%%%%%%%%%%%%%%%%%%%%%%%%%%%
\subsubsection{\textproc{PathFound}: \textit{Cumulative Visibility for Both Nodes of Reached Cast }}
The helper function \textproc{PathFound} (Alg. \ref{suppalg:pathfound}) returns the shortest path when the source and target nodes of a cast have cumulative visibility.

If the source node and target node have cumulative visibility, the nodes have to be $\mnvy$-type, as it is impossible for one node to be an $\mney$-node. 
An expensive query will have at least one source-tree or target-tree $\mney$-node along its examined path.
Subsequent casts by expensive queries will only occur if the source or target node of a cast is $\mney$-type.
By ensuring that either the source node or target node is $\mney$-type, the cost-to-go and cost-to-come of  nodes in subsequent casting queries can be verified, respectively.
As such, it is impossible for an expensive path to be unobstructed. 
An expensive path that is unobstructed implies that no cheaper, unobstructed path exists in the open-list, which is impossible since \rtwop{} is complete \cite{bib:r2}.
\begin{algorithm}[!ht]
\begin{algorithmic}[1]
\caption{\textproc{PathFound}: cast reached between two nodes with cumulative visibility.}
\label{suppalg:pathfound}
\Function{PathFound}{$\mlink$}
    % \State $\mnode_S \gets \fnode(\flink(T, \mlink))$
    % \State $\mnode_T \gets \fnode(\flink(S, \mlink))$
    \Comment{Found shortest path because link connects a $\mnvy$ source-tree node and a $\mnvy$ target-tree node.}
    % \State $path$ $\gets \{\fx(\mnode_T), \fx(\mnode_S)\}$
    \Comment{$path$ is accessible to all functions.}
    \State $\mlink_i \gets \flink(T, \mlink)$ 
    \State $path \gets \{\fx(\fnode(\mlink_i))\}$
    \Comment{There is only one target link.}
    \While {front of $path \ne \mxgoal$}
        \State $\mlink_i \gets \flink(T, \mlink_i)$
        \State Push $\fx(\fnode(\mlink_i))$ to front of $path$
    \EndWhile
    \State $\mlink_i \gets \flink(S, \mlink)$
    \State $path \gets $ Push $\fx(fnode(\mlink_i))$ to back of $path$
    \While {back of $path \ne \mxstart$}
        \State $\mlink_i \gets \flink(S, \mlink_i)$
        \State Push $\fx(\fnode(\mlink_i))$ to back of $path$
    \EndWhile
    \State \Return $\mtrue$
\EndFunction
\end{algorithmic}
\end{algorithm}

%%%%%%%%%%%%%%%%%%%%%%%%%%%%%%%% ALG: NOCUMULATIVEVISIBILITY %%%%%%%%%%%%%%%%%%%%%%%%%%%%%%%%%
\subsubsection{\textproc{NoCumulativeVisibility}: \textit{Unknown Cumulative Visibility for Both Nodes of Reached Cast}}
The helper function \textproc{NoCumulativeVisibility} (Alg. \ref{suppalg:nocumulativevisibility}) handles the case when the source and target node of a reached cast do not have verified cumulative visibility to the start or goal node respectively.
Such a case occurs if the source node is $\mnvu$-type, and if the target node is $\mnvu$, $\mnoc$ or $\mntm$-type.
\rtwop{} proceeds by queuing a casting query for each target link of the expanded link $\mlink$.
\begin{algorithm}[!ht]
\begin{algorithmic}[1]
\caption{\textproc{NoCumulativeVisibility}: cast reached between nodes with no cumulative visibility.}
\label{suppalg:nocumulativevisibility}
\Function{NoCumulativeVisibility}{$\mlink$}
    \State $\mnode_S \gets \fnode(\flink(S, \mlink))$
    \State $\mnode_T \gets \fnode(\flink(T, \mlink))$
    \State $\mnode_\mnext \gets $ \Call{GetNode}{$\fx(\mnode_T), \mnvu, \mnode_T\mdot\mside, S)$}
    \State \Call{FinishReachedCast}{$\mtdir_\mnext, \mnode_\mnext, \mlink, \mray$}
    \State \Return ($T, \mnode_\mnext$)
\EndFunction
\end{algorithmic}
\end{algorithm}

%%%%%%%%%%%%%%%%%%%%%%%%%%%%%%%% ALG: SINGLECUMULATIVEIVISIBILITY %%%%%%%%%%%%%%%%%%%%%%%%%%%%%%%%%
\subsubsection{\textproc{SingleCumulativeVisibility}: \textit{Cumulative Visibility for Either Node of Reached Cast}} \label{suppsec:singlecumulativevisibility}
The helper function \textproc{SingleCumulativeVisibility} (Alg. \ref{suppalg:singlecumulativevisibility}) 
when either the source or target node of a trace has cumulative visibility to the start or goal node respectively.

The algorithm progresses by checking nodes with no cumulative visibility, and determining the \textbf{next} direction is important.
If the source node has cumulative visibility, the next node is the target node, and the next direction is in the target-direction.
If the target node has cumulative visibility, the next node is the source node, and the next direction is in the source-direction.
The \textbf{previous} node is the source or target node which is not the next node.

The function updates the minimum cost at the next node's corner if the current query is the cheapest when reaching the next node. If the next node is the source node, the cost-to-go at the source node's corner is checked; if the next node is the target node, the cost-to-come at the target node's corner is checked.
The overlap rule subsequently discards or re-anchors expensive links to expensive nodes in \textproc{ConvToExBranch} (Alg. \ref{suppalg:convtoexbranch}). 

In \rtwo{}, more expensive links are re-anchored at $\mney$-nodes, and an expensive query does not generate additional queries \cite{bib:r2}.
\rtwop{} introduces a new rule to reduce the number of expensive queries further, by discarding the current query if it is expensive and is guaranteed to cross a cheaper path (see Sec. \ref{suppsec:overlap}).
The guarantee and the cheapest cost can be obtained by examining the Best object $\mbest_\mnext$ at the corner.
If the current query is the cheaper or equal to the minimum cost, the query updates $\mbest_\mnext$ instead.

\begin{algorithm}[!ht]
\begin{algorithmic}[1]
\caption{\textproc{SingleCumulativeVisibility}: cast reached between a node with cumulative visibility and another with no cumulative visibility.}
\label{suppalg:singlecumulativevisibility}
\Function{SingleCumulativeVisibility}{$\mray, \mlink$}
        \Comment{Either $\mnode_S$ or $\mnode_T$ has a type that is $\mney$ or $\mnvy$.}
    \State $\mnode_S \gets \fnode(\flink(S, \mlink))$
    \State $\mnode_T \gets \fnode(\flink(T, \mlink))$
    \State $\mtdir_\mnext \gets T$ if $\mnode_S\mdot\mntype \notin \{ \mnvy, \mney \}$ else $S$ 
        \Comment{$\mnode_S\mdot\mntype \notin \{\mnvy, \mney\} \implies \mnode_S\mdot\mntype = \mnvu$} 
    \State $\mnode_\mnext \gets \mnode_S$ if $\mtdir_\mnext = S$ else $\mnode_T$
    \State $\mnode_\mprev \gets \mnode_T$ if $\mtdir_\mnext = S$ else $\mnode_S$

    \If{$\mnode_\mprev\mdot\mntype = \mney$ \An $\mnode_\mprev\mdot\msidenode \ne \mnode_\mnext\mdot\msidenode$}
        \Comment{Discard if a node is expensive and both have different sides.}
        \State \Call{DiscardReachedCast}{$\mlink$}
        \State \Return ($\mtdir_\mnext, \varnothing$)
    \EndIf
    
    \State $\mcost_\mnext \gets $ \Call{MinCost}{$-\mtdir_\mnext, \mlink$} + $\lVert \mray\mdot\mx_T - \mray\mdot\mx_S \rVert$ 
    \State $\mpos_\mnext \gets \fpos(\mnode_\mnext)$
    \State $\mbest_\mnext \gets \fbest(-\mtdir_\mnext, \mpos_\mnext)$
    \State $\mside_\mbest \gets \mbest_\mnext\mdot\mnodebest\mdot\msidenode$
    \State $\mv_\mbest \gets \fx(\mnode_\mnext) - \mbest_\mnext\mdot\mxbest$
    \State $\mv_\mathrm{test} \gets \fx(\mnode_\mnext) - \fx(\mnode_\mprev))$
    \If {$\mbest_\mnext\mdot\mcost < c_\mnext$}
        \Comment{Current path to $\mnode_\mnext$ has larger ($-\mtdir_\mnext$)-cost than minimum at $\fpos(\mnode_\mnext)$.}
       
        \If {$\mnode_\mnext \mdot \msidenode = \mside_\mbest$ \An $\mtdir_\mnext \mside_\mbest(\mv_\mbest \times \mv_\mathrm{test}) > 0$}
            \State \Call{DiscardReachedCast}{$\mlink$}
            \State \Return ($\mtdir_\mnext, \varnothing$)
                \Comment{Future queries is always costlier as their paths cross the cheapest path to $\mx$.}
        \EndIf
        \State $\mnode_\mnext \gets $ \Call{GetNode}{$\fx(\mnode_\mnext), \mney, -\mtdir_\mnext$}
    \ElsIf{$\mbest_\mnext\mdot\mcost > c_\mnext$}
        \Comment{Current path to $\mnode_\mnext$ has smaller ($-\mtdir_\mnext$)-cost than minimum at $\fpos(\mnode_\mnext)$.}
        \State $\mnode_\mnext \gets $ \Call{GetNode}{$\fx(\mnode_\mnext), \mnvy, -\mtdir_\mnext$}
        \State $\mbest_\mnext\mdot\mcost \gets \mcost_\mnext$
        \State $\mbest_\mnext\mdot\mnodebest \gets \mnode_\mnew$ 
        \State $\mbest_\mnext\mdot\mxbest \gets \fx(\mnode_\mprev)$
        \State \Call{ConvToExBranch}{$-\mtdir_\mnext, \mpos_\mnext$}
    \Else
        \Comment{Current path to $\mnode_\mnext$ has identical ($-\mtdir_\mnext$)-cost than minimum at $\fpos(\mnode_\mnext)$.}
        \If {$\mnode_\mnext\mdot\msidenode = \mside_\mbest$ \An $\mtdir_\mnext \mside_\mbest(\mv_\mbest \times \mv_\mathrm{test})  \le 0$}
            \State $\mbest_\mnext\mdot\mxbest \gets \fx(\mnode_\mprev)$
            \Comment{Does not matter if previous node is $\mney$.}
        \EndIf
        \State $\mnode_\mnext \gets $ \Call{GetNode}{$\fx(\mnode_\mnext), \mnode_\mprev\mdot\mntype, -\mtdir_\mnext$}
    \EndIf
    \State \Call{FinishReachedCast}{$\mtdir_\mnext, \mnode_\mnext, \mlink, \mray$}
    \State \Return ($\mtdir_\mnext, \mnode_\mnext$)
\EndFunction
\end{algorithmic}
\end{algorithm}

%%%%%%%%%%%%%%%%%%%%%%%%%%%%%%%% ALG: DiscardReachedCast %%%%%%%%%%%%%%%%%%%%%%%%%%%%%%%%%
\subsubsection{\textproc{DiscardReachedCast}: \textit{Cumulative Visibility for Either Node of Reached Cast}}
The helper function \textproc{DiscardReachedCast} (Alg. \ref{suppalg:discardreachedcast}) discards a reached casting query and removes branches of links that only pass through the expanded link $\mlink$.
\begin{algorithm}[!ht]
\begin{algorithmic}[1]
\caption{\textproc{DiscardReachedCast}: discards the reached casting query.}
\label{suppalg:discardreachedcast}
\Function{DiscardReachedCast}{$\mlink$}
    \State $\mlink_S \gets \flink(S, \mlink)$
    \State \Call{Disconnect}{$T, \mlink_S, \mlink$}
    \State \Call{EraseTree}{$S, \mlink_S$}
    \State \Call{EraseTree}{$T, \mlink$}
\EndFunction
\end{algorithmic}
\end{algorithm}

%%%%%%%%%%%%%%%%%%%%%%%%%%%%%%%% ALG: FinishReachedCast %%%%%%%%%%%%%%%%%%%%%%%%%%%%%%%%%
\subsubsection{\textproc{FinishReachedCast}: \textit{Final Steps for a Reached Cast}}
The helper function \textproc{FinishReachedCast} performs the final steps of a reached cast.
The next node of the cast is converted into a new node, and the expanded link is re-anchored on the new node.
The ray representing the cast is merged into the angular sector of the source node (the rays are stored in the expanded link) if the source node has cumulative visibility.
Overlapping queries at the next node are identified and pushed into the overlapping buffer.
\begin{algorithm}[!ht]
\begin{algorithmic}[1]
\caption{\textproc{FinishReachedCast}: final steps for a reached cast.}
\label{suppalg:finishreachedcast}
\Function{FinishReachedCast}{$\mtdir_\mnext, \mnode_\mnext, \mlink, \mray$}
    \State \Call{Anchor}{$\mlink, \mnode_\mnew$}
    \State $\mlink\mdot\mcost \gets $ \Call{Cost}{$\mlink$}
    \For {$\mlink_\mnext \in \flinks(\mtdir_\mnext, \mlink)$}
        \State \Call{Isolate}{$-\mtdir_\mnext, \mlink_\mnext, \mlink$}
    \EndFor
    \If {$\fnode(\flink(S, \mlink))\mdot\mntype \in \{\mnvy, \mney\}$} 
        \Comment{Merge sector-rays if source node is $\mnvy$ or $\mney$. $\mtdir_\mnext$ is $T$.}
        \State \Call{MergeRay}{$-\mnode_\mnew\mdot\msidenode, \mlink, \mray$}
        \For {$\mlink_\mnext \in \flinks(T, \mlink)$}
            \State \Call{MergeRay}{$\mnode_\mnew\mdot\msidenode, \mlink_\mnext, \mray$}
        \EndFor
    \EndIf
    
    \State $numLinksAll \gets $ sum of $ \lvert \mnode\mdot\mlinks  \rvert $ for all $\mnode \in \fpos(\mnode_\mnext)\mdot\mnodes$ \Comment{Number of links anchored at new node's corner.}
    \State $numLinks \gets 1 + \lvert \flinks(\mtdir_\mnext, \mlink) \rvert$
    \Comment{Number of links anchored at corner by the current casting query.}
    \If {$numLinksAll > numLinks$} 
        \Comment{Trigger overlap rule later if reached a node with other links.}
        \State \Call{PushOverlap}{$\fpos(\mnode_\mnext)$}
    \EndIf
\EndFunction
\end{algorithmic}
\end{algorithm}

%%%%%%%%%%%%%%%%%%%%%%%%%%%%%%%% ALG: QUEUEREACHEDCAST %%%%%%%%%%%%%%%%%%%%%%%%%%%%%%%%%
\subsubsection{\textproc{QueueReachedCast}: \textit{Queue New Queries After a Reached Cast}}
The helper function \textproc{QueueReachedCast} (Alg. \ref{suppalg:queuereachedcast}) queues casting queries for links in the next direction (see Sec. \ref{suppsec:singlecumulativevisibility}).
\begin{algorithm}[!ht]
\begin{algorithmic}[1]
\caption{\textproc{QueueReachedCast}: queues subsequent castable queries.}
\label{suppalg:queuereachedcast}
\Function{QueueReachedCast}{$\mtdir_\mnext, \mlink$}
    \For {$\mlink_\mnext \in \flinks(\mtdir_\mnext, \mlink)$}
        \Comment{Queue next casting queries.}
        \State \Call{Queue}{$\mqcast, \mlink\mdot c + \mlink_\mnext\mdot c, \mlink_\mnext$}
    \EndFor
\EndFunction
\end{algorithmic}
\end{algorithm}

%%%%%%%%%%%%%%%%%%%%%%%%%%%%%%%%% ALG: CASTERCOLLIDED  %%%%%%%%%%%%%%%%%%%%%%%%%%%%%%%%%%%%%
\subsection{\textproc{CastCollided}: \textit{No Line-of-sight Between Nodes of Cast}}
The function \textproc{CastCollided} (Alg. \ref{suppalg:castcollided}) generates traces when a cast collides.
The \textbf{minor-trace} is generated from the collision point and has a side that is different from the source node of the cast.
If the target node is the goal node, and the source node is not a start node, the \textbf{third-trace} is generated from the source node.
The third-trace has a side that is the same as the source node.
The \textbf{major-trace} is generated from the collision point and has a side that is the same as the source node of the cast.

% Fig. \ref{suppfig:castcollided}.
\begin{algorithm}[!ht]
\begin{algorithmic}[1]
\caption{\textproc{CastCollided}: cast collided and ray has no line-of-sight.}
\label{suppalg:castcollided}
\Function{CastCollided}{$\mray, \mlink$}
    \State \Call{MinorTrace}{$\mray, \mlink$}
    \State \Call{ThirdTrace}{$\mray, \mlink$}
    \State \Call{MajorTrace}{$\mray, \mlink$}
\EndFunction
\end{algorithmic}
\end{algorithm}

%%%%%%%%%%%%%%%%%%%%%%%%%%%%%%%%% ALG: MINORTRACE  %%%%%%%%%%%%%%%%%%%%%%%%%%%%%%%%%%%%%
\subsubsection{\textproc{MinorTrace}: \textit{Generates a Trace With Different Side From Source Node}}
When a cast collides, the helper function \textproc{MinorTrace} (Alg. \ref{suppalg:minortrace}) generates a trace from the collision point. The trace, called the \textit{minor-trace}, has a side that is different from the source node.
The ray of the collided cast is merged into the source node of the cast, via a trace-link.

The reader may choose to ignore the third-trace (Alg. \ref{suppalg:thirdtrace}) if the minor-trace traces back  and re-encounters the source node of the cast.
The default implementation of \rtwop{} introduces an additional variable to the Trace object $\mtrace$ to monitor a re-encounter. However, if the minor-trace is interrupted, the re-encounter can no longer be monitored.
The monitoring is not shown in the pseudocode, as the additional step is not necessary for \rtwop{} to work.
\begin{algorithm}[!ht]
\begin{algorithmic}[1]
\caption{\textproc{MinorTrace}: minor-trace for a collided cast.}
\label{suppalg:minortrace}
\Function{MinorTrace}{$\mray, \mlink$}
    \State $\mnode_S \gets \fnode(\flink(S, \mlink))$
    \State $\mside_\mmnr \gets -\mnode_S\mdot\msidenode$
    \State $\mvray \gets \mray\mdot\mx_T - \mray\mdot\mx_S$
    \If {$\mnode_S\mdot\mntype = \mney$}
        \State \Return \Comment{Minor Trace cannot be generated for $\mney$ source node }
    \EndIf \Comment{The reader may choose to return if $\fxcol(\mside_\mmnr, \mray)$ is at the map boundary.}
    \State $\mtrace_\mmnr \gets $ \Call{CreateTrace}{$\fxcol(\mside_\mmnr, \mray), \mside_\mmnr$}
    \Comment{Create source nodelet and trace-link.}
    \State $\mtlink_\mathrm{newS} \gets $ \Call{CopyLink}{$\mlink, \mtrace_\mmnr\mdot\mtnode_S, \{S\}$}
    \State \Call{MergeRay}{$-\mside_\mmnr, \mtlink_\mathrm{newS}, \mray$}
    \State \Call{CreateNodelet}{$\mtlink_\mathrm{newS}, \mvray, \mback, \mtrace_\mmnr\mdot\mnlets_S$}
    \Comment{Create target nodelet and trace-link.}
    \State $\mtlink_\mathrm{newT} \gets $ \Call{CreateLink}{$\mtrace_\mmnr\mdot\mtnode_T$}
    \For {$\mlink_T \in \mlink\mdot\mlinks_T$}
        \State \Call{Connect}{$T, \mtlink_\mathrm{newT}, \mlink_T$}
    \EndFor
    \State \Call{CreateNodelet}{$\mtlink_\mathrm{newT}, -\mvray, \mback, \mtrace_\mmnr\mdot\mnlets_T$}
    \State \Call{Tracer}{$\mtrace_\mmnr$}
\EndFunction
\end{algorithmic}
\end{algorithm}

%%%%%%%%%%%%%%%%%%%%%%%%%%%%%%%%% ALG: THIRDTRACE  %%%%%%%%%%%%%%%%%%%%%%%%%%%%%%%%%%%%%
\subsubsection{\textproc{ThirdTrace}: \textit{Generates a Third Trace}}
When a cast from a non-start point to the goal point collides, the helper function \textproc{ThirdTrace} (Alg. \ref{suppalg:thirdtrace}) generates a trace from the source node.
The trace is called the \textit{third-trace}, which has the same side as the source node.
The ray of the collided cast is merged into the source node of the cast, via a trace-link.
\begin{algorithm}[!ht]
\begin{algorithmic}[1]
\caption{\textproc{ThirdTrace}: third-trace for a collided cast.}
\label{suppalg:thirdtrace}
\Function{ThirdTrace}{$\mray, \mlink$}
    \If {$\mray\mdot\mx_T \ne \mxgoal$ \Or $\mnode_S\mdot\mntype = \mney$}
        \State \Return 
        \Comment{Can ignore third-trace if minor-trace refinds source node...}
    \EndIf  
    \Comment{... or if $\mnode_S$ lies on an edge touching the map boundary.}
    \State $\mnode_S \gets \fnode(\flink(S, \mlink))$
    \State $\mside_\mthird \gets \mnode_S\mdot\msidenode$
    \State $\mvray \gets \mray\mdot\mx_T - \mray\mdot\mx_S$
    \State $\mtrace_\mthird \gets $ \Call{CreateTrace}{$\fx(\mnode_S), \mside_\mthird)$}
    \State $\mtrace_\mthird\mdot\mxtrace \gets $ \Call{Trace}{$\mtrace_\mthird\mdot\mxtrace,  \mtrace_\mthird\mdot\msidetrace$}
    \Comment{Third-trace begins at corner after source node.}
    
    \State $\mtlink_\mathrm{newS} \gets $ \Call{CopyLink}{$\mlink, \mtrace_\mthird\mdot\mnode_S, \{S\}$} \Comment{Create source nodelet and trace-link.}
    \State \Call{MergeRay}{$\mside_\mthird, \mtlink_\mathrm{newS}, \mray$}
    \State \Call{CreateNodelet}{$\mtlink_\mathrm{newS}, \mtrace_\mthird\mdot\mxtrace - \fx(\mnode_S), \mback, \mtrace_\mthird\mdot\mnlets_S$}

    \State $\mnode_\mathrm{newUn} \gets $ \Call{GetNode}{$\fx(\mnode_S), \mnun, \mside_\mthird, T$} 
    \Comment{Create a target-tree $\mnun$ node and link at casting point.}
    \State $\mlink_\mathrm{newUn} \gets $ \Call{CreateLink}{$\mnode_\mathrm{newUn}$}
    \For {$\mlink_T \in \mlink\mdot\mlinks_T$}
        \State \Call{Connect}{$T, \mlink_\mathrm{newUn}, \mlink_T$}
    \EndFor
    \State $\mlink_\mathrm{newUn}\mdot c \gets $ \Call{Cost}{$\mlink_\mathrm{newOc}$}

    \State $\mx_\mathrm{newOc} \gets $ \Call{Trace}{$\fx(\mnode_S), -\mside_\mthird$} 
    \Comment{Create a target-tree $\mnoc$ node and link at the corner before source node.}
    \State $\mnode_\mathrm{newOc} \gets $ \Call{GetNode}{$\mx_\mathrm{newOc}, \mnoc, \mside_\mthird, T$}
    \State $\mlink_\mathrm{newOc} \gets $ \Call{CreateLink}{$\mnode_\mathrm{newOc}$}
    \State \Call{Connect}{$T, \mlink_\mathrm{newOc}, \mlink_\mathrm{newUn}$}
    \State $\mlink_\mathrm{newOc}\mdot c \gets $ \Call{Cost}{$\mlink_\mathrm{newOc}$}

    \State $\mtlink_\mathrm{newT} \gets $ \Call{CreateLink}{$\mtrace_\mthird\mdot\mtnode_T$} 
    \Comment{Create target nodelet and trace-link.}
    \State \Call{Connect}{$T, \mtlink_\mathrm{newT}, \mlink_\mathrm{newOc}$}
    \State \Call{CreateNodelet}{$\mtlink_\mathrm{newT}, \mtrace_\mthird\mdot\mxtrace - \mx_\mathrm{newOc}, \mback, \mtrace_\mthird\mdot\mnlets_T$}

    \State \Call{Tracer}{$\mtrace_\mthird$}
\EndFunction
\end{algorithmic}
\end{algorithm}

%%%%%%%%%%%%%%%%%%%%%%%%%%%%%%%%% ALG: MAJORTRACE  %%%%%%%%%%%%%%%%%%%%%%%%%%%%%%%%%%%%%
\subsubsection{\textproc{MajorTrace}: \textit{Generates a Trace with Same Side as Source Node}}
When a cast collides, the helper function \textproc{MajorTrace} generates a trace from the collision.
The trace, called the \textit{major-trace}, has the same side as the source node.
The ray of the collided cast is merged into the source node of the cast, via a trace-link.
\begin{algorithm}[!ht]
\begin{algorithmic}[1]
\caption{\textproc{MajorTrace}: major-trace for a collided cast.}
\label{suppalg:majortrace}
\Function{MajorTrace}{$\mray, \mlink$}
    \State $\mnode_S \gets \fnode(\flink(S, \mlink))$
    \State $\mside_\mmjr \gets \mnode_S\mdot\msidenode$
    \State $\mvray \gets \mray\mdot\mx_T - \mray\mdot\mx_S$
    \State $\mtrace_\mmjr \gets $ \Call{CreateTrace}{$\fxcol(\mside_\mmjr, \mray)$}
    
    \State \Call{Anchor}{$\mlink, \mtrace_\mmjr\mdot\mtnode_S$}
    \Comment{$\mlink$ becomes source trace-link; Create source nodelet.}
    \State \Call{MergeRay}{$-\mside_\mmjr, \mlink, \mray$}
    \State \Call{CreateNodelet}{$\mlink, \mvray, \mback, \mtrace_\mmjr\mdot\mnlets_S$}

    \State $\mtlink_\mathrm{newT} \gets $ \Call{CreateLink}{$\mtrace_\mmjr\mdot\mnode_T$}
    \Comment{Create target nodelet and trace-links.}
    \For{$\mlink_T \in \mlink\mdot\mlinks_T$}
        \State \Call{Disconnect}{$T, \mlink, \mlink_T$} 
        \Comment{Connections in $\mlink$ prevents its removal if the mnr. or thd. traces fail.}
        \State \Call{Connect}{$T, \mtlink_\mathrm{newT}, \mlink_T$}
    \EndFor
    \State \Call{CreateNodelet}{$\mtlink_\mathrm{newT}, -\mvray, \mback, \mtrace_\mmjr\mdot\mnlets_T$}

    \State \Call{Tracer}{$\mtrace_\mmjr$}
\EndFunction
\end{algorithmic}
\end{algorithm}
%%%%%%%%%%%%%%%%%%%%%%%%%%%%%%%%% ALG: TRACER  %%%%%%%%%%%%%%%%%%%%%%%%%%%%%%%%%%%%%
\newpage
\section{\textproc{Tracer}: \textit{Handles a Tracing Query}} 
\setcounter{algorithm}{0}

The main tracing function \textproc{Tracer} (Alg. \ref{suppalg:tracer}) implements the tracing query.
While 
There is only \textit{one} source nodelet during a trace, at at least one target nodelet.
The tracing query makes use of ordered set of nodelets $\mnlets_S$ and $\mnlets_T$ to prune, place and examine nodes.
Each nodelet contains a trace-link which connects a trace-node to a parent node, allowing the algorithm to examine a parent node with respect to the trace.
The source nodelet examines a source node, while a target nodelet examines a target node.
The source node lies on the source-tree, while the target node lies on the target-tree.

% Fig. \ref{supp:suppfig:tracer}.

Each iteration in \textproc{Tracer} evaluates a corner at $\mxtrace$.
If the trace traces to the source node (\textproc{RefoundSrc}, Alg. \ref{suppalg:refoundsrc}), the query is discarded.
If the trace does not progress with respect to the source node, \textproc{SrcProgCast} (Alg. \ref{suppalg:srcprogcast}) is called and a casting query is generated from the source node if the angular progression decreased by more than $180^\circ$ with respect to the source node. 
Otherwise, if the progression decreases by less than $180^\circ$, the trace moves to the next corner without evaluating the nodes.

If the trace has progressed with respect to the source node, the source and target nodes are examined further.
\textproc{TracerProc} (Alg. \ref{suppalg:tracerproc}) evaluates the target nodes with the progression, occupied-sector, and pruning rules.
\textproc{TracerProc} subsequently evaluates the source node with the angular-sector, occupied-sector, and pruning rules, which generates a recursive trace and discards the current trace if necessary.
\textproc{TracerProc} for the target nodes is called before the source node to ensure that the path is taut when a recursive trace is generated.

The interrupt rule interrupts the trace in \textproc{InterruptRule} (Alg. \ref{suppalg:interrupt}) if several corners are traced.
The placement rule in \textproc{PlaceRule} (Alg. \ref{suppalg:placerule}) tries to place a turning point or phantom point at the current position, and casts to any potentially visible target node from a placed turning point.
The placement rule engages the overlap rule instead if the query crossed paths with other queries. 

\begin{algorithm}[!ht]
\begin{algorithmic}[1]
\caption{\textproc{Tracer}: handles a tracing query.}
\label{suppalg:tracer}
\Function{Tracer}{$\mtrace$}
    \DoWhile
    \Comment{There is only one source link, and $\mtrace\mdot\mnlets_S = \{\mnlet_S\}$}
        \State $\mtrace\mdot\mnumcrns \gets \mtrace\mdot\mnumcrns + 1$
        % \State $\mnlet_S \gets $ the only trace-node in $\mtrace\mdot\mnlets_S$
        \If {\Call{RefoundSrc}{$\mtrace$}}
            \Comment{Refound source node}
            \State \Break
        \ElsIf {\Call{ProgRule}{$\mtrace, \fnlet(S, \mtrace)$}}
            \Comment{Not prog. w.r.t. source node.}
            \If {\Call{SrcProgCast}{$\mtrace$}}
                \Comment{Prog. reversed by $>180^\circ$ w.r.t. source node.}
                \State \Break
            \EndIf
        \Else
            \Comment{Prog. w.r.t. source node.}
            \If {\Call{TracerProc}{$T, \mtrace$}} \Comment{Order of execution is important.}
                \State \Break
            \ElsIf {\Call{TracerProc}{$S, \mtrace$}}
                \State \Break
            \ElsIf {\Call{InterruptRule}{$\mtrace$}}
                \State \Break
            \ElsIf {\Call{PlaceRule}{$\mtrace$}}
                \State \Break
            \EndIf
        \EndIf
        \State $\mtrace\mdot\mxtrace \gets $ \Call{Trace}{$\mtrace\mdot\mxtrace, \mtrace\mdot\msidetrace$}
    \EndDoWhile{$\mtrace\mdot\mxtrace \ne \varnothing$}
    \Comment{While trace is in map.}

    \For {$\mtdirpar \in \{S, T\}$} \Comment{Delete all dangling links.}
        \For {$\mnlet \in \fnlets(\mtdirpar, \mtrace)$}
            \State \Call{EraseTree}{$\mtdirpar, \mnlet\mdot\mtlink$}
        \EndFor
    \EndFor

\EndFunction
\end{algorithmic}
\end{algorithm}

%%%%%%%%%%%%%%%%%%%%%%%%%%%%%%%%% ALG: TRACERFROMLINK %%%%%%%%%%%%%%%%%%%%%%%%%%%%%%%%%%%%%
\subsection{\textproc{TracerFromLink}: \textit{Wrapper for} \textproc{Tracer}} \label{suppsec:tracerfromlink}
The tracing function \textproc{TracerFromLink} (Alg. \ref{suppalg:tracerfromlink}) wraps \textproc{Tracer} (Alg. \ref{suppalg:tracer}). 
\textproc{TracerFromLink} prepares a tracing query from a link $\mlink$ and calls \textproc{Tracer}.
The function is called when a tracing query is polled from the open-list (Alg. \ref{suppalg:run}), 
or when a $\mntm$-node is reached by a cast (Alg. \ref{suppalg:reachedtm}). 
\begin{algorithm}[!ht]
\begin{algorithmic}[1]
\caption{\textproc{TracerFromLink}: prepares a tracing query from a link.}
\label{suppalg:tracerfromlink}
\Function{TracerFromLink}{$\mlink$}
    \State $\mnode \gets \fnode(\mlink)$
    \State $\mnode_S \gets \fnode(\flink(S, \mlink))$
    \State $\mtrace \gets $ \Call{Tracer}{$\fx(\mnode), \mnode\mdot\msidenode$}
    \State \Call{Anchor}{$\mlink, \mtrace\mdot\mnode_S$}
    \State \Call{CreateNodelet}{$\mlink, \fx(\mnode) - \fx(\mnode_S), \mback, \mtrace\mdot\mnlets_S$}

    \For {$\mlink_T \in \mlink\mdot\mlinks_T$}
        \State $\mnode_T \gets \fnode(\flink(T, \mlink))$
        \State \Call{Disconnect}{$T, \mlink, \mlink_T$}
        \State \Call{Anchor}{$\mlink_T, \mtrace\mdot\mnode_T$}
        \State \Call{CreateNodelet}{$\mlink_T, \fx(\mnode) - \fx(\mnode_T), \mback, \mtrace\mdot\mnlets_T$}
    \EndFor

    \State \Call{Tracer}{$\mtrace$}
\EndFunction
\end{algorithmic}
\end{algorithm}

%%%%%%%%%%%%%%%%%%%%%%%%%%%%%%%%% ALG: TRACERPROC  %%%%%%%%%%%%%%%%%%%%%%%%%%%%%%%%%%%%%
\subsection{\textproc{TracerProc}: \textit{Process Source or Target-tree Nodes in Trace}}
Function \textproc{TracerProc} (\ref{suppalg:tracerproc}) examines the source node or target nodes. 
The function relies on the ordered set of nodelets $\mnlets_S$ and $\mnlets_T$ stored in the Trace object $\mtrace$ to examine the nodes.
If the trace is discarded or interrupted, either set becomes empty and the function returns.
While there can be multiple target nodelets at all times during a trace, there is always only \textit{one} source nodelet.

When \textproc{TracerProc} is called for the source node ($\mtdirpar=S$), the source node is first examined by the angular-sector rule. 
If the trace is no longer within the angular-sector of the node and the trace is unable to continue, the trace is interrupted or discarded.
Otherwise, the pruning rule or occupied-sector rule is checked depending on the side of the source node. If the trace has the same side as the source node, the pruning rule examines the source node. Otherwise, the occupied-sector rule examines the source node. 
The occupied-sector rule may interrupt the current trace with a recursive occupied-sector trace.

When \textproc{TracerProc} is called for the target nodes ($\mtdirpar=T$), the function checks the angular progression with respect to each target node before proceeding to the occupied-sector rule or pruning rule.
As the recursive occupied-sector trace for a target node ends quickly, the current trace will not be interrupted when the target nodes are examined.

\begin{algorithm}[!ht]
\begin{algorithmic}[1]
\caption{\textproc{TracerProc}: processes the trace in the source or target direction.}
\label{suppalg:tracerproc}
\Function{TracerProc}{$\mtdirpar, \mtrace=(\mxtrace, \msidetrace, \cdots)$}
    \For {$\mnlet \in \fnlets(\mtdirpar, \mtrace)$}
        \State $\mnodepar \gets \fnode(\mnlet\mdot\mtlink)$
        \State $\msidepar \gets \mnodepar\mdot\msidenode$
        \If {$\mtdirpar = T$ \An \Call{ProgRule}{$\mtrace, \mnlet$}}
            \State \Continue
        \ElsIf {$\mtdirpar = S$ \An \Call{AngSecRule}{$\mtrace, \mnlet$}        }
            \State \Continue 
        \ElsIf {$\fx(\mnodepar) \in \{\mx_\mstart, \mx_\mgoal \}$} 
            \Comment{Parent node is start or goal node.}
            \State \Continue
        \ElsIf {$\msidepar = \msidetrace$}
            \State \Call{PruneRule}{$\mtrace, \mnlet$}
        \Else 
            \State \Call{OcSecRule}{$\mtrace, \mnlet$}
        \EndIf
    \EndFor
    \State \Return $\fnlets(\mtdirpar, \mtrace) = \{\}$
    \Comment{Returns true if the $\mtdirpar$ set of nodelets is empty.}
\EndFunction
\end{algorithmic}
\end{algorithm}

%%%%%%%%%%%%%%%%%%%%%%%%%%%%%%%%% ALG: SRCPROGCAST  %%%%%%%%%%%%%%%%%%%%%%%%%%%%%%%%%%%%%
\subsection{\textproc{SrcProgCast}: \textit{Cast From Highly Winded Source Node}}
The \textproc{SrcProgCast} function (Alg. \ref{suppalg:srcprogcast}) interrupts the trace when the winding counter increases to two for the source node. When the counter increases to two, the progression has decreased by more than $180^\circ$ from the maximum angular progression.
The maximum angular progression points to a phantom point, which is replaced with an unreachable $\mnun$-node.
A casting query is subsequently queued from the source node to the $\mnun$-node.

The phantom point can be found directly from the only target trace-node when the trace is not progressed with respect to the source node.
The point can be found as no target nodes are placed when the angular progression is reversing for the source node, and the trace is in the convex hull of a non-convex obstacle.
No target nodes need to be placed in a convex hull as they would be pruned once the trace exits the convex hull and resumes angular progression with respect to the source node.
% Fig. \ref{suppfig:srcprogcast}
\begin{algorithm}[!ht]
\begin{algorithmic}[1]
\caption{\textproc{SrcProgCast}: queues a cast when progression w.r.t. source node has decreased by more than $180^\circ$.}
\label{suppalg:srcprogcast}
\Function{SrcProgCast}{$\mtrace = (\mxtrace, \cdots)$}
    \State $\mnlet_S \gets \fnlet(S, \mtrace)$
    \If {$\mnlet_S\mdot\mcprog > 1$}
    
        \Comment{(A) Create new target-tree $\mnun$-node and anchor target link there.}
        \State $\mnlet_T \gets \fnlet(T, \mtrace)$ 
        \Comment{The only target nodelet.}
        \State $\mlink_T \gets \flink(T, \mnlet_T\mdot\mtlink)$
        \State $\mnode_T \gets \fnode(\mlink_T)$ 
        \Comment{Target node is a phantom point.}
        \State $\mnode_\mathrm{newUn} \gets $ \Call{GetNode}{$\fx(\mnode_T), \mnun, \mnode_T\mdot\msidenode, T$}
        \State \Call{Anchor}{$\mlink_T, \mnode_\mathrm{newUn}$}

        \Comment{(B) Create new target-tree $\mnvu$-node and re-anchor source trace-link there.}
        \State $\mlink_\mathrm{newVu} \gets \mnlet_S\mdot\mtlink$
        \State $\mlink_S \gets \flink(S, \mlink_\mathrm{newVu})$
        \State $\mnode_S \gets \fnode(\mlink_S)$
        \State $\mnode_\mathrm{newVu} \gets $ \Call{GetNode}{$\fx(\mnode_S), \mnvu, \mnode_S\mdot\msidenode, T$}
        \State \Call{Anchor}{$\mlink_\mathrm{newVu}, \mnode_\mathrm{newVu}$}
        \State \Call{Connect}{$T, \mlink_\mathrm{newVu}, \mlink_T$}
        \State $\mlink_\mathrm{newVu}\mdot\mcost \gets $ \Call{Cost}{$\mlink_\mathrm{newVu}$}

        \Comment{(C) Queue casting query for source trace-link.}
        \State \Call{Queue}{$\mqcast, \mlink_S\mdot\mcost + \mlink_\mathrm{newVu}\mdot\mcost, \mlink_\mathrm{newVu}$}
        \State \Return $\mtrue$
    \EndIf
    \State \Return $\mfalse$
\EndFunction
\end{algorithmic}
\end{algorithm}

%%%%%%%%%%%%%%%%%%%%%%%%%%%%%%%%% ALG: REFOUNDSRC  %%%%%%%%%%%%%%%%%%%%%%%%%%%%%%%%%%%%%
\subsection{\textproc{RefoundSrc}: \textit{Checks if Trace Traces to Source Node}}
Function \textproc{RefoundSrc} (Alg. \ref{suppalg:refoundsrc}) returns $\mtrue$ if a trace traces to its examined source node.
A trace can never trace to a target node in \rtwop.
\begin{algorithm}[!ht]
\begin{algorithmic}[1]
\caption{\textproc{RefoundSrc}: checks if a trace has reached its source node.}
\label{suppalg:refoundsrc}

\Function{RefoundSrc}{$\mtrace = (\mxtrace, \cdots)$}
    \State $\mnlet_S \gets \fnlet(S, \mtrace)$
    \State $\mnode_S \gets \fnode(\mnlet_S\mdot\mtlink)$
    \State \Return $\mxtrace = \fx(\mnode_S)$
\EndFunction
\end{algorithmic}
\end{algorithm}

%%%%%%%%%%%%%%%%%%%%%%%%%%%%%%%%% ALG: PROGRULE  %%%%%%%%%%%%%%%%%%%%%%%%%%%%%%%%%%%%%
\clearpage
\subsection{\textproc{ProgRule}: \textit{Checks Angular Progression w.r.t. a Node}}
Function \textproc{ProgRule}  (Alg. \ref{suppalg:progrule}) returns $\mfalse$ if the trace at corner $\mxtrace$ has progressed with respect to a parent node or $\mtrue$ if the trace has not progressed. 

If a trace crosses the progression ray, it will intersect a line (unbounded on both sides) coincident to the ray (bounded on one side). 
The progression ray is drawn from a parent node in the direction $\mvprog$ and stretches to infinity. If a trace crossed the front of the ray, the trace intersected the ray.
Let $\mvprog'$ be a ray that is drawn from a parent node in the direction $-\mvprog$. If a trace crossed behind the ray, then the trace crossed $\mvprog'$.

As only the direction of the intersection with respect to the parent node needs to be known, the intersection need not be calculated explicitly. 
Let $itx =  \fsgn(\mvprev \times \mv_\mpar) \fsgn(\mvprev \times \mvprog ) \in {-1, 0, 1}$. 
$\mvprev$ is the previous trace direction that reached $\mx$. $\mv_\mpar$ is the vector pointing from the parent node to $\mx$. $\mvprog$ is the progression ray.
$-1$ and $1$ indicate that the trace has crossed behind and in front of the ray respectively. $0$ indicates that $\mvprev$ is parallel to $\mv_\mpar$ and/or $\mvprev$ is parallel to $\mvprog$. 
For both parallel cases, the reader may verify that the trace is always progressed with respect to the parent node.
Note that $\mvprog \ne 0$, $\mvprev \ne 0$ and $\mvprog \ne 0$ when $itx$ is evaluated.
\begin{algorithm}[!ht]
\begin{algorithmic}[1]
\caption{\textproc{ProgRule}: implements the progression rule.}
\label{suppalg:progrule}
\Function{ProgRule}{$\mtrace = (\mxtrace, \msidetrace, \cdots)$, $\mnlet = (\mtlink, \mvprog, \mcprog) $}
% \State $(\mtdirpar, \msidepar, \mnodepar, \mvpar, \mvprev, \sim) \gets $\Call{TraceCalc}{$\mtrace, \mnlet$}
    \State $\mnodepar \gets \fnode(\mtlink)$
    \State $\mtdirpar \gets \mnodepar\mdot\mtdirnode$ 
    \State $\mvpar \gets \mxtrace - \fx(\mnodepar)$
    \State $\mvprev \gets -$\Call{GetEdge}{$\mxtrace, -\msidetrace$} 
\If{ $\mvpar = 0$} 
    \State $\mvpar \gets $\Call{Bisect}{$\mxtrace$} \Comment{Occurs for start nodes or checkerboard corners}
\EndIf
\State $u \gets \mtdirpar \msidetrace (\mvpar \times \mvprog)$
\State $isProg \gets u < 0 $ \Or ($u = 0$ \An $\mvpar \sdot \mvprog > 0$) \Comment{$\mtrue$ if $\mvpar$ lies to $(\mtdirpar \msidetrace)$-side of $\mvprog$, or if both are pointing in same direction }
\State $wasProg \gets \mcprog = 0$

\State $itx \gets \fsgn(\mvprev \times \mvpar) \fsgn(\mvprev \times \mvprog )$ \Comment{$itx = 1$:  crossed in front of ray; $itx =-1$: crossed behind ray.}
\If {$isProg = \mtrue$ \An $wasProg = \mtrue$}
    \State $\mnlet\mdot\mvprog \gets \mvpar$ \Comment{Update ray}
\ElsIf {$isProg = \mtrue$ \An $wasProg = \mfalse$}
    \If {$itx \ge 0$}
        \State $\mnlet\mdot\mcprog \gets \mcprog - 1$ \Comment{Unwind}
        \If {$\mcprog > 0$}  \Comment{Not completely unwound, flip ray}
            \State $\mnlet\mdot\mvprog \gets -\mvprog$ 
            \State $isProg \gets \mfalse$
        \Else \Comment{Unwound completely, update ray}
            \State $\mnlet\mdot\mvprog \gets \mvpar$ 
        \EndIf
    \Else  \Comment{Wind and flip ray}
        \State $\mnlet\mdot\mcprog \gets \mcprog + 1$
        \State $\mnlet\mdot\mvprog \gets -\mvprog$ 
        \State $isProg \gets \mfalse$
    \EndIf
\ElsIf{$isProg = \mfalse$ \An $wasProg = \mtrue$} 
    \If {$itx \le 0$} \Comment{No winding: case occurs if start node lies on an obstacle's edge}
        \State $\mnlet\mdot\mvprog \gets -\mvprog$
        \State $isProg \gets \mtrue$
    \Else  \Comment {Wind}
        \State $\mnlet\mdot\mcprog \gets \mcprog + 1$ 
    \EndIf
\EndIf
\State \Return \Not $isProg$
\EndFunction
\end{algorithmic}
\end{algorithm}

%%%%%%%%%%%%%%%%%%%%%%%%%%%%%%%%% ALG: PRUNERULE  %%%%%%%%%%%%%%%%%%%%%%%%%%%%%%%%%%%%%
\clearpage
\subsection{\textproc{PruneRule}: \textit{Checks if a Node can be Pruned}}
Function \textproc{PruneRule} (Alg. \ref{suppalg:prune}) prunes a node if the resulting path at the examined corner at $\mxtrace$ is not taut. A source-tree node that is $\mnvy$ cannot be pruned by the rule, as it is handled by the angular-sector rule.

Pruning of source-tree $\mnvy$-nodes are handled by the angular-sector. 
As the angular-sector of a source-tree $\mnvy$-node can only be fully evaluated at the next corner, any pruning at the current corner can cause \rtwop{} to be incomplete.

\begin{algorithm}[!ht]
\begin{algorithmic}[1]
\caption{\textproc{PruneRule}: implements the pruning rule.}
\label{suppalg:prune}
\Function{PruneRule}{$\mtrace = (\mxtrace, \msidetrace, \cdots)$, $\mnlet = (\mtlink, \cdots) $}
    \State $\mnodepar \gets \fnode(\mtlink)$
    \State $\mtdirpar \gets \mnodepar\mdot\mtdirnode$ 
    \State $\msidepar \gets \mnodepar\mdot\msidenode$
    \State $\mvpar \gets \mxtrace - \fx(\mnodepar)$

    \Comment{\textbf{(A) $\mnvy$ source-tree nodes are handled by the angular sector rule.}}
\If{$\mtdirpar = S$ \An $\mnodepar \mdot \mntype = \mnvy$}
    \State \Return 
\EndIf 

    \Comment{(B) Try pruning for each parent node and link.}
\For{$\mlinkpar \in \flinks(\mtdirpar, \mtlink)$}

    \Comment{(B.1) Taut: go to next parent node and link.}
    \State $\mnodegpar \gets \fnode(\flink(\mtdirpar, \mlinkpar))$
    \State $\mvgpar \gets \fx(\mnodepar) - \fx(\mnodegpar)$  
    \If {\Call{IsTaut}{$\mtdirpar$, $\msidepar$, $\mvpar$, $\mvgpar$}}
        \State \Continue
        \Comment{$(\mxtrace, \mnodepar), \mnodegpar)$ is taut and nothing is pruned.}
    \EndIf

    \Comment{(B.2) Not taut: prune parent node.}
    \State \Call{Disconnect}{$-\mtdirpar$, $\mlinkpar$, $\mtlink$} 
    \State $\mlink_\mnew \gets $ \Call{Isolate}{$-\mtdirpar$, $\mlinkpar$, $\varnothing$, $\ftnode(\mtdirpar, \mtrace)$}
    \If{$\mtdirpar = T$} 
        \Comment{Remove rays if prune in target direction.}
        \State $\mlink_\mnew \mdot \mray_L \gets \varnothing$
        \State $\mlink_\mnew \mdot \mray_R \gets \varnothing$
    \EndIf

    % \Comment{(B.3) Not taut: If new parent node is target-tree $\mnph$ or $\mnun$, re-anchor new parent links to $\mntm$ parent node.}
    % \If{$\mnode_\mpar \mdot \mntype \in \{\mntm,\mnun\}$ \An $\mnode_\mgpar \mdot \mntype = \mnph$} 
    % % \Comment{Move links from old gpar. $\mnph$ nodes to $\mntm$ if old par. node is $\mntm$.} 
    %     \State $\mnode_\mathrm{newT} \gets $ \Call{GetNode}{$\fx(\mnode_\mgpar)$,  $\mnode_\mpar\mdot\mntype$, ($\mnode_\mgpar \mdot \msidenode$), $\mtdirpar$}
    %     \For {$\mlink_\mnph \in \flinks_\mpar(\mlink_\mpar)$} 
    %         \State $\mlink_\mathrm{newT} \gets $ \Call{Isolate}{$-\mtdirpar$, $\mlink_\mnph$, $\mlink_\mnew$, $\mnode_\mathrm{newT}$} 
    %     \EndFor
    % \EndIf

    \Comment{(B.4) Create new nodelet for new parent node.}
    \State \Call{CreateNodelet}{$\mlink_\mnew, \mx_\mtrace - \fx(\mnode_\mgpar), \mback, \fnlets(\mtdirpar, \mtrace)$} 
    \Comment{Push to back to try pruning later.}
        
\EndFor

        \Comment{(C) Remove current nodelet and trace-link if trace-link has no more parent links.}
\If {$\flinks(\mtdirpar, \mtlink)  = \{\}$ } 
    \State Remove $\mtlink$ from $\ftnode(\mtdirpar, \mtrace)\mdot\mlinks_\mnode$ 
    \State Remove $\mnlet$ from $\fnlets(\mtdirpar, \mtrace)$
\EndIf
\EndFunction
\end{algorithmic}
\end{algorithm}

%%%%%%%%%%%%%%%%%%%%%%%%%%%%%%%%% ALG: PRUNERULE  %%%%%%%%%%%%%%%%%%%%%%%%%%%%%%%%%%%%%
\clearpage
\subsubsection{\textproc{IsTaut}: \textit{Checks if a Node is Taut}}
The helper function \textproc{IsTaut} (Alg. \ref{suppalg:istaut}) evaluates the path segments around a node and returns $\mtrue$ if the node can be pruned.
\begin{algorithm}[!ht]
\begin{algorithmic}[1]
\caption{\textproc{IsTaut}: checks tautness of path segment.}
\label{suppalg:istaut}
\Function{IsTaut}{$\mtdirpar$, $\msidepar$, $\mvpar$, $\mvgpar$}
    \State $u \gets \mtdirpar \msidepar (\mvpar \times \mvgpar)$ 
    \If {$u = 0$} \Comment{Return $\mtrue$ if angle between $\mvpar$ and $\mvgpar$ is $180^\circ$, $\mfalse$ if $0^\circ$}
        \State \Return $\mvpar \sdot \mvgpar \ge 0$ 
    \Else \Comment{Returns $\mtrue$ if $\mvgpar$ lies to the $\mtdirpar \msidepar$-side of $\mvpar$ }
        \State \Return $u > 0$
    \EndIf
\EndFunction
\end{algorithmic}
\end{algorithm}

%%%%%%%%%%%%%%%%%%%%%%%%%%%%%%%%% ALG: OCSECRULE  %%%%%%%%%%%%%%%%%%%%%%%%%%%%%%%%%%%%%
\clearpage
\subsection{\textproc{OcSecRule}: \textit{Checks if a Node can be Pruned}}
The function \textproc{OcSecRule} (Alg. \ref{suppalg:ocsecrule}) implements the occupied-sector rule.
The function returns immediately if the trace is outside the occupied-sector of parent node.
If the trace enters the occupied-sector for the source node, a recursive occupied-sector trace is generated, and the current trace is interrupted.

If the trace enters the occupied-sector of a target node that is $\mnoc$ type, the trace is discarded because the path has looped.
Otherwise, if the target is a non-$\mnoc$ node, a $\mnoc$ target-tree node is placed in the source-direction of the target node.
The placement can be considered part of a short recursive occupied-sector trace.

% Fig. \ref{suppfig:ocsecrule}
\begin{algorithm}[!ht]
\begin{algorithmic}[1]
\caption{\textproc{OcSecRule}: implements the occupied-sector rule.}
\label{suppalg:ocsecrule}
\Function{OcSecRule}{$\mtrace = (\mx_\mtrace, \mside_\mtrace, \cdots)$, $\mnlet = (\mtlink, \cdots) $}
    % \State $(\mtdirpar, \msidepar, \mnodepar, \mvpar, \mvprev, \sim) \gets $\Call{TraceCalc}{$\mtrace, \mnlet$}
    \State $\mnodepar \gets \fnode(\mtlink)$
    \State $\mtdirpar \gets \mnodepar\mdot\mtdirnode$ 
    \State $\msidepar \gets \mnodepar\mdot\msidenode$
    \State $\mvpar \gets \mxtrace - \fx(\mnodepar)$
    \State $\mvocpar \gets $ \Call{GetEdge}{$\fx(\mnodepar), -\mtdirpar\msidepar$}

    \Comment{(A) Parent is target $\mnoc$-node. Discard trace if it enters oc.sec., return otherwise.}
    \If {$\mnodepar \mdot \mntype = \mnoc$} 
        \Comment{Previously entered occupied-sector of a target-tree node (gpar. node)}
        \State $\mnodegpar \gets \fnode(\flink(T, \flink(T, \mtlink)))$ 
        \State $\mvgpar \gets \fx(\mnodepar) - \fx(\mnodegpar)$  
        \If {$\mside_\mpar (\mv_\mpar \times \mv_\mgpar) \le 0$}
            \Comment{Discard as path has looped around gpar. node and par. $\mnoc$ node} 
            \State \Call{EraseTree}{$T, \mtlink$} 
            \State Remove $\mnlet$ from  $\mtrace\mdot\mnlets_T$
        \EndIf
        \State \Return % $\mfalse$
    
    \Comment{(B) Return if not in occupied-sector.}
    \ElsIf{$\mtdirpar \mside_\mpar (\mv_\mpar \times \mvocpar) \le 0$} 
        \State \Return % $\mfalse$
        \Comment{Not in occupied-sector of $\mnode_\mpar$}
    \EndIf

    \Comment{(C) Create recursive oc-sec. trace if entered oc-sec. of source node.} 
    \If{$\mtdirpar = S$}
        \State $\mtrace_\mnew \gets $ \Call{CreateTrace}{$\fx(\mnodepar), \msidepar$}
        \State \Call{Anchor}{$\mtlink$, $\mtrace_\mnew\mdot\mnode_S$} 
        \State Move $\mnlet$ to $\mtrace_\mnew\mdot\mnlets_S$ \Comment{s.t. $\mtrace_\mnew\mdot\mnlets_S = \{\mnlet\}$ and $\mtrace\mdot\mnlets_S = \{\}$}
        \State $\mnlet\mdot\mvprog \gets \mvocpar$

        \State $\mnode_\mathrm{newTm} \gets$ \Call{GetNode}{$\mxtrace, \mntm, \msidetrace, T$}
        \Comment{Create a $\mntm$ target-tree node and re-anchor target trace-links there.}
        \State $\mtlink_\mathrm{newT} \gets $ \Call{CreateLink}{$\mtrace_\mnew\mdot\mnode_T$}
        \State \Call{CreateNodelet}{$\mtlink_\mathrm{newT}, -\mvpar, \mback, \mtrace_\mnew \mdot \mnlets_T$}

        \For{$\mnlet_T \in \mtrace\mdot\mnlets_T$} 
            \State $\mlink_\mathrm{newT} \gets \mnlet_T\mdot\mtlink$
            \State \Call{Anchor}{$\mlink_\mathrm{newT}$, $\mnode_\mathrm{newTm}$}
            \State $\mlink_\mathrm{newT}\mdot\mcost \gets$ \Call{Cost}{$\mlink_T$}
            \State \Call{Connect}{$T$, $\mtlink_\mathrm{newT}$, $\mlink_\mathrm{newT}$}
        \EndFor

        \State $\mtrace_\mnew\mdot\mxtrace \gets $ \Call{Trace}{$\mtrace_\mnew\mdot\mxtrace$, $\mtrace_\mnew\mdot\msidetrace$}
        \Comment{Start recursive trace from the $\msidepar$-side corner of the source node}
        \State \Call{Tracer}{$\mtrace_\mnew$} 

    \Comment{(D) Place target-tree $\mnoc$-node if entered oc-sec. of target node.} 
    \Else 
        \State $\mx_\mathrm{newOc} \gets $ \Call{Trace}{$\fx(\mnodepar)$, $-\msidepar$} 
        % \Comment{Get the $-\msidepar$ corner of the target node.}
        \State $\mnode_\mathrm{newOc} \gets$ \Call{GetNode}{$\mx_\mathrm{newOc}, \mnoc, \msidepar, T$} 
        % \Comment{Get $\mnoc$ target-tree node at $-\msidepar$ corner.}
        \State \Call{Anchor}{$\mtlink$, $\mnode_\mathrm{newOc}$} 
        % \Comment{Transfer expanded link to $\mnoc$ node.}
        \State $\mtlink\mdot\mcost \gets $ \Call{Cost}{$\mtlink$}
        \State $\mtlink_\mathrm{newT} \gets $ \Call{CreateLink}{$\mtrace\mdot\mtnode_T$}
        \State \Call{Connect}{$T, \mtlink_\mathrm{newT}, \mtlink$}
        \State $\mnlet\mdot\mtlink \gets \mtlink_\mathrm{newT}$
        \State $\mnlet\mdot\mvprog \gets \mvpar$
    \EndIf
\EndFunction
\end{algorithmic}
\end{algorithm}

%%%%%%%%%%%%%%%%%%%%%%%%%%%%%%%%% ALG: ANGSEC  %%%%%%%%%%%%%%%%%%%%%%%%%%%%%%%%%%%%%
\subsection{\textproc{AngSecRule}: \textit{Implements the Angular-sector Rule}}
The function \textproc{AngSecRule} (Alg. \ref{suppalg:angsecrule}) implements the angular-sector rule for the source node.

Four helper functions breaks the implementation down into smaller parts. They are \textproc{RayNotCrossed} (Alg. \ref{suppalg:raynotcrossed}), \textproc{AngSecPrune} (Alg. \ref{suppalg:angsecprune}), \textproc{Project} (Alg. \ref{suppalg:project}), and \textproc{RecurAngSecTrace} (Alg. \ref{suppalg:recurangsectrace}).
\textproc{AngSecRule} examines the $\msidetrace$-sided ray $\mray$ of the source node's angular sector, and determines if the trace is within the angular-sector.
If the trace is within the angular-sector, \textproc{AngSecRule} returns without calling the other helper functions.

The other helper functions are called when the trace exits the source node's angular sector.
\textproc{AngSecPrune} prunes the source node if the resulting path is not taut after exiting the source node's angular sector.
% The pruned source node is guaranteed to be $\mnvy$ type. 
% A prune by the angular-sector rule occurs only when the $\mray$ ends at the source node, indicating that the node is a source-tree node with cumulative visibility ($\mnvy$ or $\mney$ type). $\mney$-nodes are pruned by the pruning rule, as no recursive angular-sector trace can be generated for an $\mney$ node.
% $\mney$ node. A recursive angular-sector trace cannot occur for an $\mney$ node as the $\mney$ node cannot no longer be pruned by future queries.
If a prune by the angular-sector occurs, the current trace continues regardless of any subsequent recursive angular-sector trace.
\textproc{Project} (Alg. \ref{suppalg:project}) projects the ray $\mray$ and finds the projected ray's collision point.
\textproc{RecurAngSecTrace} generates a recursive angular-sector trace if the current trace did not pass through the projected ray's collision point.
% Fig. \ref{suppfig:angsecrule}.
\begin{algorithm}[!ht]
\begin{algorithmic}[1]
\caption{\textproc{AngSecRule}: implements the angular-sector rule.}
\label{suppalg:angsecrule}
\Function{AngSecRule}{$\mtrace = (\mxtrace, \msidetrace, \cdots)$, $\mnlet = (\mtlink, \cdots) $}
    \State $\mray \gets \fray(\msidetrace, \mtlink)$

    \If {\Call{RayNotCrossed}{$\mray, \mtrace, \mnlet$}}
        \State \Return $\mfalse$
    \EndIf
    \State \Call{AngSecPrune}{$\mray, \mtrace, \mnlet$}
    \State \Call{Project}{$\mray$}
    \State \Call{RecurAngSecTrace}{$\mray, \mtrace, \mnlet$}
    \State \Return $\mtrue$
    
\EndFunction
\end{algorithmic}
\end{algorithm}

%%%%%%%%%%%%%%%%%%%%%%%%%%%%% ALG:RAYNOTCROSSED %%%%%%%%%%%%%%%%%%%%%%%%%%%%%%%%%%%%
\subsubsection{\textproc{RayNotCrossed}: \textit{Checks if Trace is Within Angular-Sector}}
The function \textproc{RayNotCrossed} examines the $\msidetrace$-sided ray $\mray$ of the source node and compares the ray with the current position of the trace.
If the trace crosses the ray, the function returns $\mtrue$.

If the current position lies on the ray, it is not clear if the ray has been crossed. 
The function breaks ties by considering how the line-of-sight function \textproc{LOS} (Alg. \ref{suppalg:los}) returns the first corners after a collision. 
\textproc{LOS} relies on the directional vector bisecting the corner at the current position to place the first corners. 
The consideration is required because the first corners are subsequently checked in \textproc{RecurAngSecTrace} -- the ray can only be considered crossed if the $\msidetrace$-sided first corner lies at the current position.
However, the ray may not have been projected, and the algorithm can only check against the bisecting vector.

To eliminate errors resulting from floating point calculations, the algorithm is designed to handle only discrete, integer calculations. This helps the authors to verify proofs, and provides a foundation from which \rtwop{} can be improved.
The reader may choose to implement a much simpler intersection check that uses floating point calculations instead.

\begin{algorithm}[!ht]
\begin{algorithmic}[1]
\caption{\textproc{RayNotCrossed}: checks if a sector-ray is crossed.}
\label{suppalg:raynotcrossed}
\Function{RayNotCrossed}{$\mray, \mtrace = (\mxtrace, \msidetrace, \cdots)$, $\mnlet = (\mtlink, \cdots) $}
    \If {$\mray = \varnothing$} 
        \State \Return $\mtrue$
    \EndIf
    \State $\mvray \gets \mray\mdot\mx_T - \mray\mdot\mx_S$
    \State $\mlink_S \gets \flink(S, \mtlink)$ \Comment{$\mlink$ has only one source link.}
    \State $\mvpar \gets \mxtrace - \fx(\fnode(\mlink_S))$
    
    \State $u_\mathrm{ray,par} \gets \msidetrace (\mvray \times \mvpar)$
    \If{$u_\mathrm{ray,par} > 0$}
        \State \Return $\mtrue$
        \Comment{Return as ray is not crossed.}
    \ElsIf{$u_\mathrm{ray,par} = 0$} 
        \Comment{$\mvray$ and $\mvpar$ are parallel. Use bisecting oc-sec. vector to break ties.}
        \State $\mv_\mathrm{crn} \gets $ \Call{Bisect}{$\mxtrace$} 
        \State $u_\mathrm{ray,crn} \gets \msidetrace(\mvray \times \mv_\mathrm{crn})$ 
        \If {$u_\mathrm{ray,crn} > 0$ \Or $u_\mathrm{ray,crn} = 0$ \An $\mvray \sdot \mv_\mathrm{crn} > 0$} 
            \State \Return $\mtrue$
            \Comment{Ray is not crossed: $\mvray$ lies strictly to the $\msidetrace$-side of $\mv_\mathrm{crn}$, or...}
        \EndIf
        \Comment{...ray points away from corner: $\mvray$ opposite to $\mv_\mathrm{crn}$.}
    \EndIf 
    \State \Return $\mfalse$.
\EndFunction
\end{algorithmic}
\end{algorithm}

%%%%%%%%%%%%%%%%%%%%%%%%%%%%% ALG:ANGSECPRUNE %%%%%%%%%%%%%%%%%%%%%%%%%%%%%%%%%%%%
\subsubsection{\textproc{AngSecPrune}: \textit{Tries to Prune Source Node}}
The function \textproc{AngSecPrune} (Alg. \ref{suppalg:angsecprune}) tries to prune the source node if the resulting path is not taut after exiting the node's angular sector.
If the node cannot be pruned, nothing is done.
When a prune occurs, the current trace continues regardless of a subsequent recursive angular-sector trace.

The pruned source node is guaranteed to be $\mnvy$ type. 
A prune by the angular-sector rule occurs only when the $\mray$ ends at the source node, indicating that the node is a source-tree node with cumulative visibility ($\mnvy$ or $\mney$ type). $\mney$-nodes are pruned by the pruning rule, as no recursive angular-sector trace can be generated for an $\mney$ node.
$\mney$ node. A recursive angular-sector trace cannot occur for an $\mney$ node as the $\mney$ node can no longer be pruned by future queries.
\begin{algorithm}[!ht]
\begin{algorithmic}[1]
\caption{\textproc{AngSecPrune}: tries to prune a trace's source node after exiting the node's angular-sector.}
\label{suppalg:angsecprune}
\Function{AngSecPrune}{$\mray, \mtrace = (\mxtrace, \msidetrace, \cdots)$, $\mnlet = (\mtlink, \cdots) $}
    \State $\mlink_S \gets \flink(S, \mtlink)$
    \State $\mnode_S \gets \fnode(\mlink_S)$
    
    \State $prunable \gets \mray\mdot\mx_T = \fx(\mnode_S)$ \Comment{Prunable if sector-ray ends at parent source-tree node, or...}
    \State $prunable \gets prunable $ \Or ($\mray\mdot\mx_T = \mxstart$ \An $\mray\mdot\mx_S = \mxgoal$ \An $\msidetrace = \mnode_S\mdot\msidenode$) \Comment{...prunable if ray is special sector-ray for start node and the side traced is same as start node's side.}
    \If {$prunable$} 
        \State $\mtlink_\mathrm{newS} \gets $ \Call{Isolate}{$T, \mlink_S, \varnothing, \mtrace, \mtrace\mdot\mtnode_S$}
        \State $\mnode_\mathrm{newS} \gets \fnode(\flink(S, \mtlink_\mathrm{newS}))$
        \State \Call{CreateNodelet}{$\mtlink_\mathrm{newS}, \mxtrace - \fx(\mnode_\mathrm{newS}), \mback, \mtrace\mdot\mnlets_S$}
    \EndIf
\EndFunction
\end{algorithmic}
\end{algorithm}

%%%%%%%%%%%%%%%%%%%%%%%%%%%%% ALG:ANGSECPRUNE %%%%%%%%%%%%%%%%%%%%%%%%%%%%%%%%%%%%
\subsubsection{\textproc{RecurAngSecTrace}: \textit{Tries to Generate a Recursive Angular-sector Trace}}
The function \textproc{RecurAngSecTrace} generates a recursive angular-sector trace if the trace crosses the collision point of the projected ray $\mray$.
The trace crosses the collision point if the current position $\mxtrace$ lies on the first $\msidetrace$-sided  corner from the collision point.

A $(-\msidetrace)$-sided $\mnun$ node is placed at the first $\msidetrace$-side corner from the collision point. The node ensures that the $(-\msidetrace)$-sided recursive trace progresses with respect to a target node at the initial corner traced.
The $\mnun$ node will be pruned at the initial corner if the resulting path is not taut.
A $\mntm$ node is placed at the current trace location, and is the target node of the $\mnun$ node.
Additionally the $\mnun$ node is unreachable because if a query from the recursive trace reaches the node, a cheaper path has to exist that can reach the $\mntm$ node.

% Fig. \ref{suppfig:recurangsectrace}
\begin{algorithm}[!ht]
\begin{algorithmic}[1]
\caption{\textproc{RecurAngSecTrace}: performs a recursive angular-sector trace if required.}
\label{suppalg:recurangsectrace}
\Function{RecurAngSecTrace}{$\mray, \mtrace = (\mxtrace, \msidetrace, \cdots)$, $\mnlet = (\mtlink, \cdots) $}
    \State $\mnode_S \gets \fnode(\flink(S, \mtlink))$
    \If {$\fxcol(\msidetrace, \mray) = \mxtrace$ \Or $\mnodepar\mdot\mntype = \mney$}
    \Comment{Discard if trace crossed the collision point of the sector-ray, or...}
        \State \Call{EraseTree}{$S, \mtlink$}
        \Comment{...parent source-tree node is $\mney$ (recur. trace has different side from $\mney$ node).}
        \State Remove $\mnlet$ from $\mtrace\mdot\mnlets_S$
    \Else   
        \Comment{Trace did not cross sector-ray's collision point. Recursive ang-sec. trace.}
        \State $\mtrace_\mnew \gets $ \Call{CreateTrace}{$\fxcol(-\msidetrace, \mray), -\msidetrace$}
        \State $\mnlet\mdot\mvprog \gets \mtrace_\mnew\mdot\mxtrace - \fx(\mnode_S)$
        
        \State $\mx_\mathrm{newUn} \gets \fxcol(\msidetrace, \mray)$ 
        \Comment{Create a $\mnun$ target-tree node at $\msidetrace$ corner of collision.}
        \If {$\mx_\mathrm{newUn} = \fxcol(-\msidetrace, \mray)$} 
            \Comment{Collision at corner instead of edge.}
            \State $\mx_\mathrm{newUn} \gets $ \Call{Trace}{$\mx_\mathrm{newUn}, \msidetrace$}
        \EndIf
        \State $\mnode_\mathrm{newUn} \gets $ \Call{GetNode}{$\mx_\mathrm{newUn}, \mnun, -\msidetrace, T$}
        \State $\mlink_\mathrm{newT} \gets $ \Call{CreateLink}{$\mnode_\mathrm{newUn}$}
        
        \State $\mnode_\mathrm{newTm} \gets$ \Call{GetNode}{$\mxtrace, \mntm, \msidetrace, T$} 
        \Comment{Create a $\mntm$ target-tree node at current corner at $\mxtrace$}
        \For {$\mnlet_T \in \mtrace\mdot\mnlets_T$}
            \State $\mlink_\mathrm{newTT} \gets $ \Call{CopyLink}{$\mnlet_T\mdot\mtlink, \mnode_\mathrm{newTm}, \{T\}$} 
             \Comment{Re-anchor target trace-links from current trace at $\mntm$ node.}
            \State $\mlink_\mathrm{newTT}\mdot\mcost \gets$ \Call{Cost}{$\mlink_\mathrm{newTT}$}
            \State \Call{Connect}{$T$, $\mlink_\mathrm{newT}, \mlink_\mathrm{newTT}$}
        \EndFor
        \State $\mlink_\mathrm{newT}\mdot\mcost \gets$ \Call{Cost}{$\mlink_\mathrm{newT}$}

        \State $\mtlink_\mathrm{newT} \gets $ \Call{CreateLink}{$\mtrace_\mnew\mdot\mtnode_T$} 
        \State \Call{Connect}{$T, \mtlink_\mathrm{newT}, \mlink_\mathrm{newT}$}
        \State \Call{CreateNodelet}{$\mtlink_\mathrm{newT}, \mtrace_\mnew\mdot\mxtrace - \mx_\mathrm{newUn}, \mfront, \mtrace_\mnew\mdot\mnlets_T$}

        \State \Call{Tracer}{$\mtrace_\mnew$}
    \EndIf
\EndFunction
\end{algorithmic}
\end{algorithm}

%%%%%%%%%%%%%%%%%%%%%%%%%%%%%%%%% ALG: INTERRUPT RULE  %%%%%%%%%%%%%%%%%%%%%%%%%%%%%%%%%%%%%
\clearpage
\subsection{Interrupt Rule} \label{suppsec:interrupt}
Function \textproc{InterruptRule} (Alg. \ref{suppalg:interrupt}) implements the interrupt rule, which interrupts and queues a trace when a number of corners are traced and if the trace is progressed with respect to all source-tree and target-tree parent nodes.

The number of corners to interrupt $numInterrupt$ is arbitrary. 
The larger $numInterrupt$ is, the slower \rtwop{} may get for simple queries with few turning points as the tracing queries spend more time on non-convex contours. 
The smaller $numInterrupt$ is, the slower \rtwop{} may be for more complex queries with many turning points due to frequent open-list queuing. The default value is $numInterrupt = 10$.
\begin{algorithm}[!ht]
\begin{algorithmic}[1]
\caption{\textproc{InterruptRule}: implements the interrupt rule.}
\label{suppalg:interrupt}
\Function{InterruptRule}{$\mtrace = (\mxtrace, \msidetrace, \cdots)$}
    
    \Comment{(A) Return if trace has only checked a few corners, and trace is not prog. w.r.t. all nodes.}
    \State $allProgS \gets $ $\mnlet_S \mdot \mcprog = 0 $ for all $ \mnlet_S \in \mtrace\mdot\mnlets_S$
    \State $allProgT \gets $ $\mnlet_T \mdot \mcprog = 0 $ for all $ \mnlet_T \in \mtrace\mdot\mnlets_T$
    \If{$\mtrace\mdot\mnumcrns < numInterrupt$ \Or $allProgS = \mfalse$ \Or $allProgT = \mfalse$}
        \State \Return $\mfalse$
    \EndIf

    \Comment{(B) Otherwise, interrupt and create nodes and re-anchor trace-links.}
    \State $\mnode_\mathrm{newSVu} \gets$ \Call{GetNode}{$\mxtrace, \mnvu, \msidetrace, S$}
    \State $\mlink_\mathrm{newS} \gets$ $\fnlet(S, \mtrace)\mdot\mtlink$ 
    \State \Call{Anchor}{$\mlink_\mathrm{newS}, \mnode_\mathrm{newSVu}$}
    \State $\mlink_\mathrm{newS}\mdot\mcost \gets$ \Call{Cost}{$\mlink_\mathrm{newS}$}
    
    \State $\mnode_\mathrm{newTTm} \gets$ \Call{GetNode}{$\mxtrace, \mntm, \msidetrace, T$}
    \For{$\mnlet_T \in \mtrace\mdot\mnlets_T$}
        \State $\mlink_\mathrm{newT} \gets \mnlet_T\mdot\mtlink$
        \State \Call{Anchor}{$\mlink_\mathrm{newT}, \mnode_\mathrm{newTTm}$}
        \State $\mlink_\mathrm{newT}\mdot\mcost \gets$ \Call{Cost}{$\mlink_\mathrm{newT}$}
        \State \Call{Connect}{$T, \mlink_\mathrm{newS}, \mlink_\mathrm{newT}$}
    \EndFor

    \Comment{(C) Mark for overlap-rule check, or queue a tracing query}
    \If {$\mtrace\mdot\moverlap = \mtrue$}
        \State \Call{PushOverlap}{\Call{GetPos}($\mxtrace$)}
    \Else
        \State $f \gets \mlink_\mathrm{newS}\mdot\mcost + $ \Call{GetMinCost}{$T, \mlink_\mathrm{newS}$}
        \State \Call{Queue}{$\mqtrace, f, \mlink_\mathrm{newS} $}
    \EndIf
    \State \Return $\mtrue$
\EndFunction
\end{algorithmic}
\end{algorithm}

%%%%%%%%%%%%%%%%%%%%%%%%%%%%%%%%% ALG: PLACERULE  %%%%%%%%%%%%%%%%%%%%%%%%%%%%%%%%%%%%%
\clearpage
\subsection{\textproc{PlaceRule}: Places Points and Checks Castability}
\textproc{PlaceRule} implements the placement rule and tries to place a turning point or phantom point.
The function exits after a phantom point is placed, or if no point can be placed.

If a turning point is placed, the function examines if the trace has crossed a path from a different query.
If a different path is crossed, the overlap rule will check the placed links after the trace ends.
The trace will end with the placement rule if all target nodes can be cast to.
% If there are other links, the trace has crossed a the trace is marked for an overlap-rule check that engages after all target nodes become castable.
% The rule subsequently tries to cast to each target node, queuing a casting query for each castable node.

The function is aided by four helper functions, \textproc{IsRev} (Alg. \ref{suppalg:isrev}), \textproc{IsVis} (Alg. \ref{suppalg:isvis}), \textproc{PlaceNode} (Alg. \ref{suppalg:placenode}), and \textproc{CastFromTrace} (Alg. \ref{suppalg:castfromtrace}).

\begin{algorithm}[!ht]
\begin{algorithmic}[1]
\caption{\textproc{PlaceRule}: implements the placement rule and queues a cast if needed.}
\label{suppalg:placerule}
\Function{PlaceRule}{$\mtrace = (\mxtrace, \msidetrace, \cdots)$}
    \State $\mtdirpar \gets S$ if corner at $\mxtrace$ is convex, $T$ otherwise

    \State $\mnlet_\mnew \gets $ \Call{PlaceNode}{$\mtdirpar, \mtrace$}

    \If {$\mnlet_\mnew = \varnothing$ \Or $\mtdirpar = T$}
        \State \Return $\mfalse$
        \Comment{Turning point not placed. Nothing else to do.}
    \ElsIf {$\sum \lvert \mnode\mdot\mlinks_\mnode \rvert > 1$ for all $\mnode \in $ \Call{GetPos}{$\mxtrace$}$\mdot\mnodes$ }
        \State $\mtrace\mdot\moverlap \gets \mtrue$
        \Comment{Mark for overlap rule if multiple links are anchored at $\mxtrace$.}
    \EndIf

    \If {$\mnlet_\mnew \ne \varnothing$ \An $\mtdirpar = S$}
        \Comment{Try casting if a turning point is placed.}
        \State \Call{CastFromTrace}{$\mtrace, \mnlet_\mnew$}
    \EndIf

    \State \Return $\mtrace\mdot\mnlets_T = \{\}$ 
    \Comment{Return $\mtrue$ if no more target trace-nodes.}
\EndFunction
\end{algorithmic}
\end{algorithm}

%%%%%%%%%%%%%%%%%%%%%%%%%%%%%%%%% ALG: ISREV  %%%%%%%%%%%%%%%%%%%%%%%%%%%%%%%%%%%%%
\subsubsection{\textproc{IsRev}: \textit{Checks if Angular Progression Will Reverse}}
The helper function \textproc{IsRev} (Alg.\ref{suppalg:isrev}) returns $\mtrue$ if tracing the next edge from the current corner at $\mxtrace$ causes the angular progression to reverse with respect to the parent node.
\begin{algorithm}[!ht]
\begin{algorithmic}[1]
\caption{\textproc{IsRev}: checks if a trace's angular progression will reverse at the next edge of a corner.}
\label{suppalg:isrev}
\Function{IsRev}{$\mtdirpar, \msidetrace, \mvpar, \mvnext$}
    \State \Return $\mtdirpar \msidetrace (\mvpar \times \mvnext) < 0$
\EndFunction
\end{algorithmic}
\end{algorithm}

%%%%%%%%%%%%%%%%%%%%%%%%%%%%%%%%% ALG: ISVIS %%%%%%%%%%%%%%%%%%%%%%%%%%%%%%%%%%%%%
\subsubsection{\textproc{IsVis}: \textit{Checks if a Target Node is Castable}}
The helper function \textproc{IsVis} (Alg. \ref{suppalg:isvis}) returns $\mtrue$ if a target-tree node is potentially visible from the traced position and can be cast to.
\begin{algorithm}[!ht]
\begin{algorithmic}[1]
\caption{\textproc{IsVis}: checks if a target node is potentially visible.}
\label{suppalg:isvis}
\Function{IsVis}{$\msidetrace, \mvpar, \mvnext$}  
    \Comment{Par. node is target-tree node.}
    \State \Return $\msidetrace (\mvpar \times \mvnext) \le 0$ \Comment{Assumes that trace has progressed w.r.t. target-tree node.}
\EndFunction
\end{algorithmic}
\end{algorithm}

%%%%%%%%%%%%%%%%%%%%%%%%%%%%%%%%% ALG: PLACENODE  %%%%%%%%%%%%%%%%%%%%%%%%%%%%%%%%%%%%%
\subsubsection{\textproc{PlaceNode}: \textit{Tries to Place a Node}}
The helper function \textproc{PlaceNode} (Alg. \ref{suppalg:placenode}) tries to place a turning point or phantom point.
A turning point ($\mnvu$ or $\mneu$-node) is placed if the current corner is convex, and the angular progression will reverse with respect to the source node.
A phantom point ($\mntm$-node) is placed if the current corner is non-convex, and the angular progression reverses with respect to at least one target node.
\begin{algorithm}[!ht]
\begin{algorithmic}[1]
\caption{\textproc{PlaceNode}: places a $\mntm$, $\mnvu$ or $\mneu$ node if possible.}
\label{suppalg:placenode}
\Function{PlaceNode}{$\mtdirpar, \mtrace = (\mxtrace, \msidetrace, \cdots)$}
    \State $\mvnext \gets $ \Call{GetEdge}{$\mxtrace, \msidetrace$}
    \State $\mnlet_\mnew = \varnothing$
    \For{$\mnlet \in \fnlets(\mtdirpar, \mtrace)$}
        % \State $(\sim, \sim, \mnodepar, \mvpar, \sim, \mvnext) \gets $\Call{TraceCalc}{$\mtrace, \mnlet$}
        \State $\mnodepar \gets \flink(\mnlet\mdot\mtlink)$
        \State $\mvpar \gets \mxtrace - \fx(\mnodepar)$
        
        \Comment{(A) Do not place if not prog. w.r.t. par. node, or ang. prog. increases at next edge.}
        \If {$\mcprog > 0$ \Or \Call{IsRev}{$\mtdirpar, \msidetrace, \mvpar, \mvnext$} = $\mfalse$}
            \State \Continue
        \EndIf

        \Comment{(B) Otherwise, place a new phantom ($\mntm$) or turning point ($\mneu$ or $\mnvu$).}
        \State $\mlink_\mathrm{newPar} \gets \mnlet\mdot\mtlink$
        \If {$\mnlet_\mnew = \varnothing$}
            \Comment{Create the new node and reuse current nodelet if new node not yet placed.}
            \State $\mnlet_\mnew \gets \mnlet$
            \State $\mntype_\mathrm{newPar} \gets \mnvu$
            \Comment{Determine the new node type.}
            \If {$\mtdirpar = T$}
                \State $\mntype_\mathrm{newPar} \gets \mntm$
            \ElsIf{$\mnodepar\mdot\mntype \in \{\mneu, \mney\}$}
                \State $\mntype_\mathrm{newPar} \gets \mneu$
            \EndIf
            \Comment{Create the new node and reuse current nodelet.}
            \State $\mnode_\mathrm{newPar} \gets $ \Call{GetNode}{$\mxtrace, \mntype_\mathrm{newPar}, \msidetrace, \mtdirpar$}
            \State $\mnlet_\mnew\mdot\mtlink \gets$ \Call{CreateLink}{$\ftnode(\mtdirpar, \mtrace)$}
            \State $\mnlet_\mnew\mdot\mvprog \gets \mvnext$
        \Else
            \Comment{Delete the nodelet if new node has been placed.}
            \State Remove $\mnlet$ from $\fnlets(\mtdirpar, \mtrace)$
        \EndIf

        \State \Call{Anchor}{$\mlink_\mathrm{newPar}, \mnode_\mathrm{newPar}$}
        \State $\mlink_\mathrm{newPar}\mdot c \gets$ \Call{Cost}{$\mlink_\mathrm{newPar}$}
        \State \Call{Connect}{$\mtdirpar, \mnlet_\mnew\mdot\mtlink, \mlink_\mathrm{newPar}$}
    \EndFor
    \State \Return $\mnlet_\mnew$
\EndFunction
\end{algorithmic}
\end{algorithm}

%%%%%%%%%%%%%%%%%%%%%%%%%%%%%%%%% ALG: CastFromTrace  %%%%%%%%%%%%%%%%%%%%%%%%%%%%%%%%%%%%%
\subsubsection{\textproc{CastFromTrace}: \textit{Tries to Cast From a Placed Turning Point.}}
The helper function \textproc{CastFromTrace} tries to cast to each target node after a turning point is placed at the current corner.
If castable, a casting query is queued for each target trace-link. The target trace-link is re-anchored on a target-tree $\mnvu$ node.
However, if the trace had crossed a path from a different query, it would have been marked for an overlap-rule check in \textproc{PlaceRule} (Alg. \ref{suppalg:placerule}). 
No new casting queries are queued by the trace, as the overlap-rule will queue a new casting query in the most recent source-tree node with cumulative visibility.
\begin{algorithm}[!ht]
\begin{algorithmic}[1]
\caption{\textproc{CastFromTrace}: tries to cast to all target nodes after placing a turning point.}
\label{suppalg:castfromtrace}
\Function{CastFromTrace}{$\mtrace=(\mxtrace, \msidetrace, \cdots), \mnlet_\mnew$}
    \State $\mvnext \gets $ \Call{GetEdge}{$\mxtrace, \msidetrace$}
    \State $\mlink_S \gets \flink(S, \mnlet_\mnew\mdot\mtlink)$
    \State $\mnode_S \gets \mnode(\mlink_S)$  
    \State $\mnode_\mathrm{newVu} \gets \varnothing$
    \For {$\mnlet_T \in \mtrace\mdot\mnlets_T$}

        \Comment{(A) For each target node, check if it is castable from new turning point at $\mx$.}
        % \State $(\sim, \sim, \mnodepar, \mvpar, \sim, \mvnext) \gets $\Call{TraceCalc}{$\mtrace, \mnlet_T$}
        \State $\mlink_\mathrm{newT} \gets \mnlet_T\mdot\mtlink$
        \State $\mnode_T \gets \fnode(\flink(T, \mlink_\mathrm{newT}))$
        \State $\mvpar \gets \mxtrace - \fx(\mnode_T)$
        % \If{$\mnlet_T\mdot\mcprog > 0$ \Or $\mnode_T\mdot\mntype = \mnph$ \Or \Call{IsVis}{$\msidetrace, \mvpar, \mvnext$} $= \mfalse$}
        %     \State \Continue 
        %     \Comment{Ignore target-tree node if not prog. w.r.t. node, node is $\mnph$, or node is not visible.}
        % \EndIf
        \If {\Call{IsVis}{$\msidetrace, \mvpar, \mvnext$} $= \mfalse$}
            \State \Continue 
            \Comment{Skip non-castable tgt node.}
        \EndIf
        
        \Comment{(B) Target node is castable, re-anchor target trace-link to target-tree $\mnvu$ node.}
        \If {$\mnode_\mathrm{newVu} = \varnothing$}
            \State $\mnode_\mathrm{newVu} \gets $ \Call{GetNode}{$\mxtrace, \mnvu, \msidetrace, T$}
        \EndIf
        \State \Call{Anchor}{$\mlink_\mathrm{newT}, \mnode_\mathrm{newVu}$}
        \State $\mlink_\mathrm{newT}\mdot\mcost \gets $ \Call{Cost}{$\mlink_\mathrm{newT}$}
        \State \Call{Connect}{$T, \mlink_S, \mlink_\mathrm{newT}$}

        \Comment{(C.1) Mark for overlap-rule if source node is expensive or trace crossed paths with other queries.}
        \If {$\mtrace\mdot\moverlap = \mtrue$ \Or $\mnode_S\mdot\mntype = \mneu$}
            \State $\mtrace\mdot\moverlap \gets \mfalse$
            \State \Call{PushOverlap}{\textproc{GetPos}($\mxtrace$)}
        
        \Comment{(C.2) Otherwise, queue a casting query.}
        \Else
            \State $f \gets \mlink_S\mdot\mcost + \mlink_\mathrm{newT}\mdot\mcost$ 
            \State \Call{Queue}{$\mqcast, f, \mlink_T'$}
        \EndIf
        \State Remove $\mnlet_T$ from $\mtrace\mdot\mnlets_T$
    \EndFor
\EndFunction

\end{algorithmic}
\end{algorithm}

\section{Overlap Rule} \label{suppsec:overlap}
\setcounter{algorithm}{0}

The overlap rule reduces the number of queries by verifying line-of-sight and cost-to-come for nodes in overlapping paths.

The overlap rule consists of two major components implemented by the functions \textproc{ShrinkSourceTree} (Alg. \ref{suppalg:shrinksourcetree}) and \textproc{ConvToExBranch} (Alg. \ref{suppalg:convtoexbranch}). 
Both components that allow \rtwop{} to identify and discard some expensive queries. 
The \textproc{ShrinkSourceTree} function shifts overlapping queries from the leaf nodes to the first source-tree node with cumulative visibility ($\mney$ or $\mnvy$ node), shrinking the source-tree and expanding the target-tree in the process. 
By shifting the queries, \textproc{ShrinkSourceTree} allow \rtwop{} to verify the cost-to-come of overlapping nodes.
The \textproc{ConvToExBranch} (Alg. \ref{suppalg:convtoexbranch}) marks existing nodes at a location $\mx$ as expensive when a cast reaches $\mx$ with a shorter path than the existing paths.

% processes overlapping queries after a queued query is processed (Alg. \ref{suppalg:run}).

% Fig. \ref{suppfig:overlaprule}

%%%%%%%%%%%%%%%%%%%%%%%%%%%%%%%%% ALG: SHRINKSOURCETREE  %%%%%%%%%%%%%%%%%%%%%%%%%%%%%%%%%%%%%
\subsection{\textproc{ShrinkSourceTree}: \textit{Shifts Queries to Verify Cost-to-come}} 
The \textproc{ShrinkSourceTree} function (Alg. \ref{suppalg:shrinksourcetree}) shifts overlapping queries to a source-tree node along their path, simultaneously shrinking the source-tree and expanding the target-tree. 
The source-tree node is a $\mnvy$ or $\mney$ node that is furthest along the examined path from the start node.
Let $\mnode_\mathrm{SY}$ represent the source-tree $\mnvy$ or $\mney$ node.

Overlaps are identified in a trace or reached cast. 
In a trace, overlaps are identified when a turning point ($\mneu$ or $\mnvu$ node) is placed. 
If the corner at the turning point contain nodes that anchor other links, an overlap is identified (see \textproc{PlaceNode}, Alg. \ref{suppalg:placenode}). 
Likewise, in a reached cast, an overlap is identified at the source or target node if there are other links at the node's corner (see \textproc{FinishReachedCast}, Alg. \ref{suppalg:finishreachedcast}).
Once overlaps are identified, the corners where the overlaps occur are pushed in to the overlap-buffer.
They corners are subsequently processed by \textproc{ShrinkSourceTree} at the end of an iteration in \textproc{Run} (Alg. \ref{suppalg:run}).

The reader may notice that the corner pushed into the overlap-buffer for the tracing query may not be the point where overlap occurs (see \textproc{TryCastingFromTrace}, Alg. \ref{suppalg:castfromtrace}). 
While this may cause some overlapping queries to be missed, this reduces the size of the overlap buffer, and subsequent casts will still identify the missed queries.
For simplicity, the reader may choose to push the corner directly into the overlap-buffer in \textproc{PlaceNode} instead.

For each corner in the overlap-buffer, \textproc{ShrinkSourceTree} identifies source-tree $\mneu$ and $\mnvu$ nodes.
For each link anchored at the nodes, the path in the source direction is searched, and $\mnode_\mathrm{SY}$ is identified.
The function \textproc{ConvToTgtBranch} is called from the $\mnode_\mathrm{SY}$, converting all source-tree nodes in the target direction of $\mnode_\mathrm{SY}$ to target-tree $\mnvu$ nodes.
Any query in the target links are removed.
A casting query is subsequently queued from the $\mnode_\mathrm{SY}$ node.
\begin{algorithm}[!ht]
\begin{algorithmic}[1]
\caption{\textproc{ShrinkSourceTree}: process overlapping queries by shrinking the source-tree and requeuing at a $\mnvy$ $S$-tree node.}
\label{suppalg:shrinksourcetree}
\Function{ShrinkSourceTree}{\null}
    \For {$\mpos \in $ overlap-buffer}
        \For {$\mnode \in \mpos\mdot\mnodes$}
            \If {$\mnode\mdot\mtdirnode = T$ \Or $\mnode\mdot\mntype \notin \{\mneu, \mnvu\}$}
                \State \Continue
            \EndIf
            \For {$\mlink \in \mnode\mdot\mlinks_\mnode$}
                \State $\mlink_i \gets \mlink$
                \State $\mlink_{SY} \gets \flink(\mlink_i)$
                \While {$\fnode(\mlink_S)\mdot\mntype \notin \{\mnvy, \mney\}$}
                    \State $\mlink_i \gets \mlink_S$
                    \State $\mlink_{SY} \gets \flink(S, \mlink_{SY})$
                \EndWhile
                \State \Call{ConvToTgtBranch}{$\mlink_i$}
                \State \Call{Queue}{$\mqcast, \mlink_{SY}\mdot\mcost + \mlink_i\mdot\mcost, \mlink_i$}
            \EndFor
        \EndFor
    \EndFor
\EndFunction
\end{algorithmic}
\end{algorithm}

%%%%%%%%%%%%%%%%%%%%%%%%%%%%%%%%%%%%%%%%%% ALG: CONVTOTGTBRANCH %%%%%%%%%%%%%%%%%%%%%%%%%%%%%%%%%%
\subsection{\textproc{ConvToTgtBranch}: \textit{Converts Source-tree Nodes to Target-tree Nodes}} 
The function \textproc{ConvToTgtBranch} (Alg. \ref{suppalg:convtotgtbranch}) converts source-tree nodes to target-tree $\mnvu$ nodes, re-anchoring links in the process.
It is an auxiliary recursive function of \textproc{ShrinkSourceTree} (Alg. \ref{suppalg:shrinksourcetree}).
If a query is found at a leaf node, the query is removed to avoid data races with the new casting query in \textproc{ShrinkSourceTree}.
\begin{algorithm}[!ht]
\begin{algorithmic}[1]
\caption{\textproc{ConvToTgtBranch}: converts source-tree branches to target-tree branches.}
\label{suppalg:convtotgtbranch}
\Function{ConvToTgtBranch}{$\mlink$}
    \If {$\fquery(\mlink) \ne \varnothing$}
        \State \Call{Unqueue}{$\fquery(\mlink)$}
        \Comment{Unqueue and remove any query on leaf links to avoid data races.}
    \EndIf
    \If {$\fnode(\mlink)\mdot\mtdirnode = T$}
        \State \Return
        \Comment{Reached leaf node of target-tree.}
    \EndIf
    \For{$\mlink_T \in \mlink\mdot\mlinks_T$}
        \State \Call{ConvToTgtBranch}{$\mlink_T, \fnode(\mlink)$}
    \EndFor

    \State $\mnode_S \gets \fnode(\flink(S, \mlink))$
    \State $\mnode_\mnew \gets $ \Call{GetNode}{$\fx(\mnode_S), \mnvu, \mnode_S\mdot\msidenode, T$}
    \State \Call{Anchor}{$\mlink, \mnode_\mnew$}
    \State $\mlink\mdot\mcost \gets$ \Call{Cost}{$\mlink$}
\EndFunction
\end{algorithmic}
\end{algorithm}

%%%%%%%%%%%%%%%%%%%%%%%%%%%%%%%%%%%%%%%%%% ALG: CONVTOEXBRANCH %%%%%%%%%%%%%%%%%%%%%%%%%%
\subsection{\textproc{ConvToExBranch}: \textit{Identify Expensive Nodes After a Reached Cast.}}
The function \textproc{ConvToExBranch} converts existing nodes to expensive nodes when a reached cast finds a shorter path than other paths at a corner. 
The corner is represented by the Position object ($\mpos$).

The function is called by a reached cast when reaching a node results in the shortest path so far (see \textproc{SingleCumulativeVisibility} Alg. \ref{suppalg:singlecumulativevisibility}).
When $\mtdir = S$, $\mpos$ describes the corner at the target node, and cost-to-come is examined at the target node.
When $\mtdir = T$, $\mpos$ describes the corner at the source node, and the examined cost is cost-to-go is examined at the source node.
Links anchored on the existing $\mtdir$-tree $\mnvy$ node are identified, and connected $-\mtdir$ direction links are re-anchored on expensive nodes.
The function relies on the auxiliary recursive function \textproc{ConvToExBranchAux} to perform the conversion.
Expensive paths that are guaranteed to cross the current shortest path will be discarded.

\begin{algorithm}[!ht]
\begin{algorithmic}[1]
\caption{\textproc{ConvToExBranch}: converts a branch of $\mtdir$-tree $\mnvy$ nodes to $\mney$ nodes.}
\label{suppalg:convtoexbranch}
\Function{ConvToExBranch}{$\mtdir, \mpos$}
    \For {$\mnode \in \mpos\mdot\mnodes$}
        \If {$\mnode\mdot\mntype \ne \mnvy$ \Or $\mnode\mdot\mtdirnode \ne \mtdir$}
            \State \Continue 
            \Comment{ Check only $L$ or $R$-sided $\mtdir$-tree $\mnvy$ node/}
        \EndIf

        \State $\mbest \gets \fbest(\mtdir, \mpos)$
        \State $\mside_\mbest \gets \mbest\mdot\mnode_\mbest\mdot\msidenode$ 
        \State $\mv_\mbest \gets \mpos\mdot\mx - \mbest\mdot\mxbest$
        \For {$\mlink \in \mnode\mdot\mlinks_\mnode$}
            \State $\mlinkpar \gets \flink(\mtdir, \mlink)$
            \State $\mnodepar \gets \fnode(\mlinkpar)$
            \State $\mvpar \gets \mpos\mdot\mx - \fx(\mnodepar)$
            
            \If {$\mnode\mdot\msidenode = \mside_\mbest$ \An $\mtdir \mside_\mbest(\mv_\mbest \times \mvpar) > 0$}
            \Comment{Discard ex. path from $\mlink$ if it will cross the shortest path.}
                \State \Call{Disconnect}{$\mtdir, \mlink, \mlinkpar$}
                \State \Call{EraseTree}{$-\mtdir, \mlink$}
            \Else
                \State \Call{ConvToExBranchAux}{$\mtdir, \mlinkpar, \mlink, \mnode\mdot\msidenode$}
            \EndIf
            \State \Call{EraseTree}{$\mtdir, \mlinkpar$}
            \Comment{Discard $\mlinkpar$ if no more $(-\mtdir)$-links.} 
        \EndFor
    \EndFor
\EndFunction
\end{algorithmic}
\end{algorithm}

%%%%%%%%%%%%%%%%%%%%%%%%%%%%%%%%%%%%%%%%%% ALG: CONVTOEXBRANCH %%%%%%%%%%%%%%%%%%%%%%%%%%
\subsection{\textproc{ConvToExBranchAux}: \textit{Create Expensive Nodes and Discard Expensive Paths}}
The function \textproc{ConvToExBranchAux} (Alg. \ref{suppalg:convtoexbranch}) converts $\mtdir$-tree $\mnvy$ nodes to $\mney$ nodes and reanchors links to the $\mney$ nodes.
It is the auxiliary recursive function for \textproc{ConvToExBranch} (Alg. \ref{suppalg:convtoexbranch}).

\textproc{ConvToExBranchAux} discards expensive paths if they will remain expensive in subsequent queries.
The function stops once a node that is not $\mnvy$ and not in the $\mtdir$-tree is reached.
If the reached node is a source-tree $\mnvu$ node, the function \textproc{ConvToTgtBranch} (Alg. \ref{suppalg:convtotgtbranch}) is used to shift queries to the most recent $\mney$-node to verify cost-to-come.

\begin{algorithm}[!ht]
\begin{algorithmic}[1]
\caption{ConvToExBranchAux: converts $\mnvy$ nodes to $\mney$ nodes and discards paths that will be expensive.}
\label{suppalg:convtoexbranchaux}
\Function{ConvToExBranchAux}{$\mtdir, \mlinkpar, \mlink, \mside$}
    \State $\mnode \gets \fnode(\mlink)$

    \Comment{(A) Discard if par. node and current $\mnvy$ or $\mney$ node have different sides.}
    \If {$\mnode\mdot\msidenode \ne \mside$ \An $\mnode\mdot\mntype \in \{\mnvy, \mney\}$}
        \State \Call{Disconnect}{$\mtdir, \mlink, \mlinkpar$}
        \State \Call{EraseTree}{$-\mtdir, \mlink$}
        \State \Return

    \Comment{(B) Stop recursion once a node that is not $\mtdir$-tree and not $\mnvy$ is reached.}
    \ElsIf {$\mnode\mdot\mntype \ne \mnvy$} 
        \If {$\mtdir = S$ \An $\mnode\mdot\mntype = \mnvu$}
            \Comment{Shift queries down to most recent $\mney$ if a $S$-tree $\mnvu$ node is reached.}
            \State \Call{ConvToTgtBranch}{$\mlink$}
            \State \Call{Queue}{$\mqcast, \mlink\mdot\mcost + \mlinkpar\mdot\mcost, \mlink$}
        \EndIf
        \State \Return
    \EndIf
    \Comment{$\mnode$ is $\mside$-sided, $\mtdir$-tree $\mnvy$ node at this point.}
    
%     \If {$\mtdir = S$ \An $\mnode\mdot\mntype \ne \mnvu$}
% %         \If {$\mnode\mdot\msidenode \ne \mside$ \An $\mnode\mdot\mntype \in \{\mnvy, \mney\}$}
% %         \Comment{Discard if previous node is $\mney$, current node is going to be $\mney$, and both have 
% % different sides.}
% %             \State \Call{Disconnect}{$T, \mlink_\mpar, \mlink$}
% %             \State \Call{EraseTree}{$T, \mlink$}
% %             \State \Return
% %         \ElsIf {$\fquery(\mlink) \ne \varnothing$ \Or $\mnode\mdot\mntype = \mney$} 
% %         \Comment{Stop recursion if a leaf link or a $S$-tree expensive node is reached.}
% %             \State \Return
%         % \Els
    
%         \State \Return
%     \ElsIf {$\mtdir = T$ \An $\mnode\mdot\mntype \ne $} 
%         % \If {$\mnode\mdot\mntype \ne \mnvy $}
%         %     \State \Return 
%         % \ElsIf {$\mnode\mdot\msidenode \ne \mside$}
%         %     \State \Call{Disconnect}{$T, \mlink, \mlinkpar$}
%         %     \State \Call{EraseTree}{$S, \mlink$}
%         % \EndIf
%     \EndIf

    \Comment{(C) Recurse.}
    \For {$\mlink_\mathrm{chd} \in \flinks(-\mtdir, \mlink) $}
        \State \Call{ConvToExBranchAux}{$\mtdir, \mlink, \mlink_\mathrm{chd}, \mside$}
    \EndFor

    \Comment{(D) Delete or re-anchor the current link.}
    \If {$\flinks(-\mtdir, \mlink) = \{\}$} 
    \Comment{Delete $\mlink$ if its branch is discarded}
        \State \Call{Disconnect}{$\mtdir, \mlink, \mlinkpar$}
        \State Remove $\mlink$ from $\fnode(\mlink)\mdot\mlinks_\mnode$
    \Else 
    \Comment{Anchor $\mlink$ to $\mside$-sided, $\mtdir$-tree, $\mney$ node.}
        \State $\mnode_\mnew \gets $ \Call{GetNode}{$\fx(\mnode), \mney, \mside, \mtdir$}
        \State \Call{Anchor}{$\mlink, \mnode_\mnew$}
    \EndIf
\EndFunction
\end{algorithmic}
\end{algorithm}
