# Supplementary material for: Rapid Vector-based Any-angle Path Planning with Non-convex Obstacles
Source: arXiv:2408.05806 source file (2024-08-11)
Supplement: Supplementary file 2 [file _alg_suppr2p_pushoverlap.tex]

\begin{algorithm}[!ht]
\begin{algorithmic}[1]
\caption{\textproc{PushOverlap}: Pushes a point into the overlap-buffer.}
\label{suppr2p:alg:pushoverlap}
\Function{PushOverlap}{$\mpoint$}
    \State Push $\mpoint$ into overlap-buffer.
\EndFunction
\end{algorithmic}
\end{algorithm}
