# Supplementary material for: Rapid Vector-based Any-angle Path Planning with Non-convex Obstacles
Source: arXiv:2408.05806 source file (2024-08-11)
Supplement: Supplementary file 3 [file tex_suppr2p_caster.tex]

\clearpage
\section{\textproc{Caster}: \textit{Handles a Casting Query}}
\setcounter{algorithm}{0}

The \textproc{Caster} function (Alg. \ref{suppalg:caster}) implements a casting query for a link $\mlink$.
A ray is cast from the source node of the link to the target node of the link.
The link can be anchored on either node, and is connected to one source link and at least one target link.
%%%%%%%%%%%%%%%%%%%%%%%%%%%%%%%%% ALG: CASTER  %%%%%%%%%%%%%%%%%%%%%%%%%%%%%%%%%%%%%
\begin{algorithm}[!ht]
\begin{algorithmic}[1]
\caption{\textproc{Caster}: handles a casting query.}
\label{suppalg:caster}
\Function{Caster}{$\mlink$}
    \State $\mnode_S \gets \fnode(\flink(S, \mlink))$
    \State $\mnode_T \gets \fnode(\flink(T, \mlink))$

    \State $\mray \gets $ \Call{GetRay}{$\fx(\mnode_S), \fx(\mnode_T)$}
    \State \Call{Cast}{$\mray$}

    \If {$\mray\mdot\mrtype = \mrvy$}
        \State \Return \Call{CastReached}{$\mray, \mlink$}
    \Else
        \State \Call{CastCollided}{$\mray, \mlink$}
        \State \Return $\mfalse$
    \EndIf
\EndFunction
\end{algorithmic}
\end{algorithm}

%%%%%%%%%%%%%%%%%%%%%%%%%%%%%%%%% ALG: CASTREACHED  %%%%%%%%%%%%%%%%%%%%%%%%%%%%%%%%%%%%%
\subsection{\textproc{CastReached}: \textit{Line-of-sight between Nodes of Cast}} 
The function \textproc{CastReached} (Alg. \ref{suppalg:castreached}) handles the case where a cast ray has line-of-sight.

In general, five cases occur when a cast reaches the target node from the source node.
\begin{enumerate}
    \item The shortest path is found when both nodes have cumulative visibility. This case is handled by the function \textproc{PathFound} (Alg. \ref{suppalg:pathfound}).
    \item The target node is an unreachable, $\mnun$-node. The caster query is discarded.
    \item The target node is a $\mntm$-node that is generated by an interrupted trace. The node may or may not be a valid turning point, and this case is handled by the function \textproc{ReachedTm} (Alg. \ref{suppalg:reachedtm}).
    \item Both nodes have unknown cumulative visibility. A new casting query for each target link of the link $\mlink$ is queued unless there are overlapping queries. This case is handled by the function \textproc{NoCumulativeVisibility} (Alg. \ref{suppalg:nocumulativevisibility}).
    \item Only the source node or target node has cumulative visibility. 
    If the source or target node has cumulative visibility, \rtwop{} proceeds to queue casting queries for the target links or source link respectively. This case is handled by the function \textproc{SingleCumulativeVisibility} (Alg. \ref{suppalg:singlecumulativevisibility}).
\end{enumerate}

% Fig. \ref{suppfig:castreached}.
\begin{algorithm}[!ht]
\begin{algorithmic}[1]
\caption{\textproc{CastReached}: cast has reached and ray has line-of-sight.}
\label{suppalg:castreached}
\Function{CastReached}{$\mray, \mlink$}
    \State $\mnode_S \gets \fnode(\flink(S, \mlink))$
    \State $\mnode_T \gets \fnode(\flink(T, \mlink))$
    
    \If{$\mnode_S\mdot\mntype = \mnvy $ \Or $\mnode_T\mdot\mntype = \mnvy$} 
        \Comment{Shortest path found.}
        \State \Call{PathFound}{$\mlink$}
        \State \Return $\mtrue$
    \ElsIf {$\mnode_T\mdot\mntype = \mnun$}
        \Comment{Discard if target node has type $\mnun$}
        \State \Call{DiscardReachedCast}{$\mlink$}   
    \ElsIf{$\mnode_T\mdot\mntype = \mntm$ }
        \Comment{Reached an interrupted trace.}
        \State \Call{ReachedTm}{$\mray, \mlink$}
    \ElsIf{$\mnode_S\mdot\mntype \notin \{\mnvy, \mney\}$ \An $\mnode_T\mdot\mntype \notin \{ \mnvy, \mney \}$}
        \Comment{$\mtrue$ if $\mnvu$ source node reached $\mnvu$ or $\mnoc$ target-tree node.}
        \State $(\mtdir_\mnext, \sim) \gets$ \Call{NoCumulativeVisibility}{$\mlink$}
        \State \Call{QueueReachedCast}{$\mtdir_\mnext, \mlink$}
    \Else
        \Comment{Either source or target node has cumulative visibility.}
        \State $(\mtdir_\mnext, \mnode_\mnext) \gets$ \Call{SingleCumulativeVisbility}{$\mray, \mlink$}
        \If {$\mnode_\mnext \ne \varnothing$}
            \State \Call{QueueReachedCast}{$\mtdir_\mnext, \mlink$}
        \EndIf
    \EndIf
    \State \Return $\mfalse$
\EndFunction
\end{algorithmic}
\end{algorithm}

%%%%%%%%%%%%%%%%%%%%%%%%%%%%%%%%% ALG: REACHEDTM  %%%%%%%%%%%%%%%%%%%%%%%%%%%%%%%%%%%%%
\newpage
\subsubsection{\textproc{ReachedTm}: \textit{Cast Reached for Target $\mntm$-node}}
The helper function \textproc{ReachedTm} handles cases when a cast reached a $\mntm$-node.
A $\mntm$-node is generated by an interrupted trace, which occurs when a number of corners is traced (Alg. \ref{suppalg:interrupt}), a recursive occupied-sector trace is called from the source node (Alg. \ref{suppalg:ocsecrule}), or a recursive angular-sector trace is called (Alg. \ref{suppalg:recurangsectrace}).
The $\mntm$-node has the same side as the interrupted trace that generated it.

As the $\mntm$-node can lie on any corner, \rtwop{} first checks if a turning point can be placed at the corner where the $\mntm$-node lies.
If a turning point cannot be placed at the corner, a trace resumes from the corner using the function \textproc{TracerFromLink} (Alg. \ref{suppalg:tracerfromlink}). 

If a turning point can be placed, the query proceeds by treating the target $\mntm$-node as a turning point.
If the source node has no cumulative visibility, 
the function \textproc{NoCumulativeVisibility} (Alg. \ref{suppalg:nocumulativevisibility}) is called.
If the source node has cumulative visibility, 
the function \textproc{SingleCumulativeVisibility} (Alg. \ref{suppalg:singlecumulativevisibility}) is called.

Even if a turning point can be placed, the target links of $\mlink$ may point into the occupied-sector of the target $\mntm$-node and are not castable.
A trace is generated for all non-castable links in \textproc{TraceFromTm} (Alg. \ref{suppalg:tracefromtm}), while a casting query is queued for each castable link in \textproc{CastFromTm} (Alg. \ref{suppalg:castfromtm}).

% Fig. \ref{suppfig:reachedtm}.

\begin{algorithm}[!ht]
\begin{algorithmic}[1]
\caption{\textproc{ReachedTm}: cast has reached a $\mntm$ node.}
\label{suppalg:reachedtm}
\Function{ReachedTm}{$\mray, \mlink$}
    \State $\mlink_S \gets \flink(S, \mlink)$
    \State $\mnode_S \gets \fnode(\flink(S, \mlink))$
    \State $\mnode_T \gets \fnode(\flink(T, \mlink))$
    \State $\mvray \gets \mray\mdot\mv_T - \mray\mdot\mv_S$
    \State $\mxtrace \gets \fx(\mnode_T)$
    \State $\msidetrace \gets \mnode_T\mdot\msidenode$
    \State $\mvnext \gets $ \Call{GetEdge}{$\msidetrace, \fx(\mnode_T)$}

    \Comment{Trace immediately if no turning point can be placed at $\mntm$ node.}
    \If {corner at $\mxtrace$ is non-convex \Or \Call{IsRev}{$\msidetrace, \mvray, \mvnext$} = $\mfalse$}
        \State \Call{TracerFromLink}{$\mlink$}
        \State \Return
    \EndIf

    \Comment{Try placing a turning point at $\mntm$ node.}
    \State $\mnode_\mnext \gets \varnothing$
    \If {$\mnode_S \notin \{\mnvy, \mney\}$}
        \State $(\sim, \mnode_\mnext) \gets $ \Call{NoCumulativeVisibility}{$\mlink$}
    \Else
        \State $(\sim, \mnode_\mnext) \gets $ \Call{SingleCumulativeVisibility}{$\mlink$}
        \If {$\mnode_\mnext = \varnothing$}  
            \State \Return
        \EndIf
    \EndIf

    \Comment{Queue castable links from new turning point.}
    \State $\hat{\mlinks}_\mathrm{newT} \gets $ \Call{CastFromTm}{$\mlink,  \mxtrace, \msidetrace, \mvnext$}
    
    \Comment{Continue tracing for non-castable links at new turning point.}
    \If {$\hat{\mlinks}_\mathrm{newT} \ne \{\}$}
        \State \Call{TraceFromTm}{$\mlink,  \mxtrace, \msidetrace, \mvnext, \hat{\mlinks}_\mathrm{newT}$}
    \EndIf
\EndFunction
\end{algorithmic}
\end{algorithm}

%%%%%%%%%%%%%%%%%%%%%%%%%%%%%%%% ALG: CASTROMTM %%%%%%%%%%%%%%%%%%%%%%%%%%%%%%%%%
\newpage
\subsubsection{\textproc{CastFromTm}: \textit{Try Casting From a Reached $\mntm$-node}}
The helper function \textproc{CastFromTm} (Alg. \ref{suppalg:castfromtm}) identifies castable target links of $\mlink$ and queues a casting query for each castable link.
Links that are not castable are pushed into an unordered set of links $\hat{\mlinks}_\mathrm{newT}$ and returned.
\begin{algorithm}[!ht]
\begin{algorithmic}[1]
\caption{\textproc{CastFromTm}: try casting from a new turning point at a reached $\mntm$ node.}
\label{suppalg:castfromtm}
\Function{CastFromTm}{$\mlink, \mxtrace, \msidetrace, \mvnext$}
    \State $\hat{\mlinks}_\mathrm{newT} \gets \{\}$
    \For {$\mlink_T \in \mlink\mdot\mlinks_T$}
        \State $\mnodepar \gets \fnode(\flink(T, \mlink_T))$
        \State $\mvpar \gets \mxtrace - \fx(\mnodepar)$
        % \If {$\mnodepar\mdot\mntype = \mnph$ \Or \Call{IsVis}{$\msidetrace, \mvpar, \mvnext$}$ = \mfalse$}
        %     \State Push $\mlink_T$ to back of $\hat{\mlinks}_\mathrm{newT}$
        %     \Comment{Trace from target node if next node is phantom point or not castable.}
        % \Else
        %     \Comment{Next node is castable and not phantom point.}
        %     \State $\mnode_\mnew \gets $ \Call{GetNode}{$\mxtrace, \mnvu, \msidetrace, T$}
        %     \State \Call{Anchor}{$\mlink_T, \mnode_\mnew$}
        %     \State \Call{Queue}{$\mqcast, \mlink\mdot\mcost + \mlink_T\mdot\mcost, \mlink_T$}
        % \EndIf
        \If {\Call{IsVis}{$\msidetrace, \mvpar, \mvnext$}}
            \Comment{Next node is castable and not phantom point.}
            \State $\mnode_\mnew \gets $ \Call{GetNode}{$\mxtrace, \mnvu, \msidetrace, T$}
            \State \Call{Anchor}{$\mlink_T, \mnode_\mnew$}
            \State \Call{Queue}{$\mqcast, \mlink\mdot\mcost + \mlink_T\mdot\mcost, \mlink_T$}
        \EndIf
    \EndFor
    \State \Return $\hat{\mlinks}_\mathrm{newT}$
\EndFunction
\end{algorithmic}
\end{algorithm}

%%%%%%%%%%%%%%%%%%%%%%%%%%%%%%%% ALG: TRACEFROMTM %%%%%%%%%%%%%%%%%%%%%%%%%%%%%%%%%
\newpage
\subsubsection{\textproc{TraceFromTm}: \textit{Try Tracing From a Reached $\mntm$-node}}
The helper function \textproc{TraceFromTm} (Alg. \ref{suppalg:tracefromtm}) generates a trace for all non-castable target links anchored on the target $\mntm$-node of a reached cast.
The links are contained in an unordered set $\hat{\mlinks}_\mathrm{newT}$, and are found by the function \textproc{CastFromTm} (Alg. \ref{suppalg:castfromtm}).
\begin{algorithm}[!ht]
\begin{algorithmic}[1]
\caption{\textproc{TraceFromTm}: try tracing from a new turning point at a reached $\mntm$ node.}
\label{suppalg:tracefromtm}
\Function{TraceFromTm}{$\mlink, \mxtrace, \msidetrace, \mvnext, \hat{\mlinks}_\mathrm{newT}$}
    \State $\mtrace \gets $ \Call{CreateTrace}{$\mxtrace, \msidetrace$}
    \State $\mtlink_\mathrm{newS} \gets $ \Call{CreateLink}{$\mtrace\mdot\mnode_S$}
    \State \Call{Connect}{$T, \mlink, \mtlink_\mathrm{newS}$}
    \State \Call{CreateNodelet}{$\mtlink_\mathrm{newS}, \mvnext, \mback, \mtrace\mdot\mnlets_S$}

    \For {$\mtlink_\mathrm{newT} \in \hat{\mlinks}_\mathrm{newT}$}
        \State $\mnode_\mathrm{newT} \gets \fnode(\flink(T, \mtlink_\mathrm{newT}))$
        \State \Call{Anchor}{$\mtlink_\mathrm{newT}, \mtrace\mdot\mnlets_T$}
        \State \Call{Disconnect}{$T, \mlink, \mtlink_\mathrm{newT}$}
        \State \Call{CreateNodelet}{$\mtlink_\mathrm{newT}, \mxtrace - \fx(\mnode_\mathrm{newT}), \mback, \mtrace\mdot\mnlets_T$}
    \EndFor

    \State $\mtrace\mdot\mxtrace \gets $ \Call{Trace}{$\mxtrace, \msidetrace$}
    \State \Call{Tracer}{$\mtrace$}
\EndFunction
\end{algorithmic}
\end{algorithm}

%%%%%%%%%%%%%%%%%%%%%%%%%%%%%%%% ALG: PATHFOUND %%%%%%%%%%%%%%%%%%%%%%%%%%%%%%%%%
\subsubsection{\textproc{PathFound}: \textit{Cumulative Visibility for Both Nodes of Reached Cast }}
The helper function \textproc{PathFound} (Alg. \ref{suppalg:pathfound}) returns the shortest path when the source and target nodes of a cast have cumulative visibility.

If the source node and target node have cumulative visibility, the nodes have to be $\mnvy$-type, as it is impossible for one node to be an $\mney$-node. 
An expensive query will have at least one source-tree or target-tree $\mney$-node along its examined path.
Subsequent casts by expensive queries will only occur if the source or target node of a cast is $\mney$-type.
By ensuring that either the source node or target node is $\mney$-type, the cost-to-go and cost-to-come of  nodes in subsequent casting queries can be verified, respectively.
As such, it is impossible for an expensive path to be unobstructed. 
An expensive path that is unobstructed implies that no cheaper, unobstructed path exists in the open-list, which is impossible since \rtwop{} is complete \cite{bib:r2}.
\begin{algorithm}[!ht]
\begin{algorithmic}[1]
\caption{\textproc{PathFound}: cast reached between two nodes with cumulative visibility.}
\label{suppalg:pathfound}
\Function{PathFound}{$\mlink$}
    % \State $\mnode_S \gets \fnode(\flink(T, \mlink))$
    % \State $\mnode_T \gets \fnode(\flink(S, \mlink))$
    \Comment{Found shortest path because link connects a $\mnvy$ source-tree node and a $\mnvy$ target-tree node.}
    % \State $path$ $\gets \{\fx(\mnode_T), \fx(\mnode_S)\}$
    \Comment{$path$ is accessible to all functions.}
    \State $\mlink_i \gets \flink(T, \mlink)$ 
    \State $path \gets \{\fx(\fnode(\mlink_i))\}$
    \Comment{There is only one target link.}
    \While {front of $path \ne \mxgoal$}
        \State $\mlink_i \gets \flink(T, \mlink_i)$
        \State Push $\fx(\fnode(\mlink_i))$ to front of $path$
    \EndWhile
    \State $\mlink_i \gets \flink(S, \mlink)$
    \State $path \gets $ Push $\fx(fnode(\mlink_i))$ to back of $path$
    \While {back of $path \ne \mxstart$}
        \State $\mlink_i \gets \flink(S, \mlink_i)$
        \State Push $\fx(\fnode(\mlink_i))$ to back of $path$
    \EndWhile
    \State \Return $\mtrue$
\EndFunction
\end{algorithmic}
\end{algorithm}

%%%%%%%%%%%%%%%%%%%%%%%%%%%%%%%% ALG: NOCUMULATIVEVISIBILITY %%%%%%%%%%%%%%%%%%%%%%%%%%%%%%%%%
\subsubsection{\textproc{NoCumulativeVisibility}: \textit{Unknown Cumulative Visibility for Both Nodes of Reached Cast}}
The helper function \textproc{NoCumulativeVisibility} (Alg. \ref{suppalg:nocumulativevisibility}) handles the case when the source and target node of a reached cast do not have verified cumulative visibility to the start or goal node respectively.
Such a case occurs if the source node is $\mnvu$-type, and if the target node is $\mnvu$, $\mnoc$ or $\mntm$-type.
\rtwop{} proceeds by queuing a casting query for each target link of the expanded link $\mlink$.
\begin{algorithm}[!ht]
\begin{algorithmic}[1]
\caption{\textproc{NoCumulativeVisibility}: cast reached between nodes with no cumulative visibility.}
\label{suppalg:nocumulativevisibility}
\Function{NoCumulativeVisibility}{$\mlink$}
    \State $\mnode_S \gets \fnode(\flink(S, \mlink))$
    \State $\mnode_T \gets \fnode(\flink(T, \mlink))$
    \State $\mnode_\mnext \gets $ \Call{GetNode}{$\fx(\mnode_T), \mnvu, \mnode_T\mdot\mside, S)$}
    \State \Call{FinishReachedCast}{$\mtdir_\mnext, \mnode_\mnext, \mlink, \mray$}
    \State \Return ($T, \mnode_\mnext$)
\EndFunction
\end{algorithmic}
\end{algorithm}

%%%%%%%%%%%%%%%%%%%%%%%%%%%%%%%% ALG: SINGLECUMULATIVEIVISIBILITY %%%%%%%%%%%%%%%%%%%%%%%%%%%%%%%%%
\subsubsection{\textproc{SingleCumulativeVisibility}: \textit{Cumulative Visibility for Either Node of Reached Cast}} \label{suppsec:singlecumulativevisibility}
The helper function \textproc{SingleCumulativeVisibility} (Alg. \ref{suppalg:singlecumulativevisibility}) 
when either the source or target node of a trace has cumulative visibility to the start or goal node respectively.

The algorithm progresses by checking nodes with no cumulative visibility, and determining the \textbf{next} direction is important.
If the source node has cumulative visibility, the next node is the target node, and the next direction is in the target-direction.
If the target node has cumulative visibility, the next node is the source node, and the next direction is in the source-direction.
The \textbf{previous} node is the source or target node which is not the next node.

The function updates the minimum cost at the next node's corner if the current query is the cheapest when reaching the next node. If the next node is the source node, the cost-to-go at the source node's corner is checked; if the next node is the target node, the cost-to-come at the target node's corner is checked.
The overlap rule subsequently discards or re-anchors expensive links to expensive nodes in \textproc{ConvToExBranch} (Alg. \ref{suppalg:convtoexbranch}). 

In \rtwo{}, more expensive links are re-anchored at $\mney$-nodes, and an expensive query does not generate additional queries \cite{bib:r2}.
\rtwop{} introduces a new rule to reduce the number of expensive queries further, by discarding the current query if it is expensive and is guaranteed to cross a cheaper path (see Sec. \ref{suppsec:overlap}).
The guarantee and the cheapest cost can be obtained by examining the Best object $\mbest_\mnext$ at the corner.
If the current query is the cheaper or equal to the minimum cost, the query updates $\mbest_\mnext$ instead.

\begin{algorithm}[!ht]
\begin{algorithmic}[1]
\caption{\textproc{SingleCumulativeVisibility}: cast reached between a node with cumulative visibility and another with no cumulative visibility.}
\label{suppalg:singlecumulativevisibility}
\Function{SingleCumulativeVisibility}{$\mray, \mlink$}
        \Comment{Either $\mnode_S$ or $\mnode_T$ has a type that is $\mney$ or $\mnvy$.}
    \State $\mnode_S \gets \fnode(\flink(S, \mlink))$
    \State $\mnode_T \gets \fnode(\flink(T, \mlink))$
    \State $\mtdir_\mnext \gets T$ if $\mnode_S\mdot\mntype \notin \{ \mnvy, \mney \}$ else $S$ 
        \Comment{$\mnode_S\mdot\mntype \notin \{\mnvy, \mney\} \implies \mnode_S\mdot\mntype = \mnvu$} 
    \State $\mnode_\mnext \gets \mnode_S$ if $\mtdir_\mnext = S$ else $\mnode_T$
    \State $\mnode_\mprev \gets \mnode_T$ if $\mtdir_\mnext = S$ else $\mnode_S$

    \If{$\mnode_\mprev\mdot\mntype = \mney$ \An $\mnode_\mprev\mdot\msidenode \ne \mnode_\mnext\mdot\msidenode$}
        \Comment{Discard if a node is expensive and both have different sides.}
        \State \Call{DiscardReachedCast}{$\mlink$}
        \State \Return ($\mtdir_\mnext, \varnothing$)
    \EndIf
    
    \State $\mcost_\mnext \gets $ \Call{MinCost}{$-\mtdir_\mnext, \mlink$} + $\lVert \mray\mdot\mx_T - \mray\mdot\mx_S \rVert$ 
    \State $\mpos_\mnext \gets \fpos(\mnode_\mnext)$
    \State $\mbest_\mnext \gets \fbest(-\mtdir_\mnext, \mpos_\mnext)$
    \State $\mside_\mbest \gets \mbest_\mnext\mdot\mnodebest\mdot\msidenode$
    \State $\mv_\mbest \gets \fx(\mnode_\mnext) - \mbest_\mnext\mdot\mxbest$
    \State $\mv_\mathrm{test} \gets \fx(\mnode_\mnext) - \fx(\mnode_\mprev))$
    \If {$\mbest_\mnext\mdot\mcost < c_\mnext$}
        \Comment{Current path to $\mnode_\mnext$ has larger ($-\mtdir_\mnext$)-cost than minimum at $\fpos(\mnode_\mnext)$.}
       
        \If {$\mnode_\mnext \mdot \msidenode = \mside_\mbest$ \An $\mtdir_\mnext \mside_\mbest(\mv_\mbest \times \mv_\mathrm{test}) > 0$}
            \State \Call{DiscardReachedCast}{$\mlink$}
            \State \Return ($\mtdir_\mnext, \varnothing$)
                \Comment{Future queries is always costlier as their paths cross the cheapest path to $\mx$.}
        \EndIf
        \State $\mnode_\mnext \gets $ \Call{GetNode}{$\fx(\mnode_\mnext), \mney, -\mtdir_\mnext$}
    \ElsIf{$\mbest_\mnext\mdot\mcost > c_\mnext$}
        \Comment{Current path to $\mnode_\mnext$ has smaller ($-\mtdir_\mnext$)-cost than minimum at $\fpos(\mnode_\mnext)$.}
        \State $\mnode_\mnext \gets $ \Call{GetNode}{$\fx(\mnode_\mnext), \mnvy, -\mtdir_\mnext$}
        \State $\mbest_\mnext\mdot\mcost \gets \mcost_\mnext$
        \State $\mbest_\mnext\mdot\mnodebest \gets \mnode_\mnew$ 
        \State $\mbest_\mnext\mdot\mxbest \gets \fx(\mnode_\mprev)$
        \State \Call{ConvToExBranch}{$-\mtdir_\mnext, \mpos_\mnext$}
    \Else
        \Comment{Current path to $\mnode_\mnext$ has identical ($-\mtdir_\mnext$)-cost than minimum at $\fpos(\mnode_\mnext)$.}
        \If {$\mnode_\mnext\mdot\msidenode = \mside_\mbest$ \An $\mtdir_\mnext \mside_\mbest(\mv_\mbest \times \mv_\mathrm{test})  \le 0$}
            \State $\mbest_\mnext\mdot\mxbest \gets \fx(\mnode_\mprev)$
            \Comment{Does not matter if previous node is $\mney$.}
        \EndIf
        \State $\mnode_\mnext \gets $ \Call{GetNode}{$\fx(\mnode_\mnext), \mnode_\mprev\mdot\mntype, -\mtdir_\mnext$}
    \EndIf
    \State \Call{FinishReachedCast}{$\mtdir_\mnext, \mnode_\mnext, \mlink, \mray$}
    \State \Return ($\mtdir_\mnext, \mnode_\mnext$)
\EndFunction
\end{algorithmic}
\end{algorithm}

%%%%%%%%%%%%%%%%%%%%%%%%%%%%%%%% ALG: DiscardReachedCast %%%%%%%%%%%%%%%%%%%%%%%%%%%%%%%%%
\subsubsection{\textproc{DiscardReachedCast}: \textit{Cumulative Visibility for Either Node of Reached Cast}}
The helper function \textproc{DiscardReachedCast} (Alg. \ref{suppalg:discardreachedcast}) discards a reached casting query and removes branches of links that only pass through the expanded link $\mlink$.
\begin{algorithm}[!ht]
\begin{algorithmic}[1]
\caption{\textproc{DiscardReachedCast}: discards the reached casting query.}
\label{suppalg:discardreachedcast}
\Function{DiscardReachedCast}{$\mlink$}
    \State $\mlink_S \gets \flink(S, \mlink)$
    \State \Call{Disconnect}{$T, \mlink_S, \mlink$}
    \State \Call{EraseTree}{$S, \mlink_S$}
    \State \Call{EraseTree}{$T, \mlink$}
\EndFunction
\end{algorithmic}
\end{algorithm}

%%%%%%%%%%%%%%%%%%%%%%%%%%%%%%%% ALG: FinishReachedCast %%%%%%%%%%%%%%%%%%%%%%%%%%%%%%%%%
\subsubsection{\textproc{FinishReachedCast}: \textit{Final Steps for a Reached Cast}}
The helper function \textproc{FinishReachedCast} performs the final steps of a reached cast.
The next node of the cast is converted into a new node, and the expanded link is re-anchored on the new node.
The ray representing the cast is merged into the angular sector of the source node (the rays are stored in the expanded link) if the source node has cumulative visibility.
Overlapping queries at the next node are identified and pushed into the overlapping buffer.
\begin{algorithm}[!ht]
\begin{algorithmic}[1]
\caption{\textproc{FinishReachedCast}: final steps for a reached cast.}
\label{suppalg:finishreachedcast}
\Function{FinishReachedCast}{$\mtdir_\mnext, \mnode_\mnext, \mlink, \mray$}
    \State \Call{Anchor}{$\mlink, \mnode_\mnew$}
    \State $\mlink\mdot\mcost \gets $ \Call{Cost}{$\mlink$}
    \For {$\mlink_\mnext \in \flinks(\mtdir_\mnext, \mlink)$}
        \State \Call{Isolate}{$-\mtdir_\mnext, \mlink_\mnext, \mlink$}
    \EndFor
    \If {$\fnode(\flink(S, \mlink))\mdot\mntype \in \{\mnvy, \mney\}$} 
        \Comment{Merge sector-rays if source node is $\mnvy$ or $\mney$. $\mtdir_\mnext$ is $T$.}
        \State \Call{MergeRay}{$-\mnode_\mnew\mdot\msidenode, \mlink, \mray$}
        \For {$\mlink_\mnext \in \flinks(T, \mlink)$}
            \State \Call{MergeRay}{$\mnode_\mnew\mdot\msidenode, \mlink_\mnext, \mray$}
        \EndFor
    \EndIf
    
    \State $numLinksAll \gets $ sum of $ \lvert \mnode\mdot\mlinks  \rvert $ for all $\mnode \in \fpos(\mnode_\mnext)\mdot\mnodes$ \Comment{Number of links anchored at new node's corner.}
    \State $numLinks \gets 1 + \lvert \flinks(\mtdir_\mnext, \mlink) \rvert$
    \Comment{Number of links anchored at corner by the current casting query.}
    \If {$numLinksAll > numLinks$} 
        \Comment{Trigger overlap rule later if reached a node with other links.}
        \State \Call{PushOverlap}{$\fpos(\mnode_\mnext)$}
    \EndIf
\EndFunction
\end{algorithmic}
\end{algorithm}

%%%%%%%%%%%%%%%%%%%%%%%%%%%%%%%% ALG: QUEUEREACHEDCAST %%%%%%%%%%%%%%%%%%%%%%%%%%%%%%%%%
\subsubsection{\textproc{QueueReachedCast}: \textit{Queue New Queries After a Reached Cast}}
The helper function \textproc{QueueReachedCast} (Alg. \ref{suppalg:queuereachedcast}) queues casting queries for links in the next direction (see Sec. \ref{suppsec:singlecumulativevisibility}).
\begin{algorithm}[!ht]
\begin{algorithmic}[1]
\caption{\textproc{QueueReachedCast}: queues subsequent castable queries.}
\label{suppalg:queuereachedcast}
\Function{QueueReachedCast}{$\mtdir_\mnext, \mlink$}
    \For {$\mlink_\mnext \in \flinks(\mtdir_\mnext, \mlink)$}
        \Comment{Queue next casting queries.}
        \State \Call{Queue}{$\mqcast, \mlink\mdot c + \mlink_\mnext\mdot c, \mlink_\mnext$}
    \EndFor
\EndFunction
\end{algorithmic}
\end{algorithm}

%%%%%%%%%%%%%%%%%%%%%%%%%%%%%%%%% ALG: CASTERCOLLIDED  %%%%%%%%%%%%%%%%%%%%%%%%%%%%%%%%%%%%%
\subsection{\textproc{CastCollided}: \textit{No Line-of-sight Between Nodes of Cast}}
The function \textproc{CastCollided} (Alg. \ref{suppalg:castcollided}) generates traces when a cast collides.
The \textbf{minor-trace} is generated from the collision point and has a side that is different from the source node of the cast.
If the target node is the goal node, and the source node is not a start node, the \textbf{third-trace} is generated from the source node.
The third-trace has a side that is the same as the source node.
The \textbf{major-trace} is generated from the collision point and has a side that is the same as the source node of the cast.

% Fig. \ref{suppfig:castcollided}.
\begin{algorithm}[!ht]
\begin{algorithmic}[1]
\caption{\textproc{CastCollided}: cast collided and ray has no line-of-sight.}
\label{suppalg:castcollided}
\Function{CastCollided}{$\mray, \mlink$}
    \State \Call{MinorTrace}{$\mray, \mlink$}
    \State \Call{ThirdTrace}{$\mray, \mlink$}
    \State \Call{MajorTrace}{$\mray, \mlink$}
\EndFunction
\end{algorithmic}
\end{algorithm}

%%%%%%%%%%%%%%%%%%%%%%%%%%%%%%%%% ALG: MINORTRACE  %%%%%%%%%%%%%%%%%%%%%%%%%%%%%%%%%%%%%
\subsubsection{\textproc{MinorTrace}: \textit{Generates a Trace With Different Side From Source Node}}
When a cast collides, the helper function \textproc{MinorTrace} (Alg. \ref{suppalg:minortrace}) generates a trace from the collision point. The trace, called the \textit{minor-trace}, has a side that is different from the source node.
The ray of the collided cast is merged into the source node of the cast, via a trace-link.

The reader may choose to ignore the third-trace (Alg. \ref{suppalg:thirdtrace}) if the minor-trace traces back  and re-encounters the source node of the cast.
The default implementation of \rtwop{} introduces an additional variable to the Trace object $\mtrace$ to monitor a re-encounter. However, if the minor-trace is interrupted, the re-encounter can no longer be monitored.
The monitoring is not shown in the pseudocode, as the additional step is not necessary for \rtwop{} to work.
\begin{algorithm}[!ht]
\begin{algorithmic}[1]
\caption{\textproc{MinorTrace}: minor-trace for a collided cast.}
\label{suppalg:minortrace}
\Function{MinorTrace}{$\mray, \mlink$}
    \State $\mnode_S \gets \fnode(\flink(S, \mlink))$
    \State $\mside_\mmnr \gets -\mnode_S\mdot\msidenode$
    \State $\mvray \gets \mray\mdot\mx_T - \mray\mdot\mx_S$
    \If {$\mnode_S\mdot\mntype = \mney$}
        \State \Return \Comment{Minor Trace cannot be generated for $\mney$ source node }
    \EndIf \Comment{The reader may choose to return if $\fxcol(\mside_\mmnr, \mray)$ is at the map boundary.}
    \State $\mtrace_\mmnr \gets $ \Call{CreateTrace}{$\fxcol(\mside_\mmnr, \mray), \mside_\mmnr$}
    \Comment{Create source nodelet and trace-link.}
    \State $\mtlink_\mathrm{newS} \gets $ \Call{CopyLink}{$\mlink, \mtrace_\mmnr\mdot\mtnode_S, \{S\}$}
    \State \Call{MergeRay}{$-\mside_\mmnr, \mtlink_\mathrm{newS}, \mray$}
    \State \Call{CreateNodelet}{$\mtlink_\mathrm{newS}, \mvray, \mback, \mtrace_\mmnr\mdot\mnlets_S$}
    \Comment{Create target nodelet and trace-link.}
    \State $\mtlink_\mathrm{newT} \gets $ \Call{CreateLink}{$\mtrace_\mmnr\mdot\mtnode_T$}
    \For {$\mlink_T \in \mlink\mdot\mlinks_T$}
        \State \Call{Connect}{$T, \mtlink_\mathrm{newT}, \mlink_T$}
    \EndFor
    \State \Call{CreateNodelet}{$\mtlink_\mathrm{newT}, -\mvray, \mback, \mtrace_\mmnr\mdot\mnlets_T$}
    \State \Call{Tracer}{$\mtrace_\mmnr$}
\EndFunction
\end{algorithmic}
\end{algorithm}

%%%%%%%%%%%%%%%%%%%%%%%%%%%%%%%%% ALG: THIRDTRACE  %%%%%%%%%%%%%%%%%%%%%%%%%%%%%%%%%%%%%
\subsubsection{\textproc{ThirdTrace}: \textit{Generates a Third Trace}}
When a cast from a non-start point to the goal point collides, the helper function \textproc{ThirdTrace} (Alg. \ref{suppalg:thirdtrace}) generates a trace from the source node.
The trace is called the \textit{third-trace}, which has the same side as the source node.
The ray of the collided cast is merged into the source node of the cast, via a trace-link.
\begin{algorithm}[!ht]
\begin{algorithmic}[1]
\caption{\textproc{ThirdTrace}: third-trace for a collided cast.}
\label{suppalg:thirdtrace}
\Function{ThirdTrace}{$\mray, \mlink$}
    \If {$\mray\mdot\mx_T \ne \mxgoal$ \Or $\mnode_S\mdot\mntype = \mney$}
        \State \Return 
        \Comment{Can ignore third-trace if minor-trace refinds source node...}
    \EndIf  
    \Comment{... or if $\mnode_S$ lies on an edge touching the map boundary.}
    \State $\mnode_S \gets \fnode(\flink(S, \mlink))$
    \State $\mside_\mthird \gets \mnode_S\mdot\msidenode$
    \State $\mvray \gets \mray\mdot\mx_T - \mray\mdot\mx_S$
    \State $\mtrace_\mthird \gets $ \Call{CreateTrace}{$\fx(\mnode_S), \mside_\mthird)$}
    \State $\mtrace_\mthird\mdot\mxtrace \gets $ \Call{Trace}{$\mtrace_\mthird\mdot\mxtrace,  \mtrace_\mthird\mdot\msidetrace$}
    \Comment{Third-trace begins at corner after source node.}
    
    \State $\mtlink_\mathrm{newS} \gets $ \Call{CopyLink}{$\mlink, \mtrace_\mthird\mdot\mnode_S, \{S\}$} \Comment{Create source nodelet and trace-link.}
    \State \Call{MergeRay}{$\mside_\mthird, \mtlink_\mathrm{newS}, \mray$}
    \State \Call{CreateNodelet}{$\mtlink_\mathrm{newS}, \mtrace_\mthird\mdot\mxtrace - \fx(\mnode_S), \mback, \mtrace_\mthird\mdot\mnlets_S$}

    \State $\mnode_\mathrm{newUn} \gets $ \Call{GetNode}{$\fx(\mnode_S), \mnun, \mside_\mthird, T$} 
    \Comment{Create a target-tree $\mnun$ node and link at casting point.}
    \State $\mlink_\mathrm{newUn} \gets $ \Call{CreateLink}{$\mnode_\mathrm{newUn}$}
    \For {$\mlink_T \in \mlink\mdot\mlinks_T$}
        \State \Call{Connect}{$T, \mlink_\mathrm{newUn}, \mlink_T$}
    \EndFor
    \State $\mlink_\mathrm{newUn}\mdot c \gets $ \Call{Cost}{$\mlink_\mathrm{newOc}$}

    \State $\mx_\mathrm{newOc} \gets $ \Call{Trace}{$\fx(\mnode_S), -\mside_\mthird$} 
    \Comment{Create a target-tree $\mnoc$ node and link at the corner before source node.}
    \State $\mnode_\mathrm{newOc} \gets $ \Call{GetNode}{$\mx_\mathrm{newOc}, \mnoc, \mside_\mthird, T$}
    \State $\mlink_\mathrm{newOc} \gets $ \Call{CreateLink}{$\mnode_\mathrm{newOc}$}
    \State \Call{Connect}{$T, \mlink_\mathrm{newOc}, \mlink_\mathrm{newUn}$}
    \State $\mlink_\mathrm{newOc}\mdot c \gets $ \Call{Cost}{$\mlink_\mathrm{newOc}$}

    \State $\mtlink_\mathrm{newT} \gets $ \Call{CreateLink}{$\mtrace_\mthird\mdot\mtnode_T$} 
    \Comment{Create target nodelet and trace-link.}
    \State \Call{Connect}{$T, \mtlink_\mathrm{newT}, \mlink_\mathrm{newOc}$}
    \State \Call{CreateNodelet}{$\mtlink_\mathrm{newT}, \mtrace_\mthird\mdot\mxtrace - \mx_\mathrm{newOc}, \mback, \mtrace_\mthird\mdot\mnlets_T$}

    \State \Call{Tracer}{$\mtrace_\mthird$}
\EndFunction
\end{algorithmic}
\end{algorithm}

%%%%%%%%%%%%%%%%%%%%%%%%%%%%%%%%% ALG: MAJORTRACE  %%%%%%%%%%%%%%%%%%%%%%%%%%%%%%%%%%%%%
\subsubsection{\textproc{MajorTrace}: \textit{Generates a Trace with Same Side as Source Node}}
When a cast collides, the helper function \textproc{MajorTrace} generates a trace from the collision.
The trace, called the \textit{major-trace}, has the same side as the source node.
The ray of the collided cast is merged into the source node of the cast, via a trace-link.
\begin{algorithm}[!ht]
\begin{algorithmic}[1]
\caption{\textproc{MajorTrace}: major-trace for a collided cast.}
\label{suppalg:majortrace}
\Function{MajorTrace}{$\mray, \mlink$}
    \State $\mnode_S \gets \fnode(\flink(S, \mlink))$
    \State $\mside_\mmjr \gets \mnode_S\mdot\msidenode$
    \State $\mvray \gets \mray\mdot\mx_T - \mray\mdot\mx_S$
    \State $\mtrace_\mmjr \gets $ \Call{CreateTrace}{$\fxcol(\mside_\mmjr, \mray)$}
    
    \State \Call{Anchor}{$\mlink, \mtrace_\mmjr\mdot\mtnode_S$}
    \Comment{$\mlink$ becomes source trace-link; Create source nodelet.}
    \State \Call{MergeRay}{$-\mside_\mmjr, \mlink, \mray$}
    \State \Call{CreateNodelet}{$\mlink, \mvray, \mback, \mtrace_\mmjr\mdot\mnlets_S$}

    \State $\mtlink_\mathrm{newT} \gets $ \Call{CreateLink}{$\mtrace_\mmjr\mdot\mnode_T$}
    \Comment{Create target nodelet and trace-links.}
    \For{$\mlink_T \in \mlink\mdot\mlinks_T$}
        \State \Call{Disconnect}{$T, \mlink, \mlink_T$} 
        \Comment{Connections in $\mlink$ prevents its removal if the mnr. or thd. traces fail.}
        \State \Call{Connect}{$T, \mtlink_\mathrm{newT}, \mlink_T$}
    \EndFor
    \State \Call{CreateNodelet}{$\mtlink_\mathrm{newT}, -\mvray, \mback, \mtrace_\mmjr\mdot\mnlets_T$}

    \State \Call{Tracer}{$\mtrace_\mmjr$}
\EndFunction
\end{algorithmic}
\end{algorithm}
