# Supplementary material for: Rapid Vector-based Any-angle Path Planning with Non-convex Obstacles
Source: arXiv:2408.05806 source file (2024-08-11)
Supplement: Supplementary file 4 [file tex_suppr2p_overlap.tex]

\section{Overlap Rule} \label{suppsec:overlap}
\setcounter{algorithm}{0}

The overlap rule reduces the number of queries by verifying line-of-sight and cost-to-come for nodes in overlapping paths.

The overlap rule consists of two major components implemented by the functions \textproc{ShrinkSourceTree} (Alg. \ref{suppalg:shrinksourcetree}) and \textproc{ConvToExBranch} (Alg. \ref{suppalg:convtoexbranch}). 
Both components that allow \rtwop{} to identify and discard some expensive queries. 
The \textproc{ShrinkSourceTree} function shifts overlapping queries from the leaf nodes to the first source-tree node with cumulative visibility ($\mney$ or $\mnvy$ node), shrinking the source-tree and expanding the target-tree in the process. 
By shifting the queries, \textproc{ShrinkSourceTree} allow \rtwop{} to verify the cost-to-come of overlapping nodes.
The \textproc{ConvToExBranch} (Alg. \ref{suppalg:convtoexbranch}) marks existing nodes at a location $\mx$ as expensive when a cast reaches $\mx$ with a shorter path than the existing paths.

% processes overlapping queries after a queued query is processed (Alg. \ref{suppalg:run}).

% Fig. \ref{suppfig:overlaprule}

%%%%%%%%%%%%%%%%%%%%%%%%%%%%%%%%% ALG: SHRINKSOURCETREE  %%%%%%%%%%%%%%%%%%%%%%%%%%%%%%%%%%%%%
\subsection{\textproc{ShrinkSourceTree}: \textit{Shifts Queries to Verify Cost-to-come}} 
The \textproc{ShrinkSourceTree} function (Alg. \ref{suppalg:shrinksourcetree}) shifts overlapping queries to a source-tree node along their path, simultaneously shrinking the source-tree and expanding the target-tree. 
The source-tree node is a $\mnvy$ or $\mney$ node that is furthest along the examined path from the start node.
Let $\mnode_\mathrm{SY}$ represent the source-tree $\mnvy$ or $\mney$ node.

Overlaps are identified in a trace or reached cast. 
In a trace, overlaps are identified when a turning point ($\mneu$ or $\mnvu$ node) is placed. 
If the corner at the turning point contain nodes that anchor other links, an overlap is identified (see \textproc{PlaceNode}, Alg. \ref{suppalg:placenode}). 
Likewise, in a reached cast, an overlap is identified at the source or target node if there are other links at the node's corner (see \textproc{FinishReachedCast}, Alg. \ref{suppalg:finishreachedcast}).
Once overlaps are identified, the corners where the overlaps occur are pushed in to the overlap-buffer.
They corners are subsequently processed by \textproc{ShrinkSourceTree} at the end of an iteration in \textproc{Run} (Alg. \ref{suppalg:run}).

The reader may notice that the corner pushed into the overlap-buffer for the tracing query may not be the point where overlap occurs (see \textproc{TryCastingFromTrace}, Alg. \ref{suppalg:castfromtrace}). 
While this may cause some overlapping queries to be missed, this reduces the size of the overlap buffer, and subsequent casts will still identify the missed queries.
For simplicity, the reader may choose to push the corner directly into the overlap-buffer in \textproc{PlaceNode} instead.

For each corner in the overlap-buffer, \textproc{ShrinkSourceTree} identifies source-tree $\mneu$ and $\mnvu$ nodes.
For each link anchored at the nodes, the path in the source direction is searched, and $\mnode_\mathrm{SY}$ is identified.
The function \textproc{ConvToTgtBranch} is called from the $\mnode_\mathrm{SY}$, converting all source-tree nodes in the target direction of $\mnode_\mathrm{SY}$ to target-tree $\mnvu$ nodes.
Any query in the target links are removed.
A casting query is subsequently queued from the $\mnode_\mathrm{SY}$ node.
\begin{algorithm}[!ht]
\begin{algorithmic}[1]
\caption{\textproc{ShrinkSourceTree}: process overlapping queries by shrinking the source-tree and requeuing at a $\mnvy$ $S$-tree node.}
\label{suppalg:shrinksourcetree}
\Function{ShrinkSourceTree}{\null}
    \For {$\mpos \in $ overlap-buffer}
        \For {$\mnode \in \mpos\mdot\mnodes$}
            \If {$\mnode\mdot\mtdirnode = T$ \Or $\mnode\mdot\mntype \notin \{\mneu, \mnvu\}$}
                \State \Continue
            \EndIf
            \For {$\mlink \in \mnode\mdot\mlinks_\mnode$}
                \State $\mlink_i \gets \mlink$
                \State $\mlink_{SY} \gets \flink(\mlink_i)$
                \While {$\fnode(\mlink_S)\mdot\mntype \notin \{\mnvy, \mney\}$}
                    \State $\mlink_i \gets \mlink_S$
                    \State $\mlink_{SY} \gets \flink(S, \mlink_{SY})$
                \EndWhile
                \State \Call{ConvToTgtBranch}{$\mlink_i$}
                \State \Call{Queue}{$\mqcast, \mlink_{SY}\mdot\mcost + \mlink_i\mdot\mcost, \mlink_i$}
            \EndFor
        \EndFor
    \EndFor
\EndFunction
\end{algorithmic}
\end{algorithm}

%%%%%%%%%%%%%%%%%%%%%%%%%%%%%%%%%%%%%%%%%% ALG: CONVTOTGTBRANCH %%%%%%%%%%%%%%%%%%%%%%%%%%%%%%%%%%
\subsection{\textproc{ConvToTgtBranch}: \textit{Converts Source-tree Nodes to Target-tree Nodes}} 
The function \textproc{ConvToTgtBranch} (Alg. \ref{suppalg:convtotgtbranch}) converts source-tree nodes to target-tree $\mnvu$ nodes, re-anchoring links in the process.
It is an auxiliary recursive function of \textproc{ShrinkSourceTree} (Alg. \ref{suppalg:shrinksourcetree}).
If a query is found at a leaf node, the query is removed to avoid data races with the new casting query in \textproc{ShrinkSourceTree}.
\begin{algorithm}[!ht]
\begin{algorithmic}[1]
\caption{\textproc{ConvToTgtBranch}: converts source-tree branches to target-tree branches.}
\label{suppalg:convtotgtbranch}
\Function{ConvToTgtBranch}{$\mlink$}
    \If {$\fquery(\mlink) \ne \varnothing$}
        \State \Call{Unqueue}{$\fquery(\mlink)$}
        \Comment{Unqueue and remove any query on leaf links to avoid data races.}
    \EndIf
    \If {$\fnode(\mlink)\mdot\mtdirnode = T$}
        \State \Return
        \Comment{Reached leaf node of target-tree.}
    \EndIf
    \For{$\mlink_T \in \mlink\mdot\mlinks_T$}
        \State \Call{ConvToTgtBranch}{$\mlink_T, \fnode(\mlink)$}
    \EndFor

    \State $\mnode_S \gets \fnode(\flink(S, \mlink))$
    \State $\mnode_\mnew \gets $ \Call{GetNode}{$\fx(\mnode_S), \mnvu, \mnode_S\mdot\msidenode, T$}
    \State \Call{Anchor}{$\mlink, \mnode_\mnew$}
    \State $\mlink\mdot\mcost \gets$ \Call{Cost}{$\mlink$}
\EndFunction
\end{algorithmic}
\end{algorithm}

%%%%%%%%%%%%%%%%%%%%%%%%%%%%%%%%%%%%%%%%%% ALG: CONVTOEXBRANCH %%%%%%%%%%%%%%%%%%%%%%%%%%
\subsection{\textproc{ConvToExBranch}: \textit{Identify Expensive Nodes After a Reached Cast.}}
The function \textproc{ConvToExBranch} converts existing nodes to expensive nodes when a reached cast finds a shorter path than other paths at a corner. 
The corner is represented by the Position object ($\mpos$).

The function is called by a reached cast when reaching a node results in the shortest path so far (see \textproc{SingleCumulativeVisibility} Alg. \ref{suppalg:singlecumulativevisibility}).
When $\mtdir = S$, $\mpos$ describes the corner at the target node, and cost-to-come is examined at the target node.
When $\mtdir = T$, $\mpos$ describes the corner at the source node, and the examined cost is cost-to-go is examined at the source node.
Links anchored on the existing $\mtdir$-tree $\mnvy$ node are identified, and connected $-\mtdir$ direction links are re-anchored on expensive nodes.
The function relies on the auxiliary recursive function \textproc{ConvToExBranchAux} to perform the conversion.
Expensive paths that are guaranteed to cross the current shortest path will be discarded.

\begin{algorithm}[!ht]
\begin{algorithmic}[1]
\caption{\textproc{ConvToExBranch}: converts a branch of $\mtdir$-tree $\mnvy$ nodes to $\mney$ nodes.}
\label{suppalg:convtoexbranch}
\Function{ConvToExBranch}{$\mtdir, \mpos$}
    \For {$\mnode \in \mpos\mdot\mnodes$}
        \If {$\mnode\mdot\mntype \ne \mnvy$ \Or $\mnode\mdot\mtdirnode \ne \mtdir$}
            \State \Continue 
            \Comment{ Check only $L$ or $R$-sided $\mtdir$-tree $\mnvy$ node/}
        \EndIf

        \State $\mbest \gets \fbest(\mtdir, \mpos)$
        \State $\mside_\mbest \gets \mbest\mdot\mnode_\mbest\mdot\msidenode$ 
        \State $\mv_\mbest \gets \mpos\mdot\mx - \mbest\mdot\mxbest$
        \For {$\mlink \in \mnode\mdot\mlinks_\mnode$}
            \State $\mlinkpar \gets \flink(\mtdir, \mlink)$
            \State $\mnodepar \gets \fnode(\mlinkpar)$
            \State $\mvpar \gets \mpos\mdot\mx - \fx(\mnodepar)$
            
            \If {$\mnode\mdot\msidenode = \mside_\mbest$ \An $\mtdir \mside_\mbest(\mv_\mbest \times \mvpar) > 0$}
            \Comment{Discard ex. path from $\mlink$ if it will cross the shortest path.}
                \State \Call{Disconnect}{$\mtdir, \mlink, \mlinkpar$}
                \State \Call{EraseTree}{$-\mtdir, \mlink$}
            \Else
                \State \Call{ConvToExBranchAux}{$\mtdir, \mlinkpar, \mlink, \mnode\mdot\msidenode$}
            \EndIf
            \State \Call{EraseTree}{$\mtdir, \mlinkpar$}
            \Comment{Discard $\mlinkpar$ if no more $(-\mtdir)$-links.} 
        \EndFor
    \EndFor
\EndFunction
\end{algorithmic}
\end{algorithm}

%%%%%%%%%%%%%%%%%%%%%%%%%%%%%%%%%%%%%%%%%% ALG: CONVTOEXBRANCH %%%%%%%%%%%%%%%%%%%%%%%%%%
\subsection{\textproc{ConvToExBranchAux}: \textit{Create Expensive Nodes and Discard Expensive Paths}}
The function \textproc{ConvToExBranchAux} (Alg. \ref{suppalg:convtoexbranch}) converts $\mtdir$-tree $\mnvy$ nodes to $\mney$ nodes and reanchors links to the $\mney$ nodes.
It is the auxiliary recursive function for \textproc{ConvToExBranch} (Alg. \ref{suppalg:convtoexbranch}).

\textproc{ConvToExBranchAux} discards expensive paths if they will remain expensive in subsequent queries.
The function stops once a node that is not $\mnvy$ and not in the $\mtdir$-tree is reached.
If the reached node is a source-tree $\mnvu$ node, the function \textproc{ConvToTgtBranch} (Alg. \ref{suppalg:convtotgtbranch}) is used to shift queries to the most recent $\mney$-node to verify cost-to-come.

\begin{algorithm}[!ht]
\begin{algorithmic}[1]
\caption{ConvToExBranchAux: converts $\mnvy$ nodes to $\mney$ nodes and discards paths that will be expensive.}
\label{suppalg:convtoexbranchaux}
\Function{ConvToExBranchAux}{$\mtdir, \mlinkpar, \mlink, \mside$}
    \State $\mnode \gets \fnode(\mlink)$

    \Comment{(A) Discard if par. node and current $\mnvy$ or $\mney$ node have different sides.}
    \If {$\mnode\mdot\msidenode \ne \mside$ \An $\mnode\mdot\mntype \in \{\mnvy, \mney\}$}
        \State \Call{Disconnect}{$\mtdir, \mlink, \mlinkpar$}
        \State \Call{EraseTree}{$-\mtdir, \mlink$}
        \State \Return

    \Comment{(B) Stop recursion once a node that is not $\mtdir$-tree and not $\mnvy$ is reached.}
    \ElsIf {$\mnode\mdot\mntype \ne \mnvy$} 
        \If {$\mtdir = S$ \An $\mnode\mdot\mntype = \mnvu$}
            \Comment{Shift queries down to most recent $\mney$ if a $S$-tree $\mnvu$ node is reached.}
            \State \Call{ConvToTgtBranch}{$\mlink$}
            \State \Call{Queue}{$\mqcast, \mlink\mdot\mcost + \mlinkpar\mdot\mcost, \mlink$}
        \EndIf
        \State \Return
    \EndIf
    \Comment{$\mnode$ is $\mside$-sided, $\mtdir$-tree $\mnvy$ node at this point.}
    
%     \If {$\mtdir = S$ \An $\mnode\mdot\mntype \ne \mnvu$}
% %         \If {$\mnode\mdot\msidenode \ne \mside$ \An $\mnode\mdot\mntype \in \{\mnvy, \mney\}$}
% %         \Comment{Discard if previous node is $\mney$, current node is going to be $\mney$, and both have 
% % different sides.}
% %             \State \Call{Disconnect}{$T, \mlink_\mpar, \mlink$}
% %             \State \Call{EraseTree}{$T, \mlink$}
% %             \State \Return
% %         \ElsIf {$\fquery(\mlink) \ne \varnothing$ \Or $\mnode\mdot\mntype = \mney$} 
% %         \Comment{Stop recursion if a leaf link or a $S$-tree expensive node is reached.}
% %             \State \Return
%         % \Els
    
%         \State \Return
%     \ElsIf {$\mtdir = T$ \An $\mnode\mdot\mntype \ne $} 
%         % \If {$\mnode\mdot\mntype \ne \mnvy $}
%         %     \State \Return 
%         % \ElsIf {$\mnode\mdot\msidenode \ne \mside$}
%         %     \State \Call{Disconnect}{$T, \mlink, \mlinkpar$}
%         %     \State \Call{EraseTree}{$S, \mlink$}
%         % \EndIf
%     \EndIf

    \Comment{(C) Recurse.}
    \For {$\mlink_\mathrm{chd} \in \flinks(-\mtdir, \mlink) $}
        \State \Call{ConvToExBranchAux}{$\mtdir, \mlink, \mlink_\mathrm{chd}, \mside$}
    \EndFor

    \Comment{(D) Delete or re-anchor the current link.}
    \If {$\flinks(-\mtdir, \mlink) = \{\}$} 
    \Comment{Delete $\mlink$ if its branch is discarded}
        \State \Call{Disconnect}{$\mtdir, \mlink, \mlinkpar$}
        \State Remove $\mlink$ from $\fnode(\mlink)\mdot\mlinks_\mnode$
    \Else 
    \Comment{Anchor $\mlink$ to $\mside$-sided, $\mtdir$-tree, $\mney$ node.}
        \State $\mnode_\mnew \gets $ \Call{GetNode}{$\fx(\mnode), \mney, \mside, \mtdir$}
        \State \Call{Anchor}{$\mlink, \mnode_\mnew$}
    \EndIf
\EndFunction
\end{algorithmic}
\end{algorithm}
