# Supplementary material for: Rapid Vector-based Any-angle Path Planning with Non-convex Obstacles
Source: arXiv:2408.05806 source file (2024-08-11)
Supplement: Supplementary file 5 [file tex_suppr2p_tracer.tex]

%%%%%%%%%%%%%%%%%%%%%%%%%%%%%%%%% ALG: TRACER  %%%%%%%%%%%%%%%%%%%%%%%%%%%%%%%%%%%%%
\newpage
\section{\textproc{Tracer}: \textit{Handles a Tracing Query}} 
\setcounter{algorithm}{0}

The main tracing function \textproc{Tracer} (Alg. \ref{suppalg:tracer}) implements the tracing query.
While 
There is only \textit{one} source nodelet during a trace, at at least one target nodelet.
The tracing query makes use of ordered set of nodelets $\mnlets_S$ and $\mnlets_T$ to prune, place and examine nodes.
Each nodelet contains a trace-link which connects a trace-node to a parent node, allowing the algorithm to examine a parent node with respect to the trace.
The source nodelet examines a source node, while a target nodelet examines a target node.
The source node lies on the source-tree, while the target node lies on the target-tree.

% Fig. \ref{supp:suppfig:tracer}.

Each iteration in \textproc{Tracer} evaluates a corner at $\mxtrace$.
If the trace traces to the source node (\textproc{RefoundSrc}, Alg. \ref{suppalg:refoundsrc}), the query is discarded.
If the trace does not progress with respect to the source node, \textproc{SrcProgCast} (Alg. \ref{suppalg:srcprogcast}) is called and a casting query is generated from the source node if the angular progression decreased by more than $180^\circ$ with respect to the source node. 
Otherwise, if the progression decreases by less than $180^\circ$, the trace moves to the next corner without evaluating the nodes.

If the trace has progressed with respect to the source node, the source and target nodes are examined further.
\textproc{TracerProc} (Alg. \ref{suppalg:tracerproc}) evaluates the target nodes with the progression, occupied-sector, and pruning rules.
\textproc{TracerProc} subsequently evaluates the source node with the angular-sector, occupied-sector, and pruning rules, which generates a recursive trace and discards the current trace if necessary.
\textproc{TracerProc} for the target nodes is called before the source node to ensure that the path is taut when a recursive trace is generated.

The interrupt rule interrupts the trace in \textproc{InterruptRule} (Alg. \ref{suppalg:interrupt}) if several corners are traced.
The placement rule in \textproc{PlaceRule} (Alg. \ref{suppalg:placerule}) tries to place a turning point or phantom point at the current position, and casts to any potentially visible target node from a placed turning point.
The placement rule engages the overlap rule instead if the query crossed paths with other queries. 

\begin{algorithm}[!ht]
\begin{algorithmic}[1]
\caption{\textproc{Tracer}: handles a tracing query.}
\label{suppalg:tracer}
\Function{Tracer}{$\mtrace$}
    \DoWhile
    \Comment{There is only one source link, and $\mtrace\mdot\mnlets_S = \{\mnlet_S\}$}
        \State $\mtrace\mdot\mnumcrns \gets \mtrace\mdot\mnumcrns + 1$
        % \State $\mnlet_S \gets $ the only trace-node in $\mtrace\mdot\mnlets_S$
        \If {\Call{RefoundSrc}{$\mtrace$}}
            \Comment{Refound source node}
            \State \Break
        \ElsIf {\Call{ProgRule}{$\mtrace, \fnlet(S, \mtrace)$}}
            \Comment{Not prog. w.r.t. source node.}
            \If {\Call{SrcProgCast}{$\mtrace$}}
                \Comment{Prog. reversed by $>180^\circ$ w.r.t. source node.}
                \State \Break
            \EndIf
        \Else
            \Comment{Prog. w.r.t. source node.}
            \If {\Call{TracerProc}{$T, \mtrace$}} \Comment{Order of execution is important.}
                \State \Break
            \ElsIf {\Call{TracerProc}{$S, \mtrace$}}
                \State \Break
            \ElsIf {\Call{InterruptRule}{$\mtrace$}}
                \State \Break
            \ElsIf {\Call{PlaceRule}{$\mtrace$}}
                \State \Break
            \EndIf
        \EndIf
        \State $\mtrace\mdot\mxtrace \gets $ \Call{Trace}{$\mtrace\mdot\mxtrace, \mtrace\mdot\msidetrace$}
    \EndDoWhile{$\mtrace\mdot\mxtrace \ne \varnothing$}
    \Comment{While trace is in map.}

    \For {$\mtdirpar \in \{S, T\}$} \Comment{Delete all dangling links.}
        \For {$\mnlet \in \fnlets(\mtdirpar, \mtrace)$}
            \State \Call{EraseTree}{$\mtdirpar, \mnlet\mdot\mtlink$}
        \EndFor
    \EndFor

\EndFunction
\end{algorithmic}
\end{algorithm}

%%%%%%%%%%%%%%%%%%%%%%%%%%%%%%%%% ALG: TRACERFROMLINK %%%%%%%%%%%%%%%%%%%%%%%%%%%%%%%%%%%%%
\subsection{\textproc{TracerFromLink}: \textit{Wrapper for} \textproc{Tracer}} \label{suppsec:tracerfromlink}
The tracing function \textproc{TracerFromLink} (Alg. \ref{suppalg:tracerfromlink}) wraps \textproc{Tracer} (Alg. \ref{suppalg:tracer}). 
\textproc{TracerFromLink} prepares a tracing query from a link $\mlink$ and calls \textproc{Tracer}.
The function is called when a tracing query is polled from the open-list (Alg. \ref{suppalg:run}), 
or when a $\mntm$-node is reached by a cast (Alg. \ref{suppalg:reachedtm}). 
\begin{algorithm}[!ht]
\begin{algorithmic}[1]
\caption{\textproc{TracerFromLink}: prepares a tracing query from a link.}
\label{suppalg:tracerfromlink}
\Function{TracerFromLink}{$\mlink$}
    \State $\mnode \gets \fnode(\mlink)$
    \State $\mnode_S \gets \fnode(\flink(S, \mlink))$
    \State $\mtrace \gets $ \Call{Tracer}{$\fx(\mnode), \mnode\mdot\msidenode$}
    \State \Call{Anchor}{$\mlink, \mtrace\mdot\mnode_S$}
    \State \Call{CreateNodelet}{$\mlink, \fx(\mnode) - \fx(\mnode_S), \mback, \mtrace\mdot\mnlets_S$}

    \For {$\mlink_T \in \mlink\mdot\mlinks_T$}
        \State $\mnode_T \gets \fnode(\flink(T, \mlink))$
        \State \Call{Disconnect}{$T, \mlink, \mlink_T$}
        \State \Call{Anchor}{$\mlink_T, \mtrace\mdot\mnode_T$}
        \State \Call{CreateNodelet}{$\mlink_T, \fx(\mnode) - \fx(\mnode_T), \mback, \mtrace\mdot\mnlets_T$}
    \EndFor

    \State \Call{Tracer}{$\mtrace$}
\EndFunction
\end{algorithmic}
\end{algorithm}

%%%%%%%%%%%%%%%%%%%%%%%%%%%%%%%%% ALG: TRACERPROC  %%%%%%%%%%%%%%%%%%%%%%%%%%%%%%%%%%%%%
\subsection{\textproc{TracerProc}: \textit{Process Source or Target-tree Nodes in Trace}}
Function \textproc{TracerProc} (\ref{suppalg:tracerproc}) examines the source node or target nodes. 
The function relies on the ordered set of nodelets $\mnlets_S$ and $\mnlets_T$ stored in the Trace object $\mtrace$ to examine the nodes.
If the trace is discarded or interrupted, either set becomes empty and the function returns.
While there can be multiple target nodelets at all times during a trace, there is always only \textit{one} source nodelet.

When \textproc{TracerProc} is called for the source node ($\mtdirpar=S$), the source node is first examined by the angular-sector rule. 
If the trace is no longer within the angular-sector of the node and the trace is unable to continue, the trace is interrupted or discarded.
Otherwise, the pruning rule or occupied-sector rule is checked depending on the side of the source node. If the trace has the same side as the source node, the pruning rule examines the source node. Otherwise, the occupied-sector rule examines the source node. 
The occupied-sector rule may interrupt the current trace with a recursive occupied-sector trace.

When \textproc{TracerProc} is called for the target nodes ($\mtdirpar=T$), the function checks the angular progression with respect to each target node before proceeding to the occupied-sector rule or pruning rule.
As the recursive occupied-sector trace for a target node ends quickly, the current trace will not be interrupted when the target nodes are examined.

\begin{algorithm}[!ht]
\begin{algorithmic}[1]
\caption{\textproc{TracerProc}: processes the trace in the source or target direction.}
\label{suppalg:tracerproc}
\Function{TracerProc}{$\mtdirpar, \mtrace=(\mxtrace, \msidetrace, \cdots)$}
    \For {$\mnlet \in \fnlets(\mtdirpar, \mtrace)$}
        \State $\mnodepar \gets \fnode(\mnlet\mdot\mtlink)$
        \State $\msidepar \gets \mnodepar\mdot\msidenode$
        \If {$\mtdirpar = T$ \An \Call{ProgRule}{$\mtrace, \mnlet$}}
            \State \Continue
        \ElsIf {$\mtdirpar = S$ \An \Call{AngSecRule}{$\mtrace, \mnlet$}        }
            \State \Continue 
        \ElsIf {$\fx(\mnodepar) \in \{\mx_\mstart, \mx_\mgoal \}$} 
            \Comment{Parent node is start or goal node.}
            \State \Continue
        \ElsIf {$\msidepar = \msidetrace$}
            \State \Call{PruneRule}{$\mtrace, \mnlet$}
        \Else 
            \State \Call{OcSecRule}{$\mtrace, \mnlet$}
        \EndIf
    \EndFor
    \State \Return $\fnlets(\mtdirpar, \mtrace) = \{\}$
    \Comment{Returns true if the $\mtdirpar$ set of nodelets is empty.}
\EndFunction
\end{algorithmic}
\end{algorithm}

%%%%%%%%%%%%%%%%%%%%%%%%%%%%%%%%% ALG: SRCPROGCAST  %%%%%%%%%%%%%%%%%%%%%%%%%%%%%%%%%%%%%
\subsection{\textproc{SrcProgCast}: \textit{Cast From Highly Winded Source Node}}
The \textproc{SrcProgCast} function (Alg. \ref{suppalg:srcprogcast}) interrupts the trace when the winding counter increases to two for the source node. When the counter increases to two, the progression has decreased by more than $180^\circ$ from the maximum angular progression.
The maximum angular progression points to a phantom point, which is replaced with an unreachable $\mnun$-node.
A casting query is subsequently queued from the source node to the $\mnun$-node.

The phantom point can be found directly from the only target trace-node when the trace is not progressed with respect to the source node.
The point can be found as no target nodes are placed when the angular progression is reversing for the source node, and the trace is in the convex hull of a non-convex obstacle.
No target nodes need to be placed in a convex hull as they would be pruned once the trace exits the convex hull and resumes angular progression with respect to the source node.
% Fig. \ref{suppfig:srcprogcast}
\begin{algorithm}[!ht]
\begin{algorithmic}[1]
\caption{\textproc{SrcProgCast}: queues a cast when progression w.r.t. source node has decreased by more than $180^\circ$.}
\label{suppalg:srcprogcast}
\Function{SrcProgCast}{$\mtrace = (\mxtrace, \cdots)$}
    \State $\mnlet_S \gets \fnlet(S, \mtrace)$
    \If {$\mnlet_S\mdot\mcprog > 1$}
    
        \Comment{(A) Create new target-tree $\mnun$-node and anchor target link there.}
        \State $\mnlet_T \gets \fnlet(T, \mtrace)$ 
        \Comment{The only target nodelet.}
        \State $\mlink_T \gets \flink(T, \mnlet_T\mdot\mtlink)$
        \State $\mnode_T \gets \fnode(\mlink_T)$ 
        \Comment{Target node is a phantom point.}
        \State $\mnode_\mathrm{newUn} \gets $ \Call{GetNode}{$\fx(\mnode_T), \mnun, \mnode_T\mdot\msidenode, T$}
        \State \Call{Anchor}{$\mlink_T, \mnode_\mathrm{newUn}$}

        \Comment{(B) Create new target-tree $\mnvu$-node and re-anchor source trace-link there.}
        \State $\mlink_\mathrm{newVu} \gets \mnlet_S\mdot\mtlink$
        \State $\mlink_S \gets \flink(S, \mlink_\mathrm{newVu})$
        \State $\mnode_S \gets \fnode(\mlink_S)$
        \State $\mnode_\mathrm{newVu} \gets $ \Call{GetNode}{$\fx(\mnode_S), \mnvu, \mnode_S\mdot\msidenode, T$}
        \State \Call{Anchor}{$\mlink_\mathrm{newVu}, \mnode_\mathrm{newVu}$}
        \State \Call{Connect}{$T, \mlink_\mathrm{newVu}, \mlink_T$}
        \State $\mlink_\mathrm{newVu}\mdot\mcost \gets $ \Call{Cost}{$\mlink_\mathrm{newVu}$}

        \Comment{(C) Queue casting query for source trace-link.}
        \State \Call{Queue}{$\mqcast, \mlink_S\mdot\mcost + \mlink_\mathrm{newVu}\mdot\mcost, \mlink_\mathrm{newVu}$}
        \State \Return $\mtrue$
    \EndIf
    \State \Return $\mfalse$
\EndFunction
\end{algorithmic}
\end{algorithm}

%%%%%%%%%%%%%%%%%%%%%%%%%%%%%%%%% ALG: REFOUNDSRC  %%%%%%%%%%%%%%%%%%%%%%%%%%%%%%%%%%%%%
\subsection{\textproc{RefoundSrc}: \textit{Checks if Trace Traces to Source Node}}
Function \textproc{RefoundSrc} (Alg. \ref{suppalg:refoundsrc}) returns $\mtrue$ if a trace traces to its examined source node.
A trace can never trace to a target node in \rtwop.
\begin{algorithm}[!ht]
\begin{algorithmic}[1]
\caption{\textproc{RefoundSrc}: checks if a trace has reached its source node.}
\label{suppalg:refoundsrc}

\Function{RefoundSrc}{$\mtrace = (\mxtrace, \cdots)$}
    \State $\mnlet_S \gets \fnlet(S, \mtrace)$
    \State $\mnode_S \gets \fnode(\mnlet_S\mdot\mtlink)$
    \State \Return $\mxtrace = \fx(\mnode_S)$
\EndFunction
\end{algorithmic}
\end{algorithm}

%%%%%%%%%%%%%%%%%%%%%%%%%%%%%%%%% ALG: PROGRULE  %%%%%%%%%%%%%%%%%%%%%%%%%%%%%%%%%%%%%
\clearpage
\subsection{\textproc{ProgRule}: \textit{Checks Angular Progression w.r.t. a Node}}
Function \textproc{ProgRule}  (Alg. \ref{suppalg:progrule}) returns $\mfalse$ if the trace at corner $\mxtrace$ has progressed with respect to a parent node or $\mtrue$ if the trace has not progressed. 

If a trace crosses the progression ray, it will intersect a line (unbounded on both sides) coincident to the ray (bounded on one side). 
The progression ray is drawn from a parent node in the direction $\mvprog$ and stretches to infinity. If a trace crossed the front of the ray, the trace intersected the ray.
Let $\mvprog'$ be a ray that is drawn from a parent node in the direction $-\mvprog$. If a trace crossed behind the ray, then the trace crossed $\mvprog'$.

As only the direction of the intersection with respect to the parent node needs to be known, the intersection need not be calculated explicitly. 
Let $itx =  \fsgn(\mvprev \times \mv_\mpar) \fsgn(\mvprev \times \mvprog ) \in {-1, 0, 1}$. 
$\mvprev$ is the previous trace direction that reached $\mx$. $\mv_\mpar$ is the vector pointing from the parent node to $\mx$. $\mvprog$ is the progression ray.
$-1$ and $1$ indicate that the trace has crossed behind and in front of the ray respectively. $0$ indicates that $\mvprev$ is parallel to $\mv_\mpar$ and/or $\mvprev$ is parallel to $\mvprog$. 
For both parallel cases, the reader may verify that the trace is always progressed with respect to the parent node.
Note that $\mvprog \ne 0$, $\mvprev \ne 0$ and $\mvprog \ne 0$ when $itx$ is evaluated.
\begin{algorithm}[!ht]
\begin{algorithmic}[1]
\caption{\textproc{ProgRule}: implements the progression rule.}
\label{suppalg:progrule}
\Function{ProgRule}{$\mtrace = (\mxtrace, \msidetrace, \cdots)$, $\mnlet = (\mtlink, \mvprog, \mcprog) $}
% \State $(\mtdirpar, \msidepar, \mnodepar, \mvpar, \mvprev, \sim) \gets $\Call{TraceCalc}{$\mtrace, \mnlet$}
    \State $\mnodepar \gets \fnode(\mtlink)$
    \State $\mtdirpar \gets \mnodepar\mdot\mtdirnode$ 
    \State $\mvpar \gets \mxtrace - \fx(\mnodepar)$
    \State $\mvprev \gets -$\Call{GetEdge}{$\mxtrace, -\msidetrace$} 
\If{ $\mvpar = 0$} 
    \State $\mvpar \gets $\Call{Bisect}{$\mxtrace$} \Comment{Occurs for start nodes or checkerboard corners}
\EndIf
\State $u \gets \mtdirpar \msidetrace (\mvpar \times \mvprog)$
\State $isProg \gets u < 0 $ \Or ($u = 0$ \An $\mvpar \sdot \mvprog > 0$) \Comment{$\mtrue$ if $\mvpar$ lies to $(\mtdirpar \msidetrace)$-side of $\mvprog$, or if both are pointing in same direction }
\State $wasProg \gets \mcprog = 0$

\State $itx \gets \fsgn(\mvprev \times \mvpar) \fsgn(\mvprev \times \mvprog )$ \Comment{$itx = 1$:  crossed in front of ray; $itx =-1$: crossed behind ray.}
\If {$isProg = \mtrue$ \An $wasProg = \mtrue$}
    \State $\mnlet\mdot\mvprog \gets \mvpar$ \Comment{Update ray}
\ElsIf {$isProg = \mtrue$ \An $wasProg = \mfalse$}
    \If {$itx \ge 0$}
        \State $\mnlet\mdot\mcprog \gets \mcprog - 1$ \Comment{Unwind}
        \If {$\mcprog > 0$}  \Comment{Not completely unwound, flip ray}
            \State $\mnlet\mdot\mvprog \gets -\mvprog$ 
            \State $isProg \gets \mfalse$
        \Else \Comment{Unwound completely, update ray}
            \State $\mnlet\mdot\mvprog \gets \mvpar$ 
        \EndIf
    \Else  \Comment{Wind and flip ray}
        \State $\mnlet\mdot\mcprog \gets \mcprog + 1$
        \State $\mnlet\mdot\mvprog \gets -\mvprog$ 
        \State $isProg \gets \mfalse$
    \EndIf
\ElsIf{$isProg = \mfalse$ \An $wasProg = \mtrue$} 
    \If {$itx \le 0$} \Comment{No winding: case occurs if start node lies on an obstacle's edge}
        \State $\mnlet\mdot\mvprog \gets -\mvprog$
        \State $isProg \gets \mtrue$
    \Else  \Comment {Wind}
        \State $\mnlet\mdot\mcprog \gets \mcprog + 1$ 
    \EndIf
\EndIf
\State \Return \Not $isProg$
\EndFunction
\end{algorithmic}
\end{algorithm}

%%%%%%%%%%%%%%%%%%%%%%%%%%%%%%%%% ALG: PRUNERULE  %%%%%%%%%%%%%%%%%%%%%%%%%%%%%%%%%%%%%
\clearpage
\subsection{\textproc{PruneRule}: \textit{Checks if a Node can be Pruned}}
Function \textproc{PruneRule} (Alg. \ref{suppalg:prune}) prunes a node if the resulting path at the examined corner at $\mxtrace$ is not taut. A source-tree node that is $\mnvy$ cannot be pruned by the rule, as it is handled by the angular-sector rule.

Pruning of source-tree $\mnvy$-nodes are handled by the angular-sector. 
As the angular-sector of a source-tree $\mnvy$-node can only be fully evaluated at the next corner, any pruning at the current corner can cause \rtwop{} to be incomplete.

\begin{algorithm}[!ht]
\begin{algorithmic}[1]
\caption{\textproc{PruneRule}: implements the pruning rule.}
\label{suppalg:prune}
\Function{PruneRule}{$\mtrace = (\mxtrace, \msidetrace, \cdots)$, $\mnlet = (\mtlink, \cdots) $}
    \State $\mnodepar \gets \fnode(\mtlink)$
    \State $\mtdirpar \gets \mnodepar\mdot\mtdirnode$ 
    \State $\msidepar \gets \mnodepar\mdot\msidenode$
    \State $\mvpar \gets \mxtrace - \fx(\mnodepar)$

    \Comment{\textbf{(A) $\mnvy$ source-tree nodes are handled by the angular sector rule.}}
\If{$\mtdirpar = S$ \An $\mnodepar \mdot \mntype = \mnvy$}
    \State \Return 
\EndIf 

    \Comment{(B) Try pruning for each parent node and link.}
\For{$\mlinkpar \in \flinks(\mtdirpar, \mtlink)$}

    \Comment{(B.1) Taut: go to next parent node and link.}
    \State $\mnodegpar \gets \fnode(\flink(\mtdirpar, \mlinkpar))$
    \State $\mvgpar \gets \fx(\mnodepar) - \fx(\mnodegpar)$  
    \If {\Call{IsTaut}{$\mtdirpar$, $\msidepar$, $\mvpar$, $\mvgpar$}}
        \State \Continue
        \Comment{$(\mxtrace, \mnodepar), \mnodegpar)$ is taut and nothing is pruned.}
    \EndIf

    \Comment{(B.2) Not taut: prune parent node.}
    \State \Call{Disconnect}{$-\mtdirpar$, $\mlinkpar$, $\mtlink$} 
    \State $\mlink_\mnew \gets $ \Call{Isolate}{$-\mtdirpar$, $\mlinkpar$, $\varnothing$, $\ftnode(\mtdirpar, \mtrace)$}
    \If{$\mtdirpar = T$} 
        \Comment{Remove rays if prune in target direction.}
        \State $\mlink_\mnew \mdot \mray_L \gets \varnothing$
        \State $\mlink_\mnew \mdot \mray_R \gets \varnothing$
    \EndIf

    % \Comment{(B.3) Not taut: If new parent node is target-tree $\mnph$ or $\mnun$, re-anchor new parent links to $\mntm$ parent node.}
    % \If{$\mnode_\mpar \mdot \mntype \in \{\mntm,\mnun\}$ \An $\mnode_\mgpar \mdot \mntype = \mnph$} 
    % % \Comment{Move links from old gpar. $\mnph$ nodes to $\mntm$ if old par. node is $\mntm$.} 
    %     \State $\mnode_\mathrm{newT} \gets $ \Call{GetNode}{$\fx(\mnode_\mgpar)$,  $\mnode_\mpar\mdot\mntype$, ($\mnode_\mgpar \mdot \msidenode$), $\mtdirpar$}
    %     \For {$\mlink_\mnph \in \flinks_\mpar(\mlink_\mpar)$} 
    %         \State $\mlink_\mathrm{newT} \gets $ \Call{Isolate}{$-\mtdirpar$, $\mlink_\mnph$, $\mlink_\mnew$, $\mnode_\mathrm{newT}$} 
    %     \EndFor
    % \EndIf

    \Comment{(B.4) Create new nodelet for new parent node.}
    \State \Call{CreateNodelet}{$\mlink_\mnew, \mx_\mtrace - \fx(\mnode_\mgpar), \mback, \fnlets(\mtdirpar, \mtrace)$} 
    \Comment{Push to back to try pruning later.}
        
\EndFor

        \Comment{(C) Remove current nodelet and trace-link if trace-link has no more parent links.}
\If {$\flinks(\mtdirpar, \mtlink)  = \{\}$ } 
    \State Remove $\mtlink$ from $\ftnode(\mtdirpar, \mtrace)\mdot\mlinks_\mnode$ 
    \State Remove $\mnlet$ from $\fnlets(\mtdirpar, \mtrace)$
\EndIf
\EndFunction
\end{algorithmic}
\end{algorithm}

%%%%%%%%%%%%%%%%%%%%%%%%%%%%%%%%% ALG: PRUNERULE  %%%%%%%%%%%%%%%%%%%%%%%%%%%%%%%%%%%%%
\clearpage
\subsubsection{\textproc{IsTaut}: \textit{Checks if a Node is Taut}}
The helper function \textproc{IsTaut} (Alg. \ref{suppalg:istaut}) evaluates the path segments around a node and returns $\mtrue$ if the node can be pruned.
\begin{algorithm}[!ht]
\begin{algorithmic}[1]
\caption{\textproc{IsTaut}: checks tautness of path segment.}
\label{suppalg:istaut}
\Function{IsTaut}{$\mtdirpar$, $\msidepar$, $\mvpar$, $\mvgpar$}
    \State $u \gets \mtdirpar \msidepar (\mvpar \times \mvgpar)$ 
    \If {$u = 0$} \Comment{Return $\mtrue$ if angle between $\mvpar$ and $\mvgpar$ is $180^\circ$, $\mfalse$ if $0^\circ$}
        \State \Return $\mvpar \sdot \mvgpar \ge 0$ 
    \Else \Comment{Returns $\mtrue$ if $\mvgpar$ lies to the $\mtdirpar \msidepar$-side of $\mvpar$ }
        \State \Return $u > 0$
    \EndIf
\EndFunction
\end{algorithmic}
\end{algorithm}

%%%%%%%%%%%%%%%%%%%%%%%%%%%%%%%%% ALG: OCSECRULE  %%%%%%%%%%%%%%%%%%%%%%%%%%%%%%%%%%%%%
\clearpage
\subsection{\textproc{OcSecRule}: \textit{Checks if a Node can be Pruned}}
The function \textproc{OcSecRule} (Alg. \ref{suppalg:ocsecrule}) implements the occupied-sector rule.
The function returns immediately if the trace is outside the occupied-sector of parent node.
If the trace enters the occupied-sector for the source node, a recursive occupied-sector trace is generated, and the current trace is interrupted.

If the trace enters the occupied-sector of a target node that is $\mnoc$ type, the trace is discarded because the path has looped.
Otherwise, if the target is a non-$\mnoc$ node, a $\mnoc$ target-tree node is placed in the source-direction of the target node.
The placement can be considered part of a short recursive occupied-sector trace.

% Fig. \ref{suppfig:ocsecrule}
\begin{algorithm}[!ht]
\begin{algorithmic}[1]
\caption{\textproc{OcSecRule}: implements the occupied-sector rule.}
\label{suppalg:ocsecrule}
\Function{OcSecRule}{$\mtrace = (\mx_\mtrace, \mside_\mtrace, \cdots)$, $\mnlet = (\mtlink, \cdots) $}
    % \State $(\mtdirpar, \msidepar, \mnodepar, \mvpar, \mvprev, \sim) \gets $\Call{TraceCalc}{$\mtrace, \mnlet$}
    \State $\mnodepar \gets \fnode(\mtlink)$
    \State $\mtdirpar \gets \mnodepar\mdot\mtdirnode$ 
    \State $\msidepar \gets \mnodepar\mdot\msidenode$
    \State $\mvpar \gets \mxtrace - \fx(\mnodepar)$
    \State $\mvocpar \gets $ \Call{GetEdge}{$\fx(\mnodepar), -\mtdirpar\msidepar$}

    \Comment{(A) Parent is target $\mnoc$-node. Discard trace if it enters oc.sec., return otherwise.}
    \If {$\mnodepar \mdot \mntype = \mnoc$} 
        \Comment{Previously entered occupied-sector of a target-tree node (gpar. node)}
        \State $\mnodegpar \gets \fnode(\flink(T, \flink(T, \mtlink)))$ 
        \State $\mvgpar \gets \fx(\mnodepar) - \fx(\mnodegpar)$  
        \If {$\mside_\mpar (\mv_\mpar \times \mv_\mgpar) \le 0$}
            \Comment{Discard as path has looped around gpar. node and par. $\mnoc$ node} 
            \State \Call{EraseTree}{$T, \mtlink$} 
            \State Remove $\mnlet$ from  $\mtrace\mdot\mnlets_T$
        \EndIf
        \State \Return % $\mfalse$
    
    \Comment{(B) Return if not in occupied-sector.}
    \ElsIf{$\mtdirpar \mside_\mpar (\mv_\mpar \times \mvocpar) \le 0$} 
        \State \Return % $\mfalse$
        \Comment{Not in occupied-sector of $\mnode_\mpar$}
    \EndIf

    \Comment{(C) Create recursive oc-sec. trace if entered oc-sec. of source node.} 
    \If{$\mtdirpar = S$}
        \State $\mtrace_\mnew \gets $ \Call{CreateTrace}{$\fx(\mnodepar), \msidepar$}
        \State \Call{Anchor}{$\mtlink$, $\mtrace_\mnew\mdot\mnode_S$} 
        \State Move $\mnlet$ to $\mtrace_\mnew\mdot\mnlets_S$ \Comment{s.t. $\mtrace_\mnew\mdot\mnlets_S = \{\mnlet\}$ and $\mtrace\mdot\mnlets_S = \{\}$}
        \State $\mnlet\mdot\mvprog \gets \mvocpar$

        \State $\mnode_\mathrm{newTm} \gets$ \Call{GetNode}{$\mxtrace, \mntm, \msidetrace, T$}
        \Comment{Create a $\mntm$ target-tree node and re-anchor target trace-links there.}
        \State $\mtlink_\mathrm{newT} \gets $ \Call{CreateLink}{$\mtrace_\mnew\mdot\mnode_T$}
        \State \Call{CreateNodelet}{$\mtlink_\mathrm{newT}, -\mvpar, \mback, \mtrace_\mnew \mdot \mnlets_T$}

        \For{$\mnlet_T \in \mtrace\mdot\mnlets_T$} 
            \State $\mlink_\mathrm{newT} \gets \mnlet_T\mdot\mtlink$
            \State \Call{Anchor}{$\mlink_\mathrm{newT}$, $\mnode_\mathrm{newTm}$}
            \State $\mlink_\mathrm{newT}\mdot\mcost \gets$ \Call{Cost}{$\mlink_T$}
            \State \Call{Connect}{$T$, $\mtlink_\mathrm{newT}$, $\mlink_\mathrm{newT}$}
        \EndFor

        \State $\mtrace_\mnew\mdot\mxtrace \gets $ \Call{Trace}{$\mtrace_\mnew\mdot\mxtrace$, $\mtrace_\mnew\mdot\msidetrace$}
        \Comment{Start recursive trace from the $\msidepar$-side corner of the source node}
        \State \Call{Tracer}{$\mtrace_\mnew$} 

    \Comment{(D) Place target-tree $\mnoc$-node if entered oc-sec. of target node.} 
    \Else 
        \State $\mx_\mathrm{newOc} \gets $ \Call{Trace}{$\fx(\mnodepar)$, $-\msidepar$} 
        % \Comment{Get the $-\msidepar$ corner of the target node.}
        \State $\mnode_\mathrm{newOc} \gets$ \Call{GetNode}{$\mx_\mathrm{newOc}, \mnoc, \msidepar, T$} 
        % \Comment{Get $\mnoc$ target-tree node at $-\msidepar$ corner.}
        \State \Call{Anchor}{$\mtlink$, $\mnode_\mathrm{newOc}$} 
        % \Comment{Transfer expanded link to $\mnoc$ node.}
        \State $\mtlink\mdot\mcost \gets $ \Call{Cost}{$\mtlink$}
        \State $\mtlink_\mathrm{newT} \gets $ \Call{CreateLink}{$\mtrace\mdot\mtnode_T$}
        \State \Call{Connect}{$T, \mtlink_\mathrm{newT}, \mtlink$}
        \State $\mnlet\mdot\mtlink \gets \mtlink_\mathrm{newT}$
        \State $\mnlet\mdot\mvprog \gets \mvpar$
    \EndIf
\EndFunction
\end{algorithmic}
\end{algorithm}

%%%%%%%%%%%%%%%%%%%%%%%%%%%%%%%%% ALG: ANGSEC  %%%%%%%%%%%%%%%%%%%%%%%%%%%%%%%%%%%%%
\subsection{\textproc{AngSecRule}: \textit{Implements the Angular-sector Rule}}
The function \textproc{AngSecRule} (Alg. \ref{suppalg:angsecrule}) implements the angular-sector rule for the source node.

Four helper functions breaks the implementation down into smaller parts. They are \textproc{RayNotCrossed} (Alg. \ref{suppalg:raynotcrossed}), \textproc{AngSecPrune} (Alg. \ref{suppalg:angsecprune}), \textproc{Project} (Alg. \ref{suppalg:project}), and \textproc{RecurAngSecTrace} (Alg. \ref{suppalg:recurangsectrace}).
\textproc{AngSecRule} examines the $\msidetrace$-sided ray $\mray$ of the source node's angular sector, and determines if the trace is within the angular-sector.
If the trace is within the angular-sector, \textproc{AngSecRule} returns without calling the other helper functions.

The other helper functions are called when the trace exits the source node's angular sector.
\textproc{AngSecPrune} prunes the source node if the resulting path is not taut after exiting the source node's angular sector.
% The pruned source node is guaranteed to be $\mnvy$ type. 
% A prune by the angular-sector rule occurs only when the $\mray$ ends at the source node, indicating that the node is a source-tree node with cumulative visibility ($\mnvy$ or $\mney$ type). $\mney$-nodes are pruned by the pruning rule, as no recursive angular-sector trace can be generated for an $\mney$ node.
% $\mney$ node. A recursive angular-sector trace cannot occur for an $\mney$ node as the $\mney$ node cannot no longer be pruned by future queries.
If a prune by the angular-sector occurs, the current trace continues regardless of any subsequent recursive angular-sector trace.
\textproc{Project} (Alg. \ref{suppalg:project}) projects the ray $\mray$ and finds the projected ray's collision point.
\textproc{RecurAngSecTrace} generates a recursive angular-sector trace if the current trace did not pass through the projected ray's collision point.
% Fig. \ref{suppfig:angsecrule}.
\begin{algorithm}[!ht]
\begin{algorithmic}[1]
\caption{\textproc{AngSecRule}: implements the angular-sector rule.}
\label{suppalg:angsecrule}
\Function{AngSecRule}{$\mtrace = (\mxtrace, \msidetrace, \cdots)$, $\mnlet = (\mtlink, \cdots) $}
    \State $\mray \gets \fray(\msidetrace, \mtlink)$

    \If {\Call{RayNotCrossed}{$\mray, \mtrace, \mnlet$}}
        \State \Return $\mfalse$
    \EndIf
    \State \Call{AngSecPrune}{$\mray, \mtrace, \mnlet$}
    \State \Call{Project}{$\mray$}
    \State \Call{RecurAngSecTrace}{$\mray, \mtrace, \mnlet$}
    \State \Return $\mtrue$
    
\EndFunction
\end{algorithmic}
\end{algorithm}

%%%%%%%%%%%%%%%%%%%%%%%%%%%%% ALG:RAYNOTCROSSED %%%%%%%%%%%%%%%%%%%%%%%%%%%%%%%%%%%%
\subsubsection{\textproc{RayNotCrossed}: \textit{Checks if Trace is Within Angular-Sector}}
The function \textproc{RayNotCrossed} examines the $\msidetrace$-sided ray $\mray$ of the source node and compares the ray with the current position of the trace.
If the trace crosses the ray, the function returns $\mtrue$.

If the current position lies on the ray, it is not clear if the ray has been crossed. 
The function breaks ties by considering how the line-of-sight function \textproc{LOS} (Alg. \ref{suppalg:los}) returns the first corners after a collision. 
\textproc{LOS} relies on the directional vector bisecting the corner at the current position to place the first corners. 
The consideration is required because the first corners are subsequently checked in \textproc{RecurAngSecTrace} -- the ray can only be considered crossed if the $\msidetrace$-sided first corner lies at the current position.
However, the ray may not have been projected, and the algorithm can only check against the bisecting vector.

To eliminate errors resulting from floating point calculations, the algorithm is designed to handle only discrete, integer calculations. This helps the authors to verify proofs, and provides a foundation from which \rtwop{} can be improved.
The reader may choose to implement a much simpler intersection check that uses floating point calculations instead.

\begin{algorithm}[!ht]
\begin{algorithmic}[1]
\caption{\textproc{RayNotCrossed}: checks if a sector-ray is crossed.}
\label{suppalg:raynotcrossed}
\Function{RayNotCrossed}{$\mray, \mtrace = (\mxtrace, \msidetrace, \cdots)$, $\mnlet = (\mtlink, \cdots) $}
    \If {$\mray = \varnothing$} 
        \State \Return $\mtrue$
    \EndIf
    \State $\mvray \gets \mray\mdot\mx_T - \mray\mdot\mx_S$
    \State $\mlink_S \gets \flink(S, \mtlink)$ \Comment{$\mlink$ has only one source link.}
    \State $\mvpar \gets \mxtrace - \fx(\fnode(\mlink_S))$
    
    \State $u_\mathrm{ray,par} \gets \msidetrace (\mvray \times \mvpar)$
    \If{$u_\mathrm{ray,par} > 0$}
        \State \Return $\mtrue$
        \Comment{Return as ray is not crossed.}
    \ElsIf{$u_\mathrm{ray,par} = 0$} 
        \Comment{$\mvray$ and $\mvpar$ are parallel. Use bisecting oc-sec. vector to break ties.}
        \State $\mv_\mathrm{crn} \gets $ \Call{Bisect}{$\mxtrace$} 
        \State $u_\mathrm{ray,crn} \gets \msidetrace(\mvray \times \mv_\mathrm{crn})$ 
        \If {$u_\mathrm{ray,crn} > 0$ \Or $u_\mathrm{ray,crn} = 0$ \An $\mvray \sdot \mv_\mathrm{crn} > 0$} 
            \State \Return $\mtrue$
            \Comment{Ray is not crossed: $\mvray$ lies strictly to the $\msidetrace$-side of $\mv_\mathrm{crn}$, or...}
        \EndIf
        \Comment{...ray points away from corner: $\mvray$ opposite to $\mv_\mathrm{crn}$.}
    \EndIf 
    \State \Return $\mfalse$.
\EndFunction
\end{algorithmic}
\end{algorithm}

%%%%%%%%%%%%%%%%%%%%%%%%%%%%% ALG:ANGSECPRUNE %%%%%%%%%%%%%%%%%%%%%%%%%%%%%%%%%%%%
\subsubsection{\textproc{AngSecPrune}: \textit{Tries to Prune Source Node}}
The function \textproc{AngSecPrune} (Alg. \ref{suppalg:angsecprune}) tries to prune the source node if the resulting path is not taut after exiting the node's angular sector.
If the node cannot be pruned, nothing is done.
When a prune occurs, the current trace continues regardless of a subsequent recursive angular-sector trace.

The pruned source node is guaranteed to be $\mnvy$ type. 
A prune by the angular-sector rule occurs only when the $\mray$ ends at the source node, indicating that the node is a source-tree node with cumulative visibility ($\mnvy$ or $\mney$ type). $\mney$-nodes are pruned by the pruning rule, as no recursive angular-sector trace can be generated for an $\mney$ node.
$\mney$ node. A recursive angular-sector trace cannot occur for an $\mney$ node as the $\mney$ node can no longer be pruned by future queries.
\begin{algorithm}[!ht]
\begin{algorithmic}[1]
\caption{\textproc{AngSecPrune}: tries to prune a trace's source node after exiting the node's angular-sector.}
\label{suppalg:angsecprune}
\Function{AngSecPrune}{$\mray, \mtrace = (\mxtrace, \msidetrace, \cdots)$, $\mnlet = (\mtlink, \cdots) $}
    \State $\mlink_S \gets \flink(S, \mtlink)$
    \State $\mnode_S \gets \fnode(\mlink_S)$
    
    \State $prunable \gets \mray\mdot\mx_T = \fx(\mnode_S)$ \Comment{Prunable if sector-ray ends at parent source-tree node, or...}
    \State $prunable \gets prunable $ \Or ($\mray\mdot\mx_T = \mxstart$ \An $\mray\mdot\mx_S = \mxgoal$ \An $\msidetrace = \mnode_S\mdot\msidenode$) \Comment{...prunable if ray is special sector-ray for start node and the side traced is same as start node's side.}
    \If {$prunable$} 
        \State $\mtlink_\mathrm{newS} \gets $ \Call{Isolate}{$T, \mlink_S, \varnothing, \mtrace, \mtrace\mdot\mtnode_S$}
        \State $\mnode_\mathrm{newS} \gets \fnode(\flink(S, \mtlink_\mathrm{newS}))$
        \State \Call{CreateNodelet}{$\mtlink_\mathrm{newS}, \mxtrace - \fx(\mnode_\mathrm{newS}), \mback, \mtrace\mdot\mnlets_S$}
    \EndIf
\EndFunction
\end{algorithmic}
\end{algorithm}

%%%%%%%%%%%%%%%%%%%%%%%%%%%%% ALG:ANGSECPRUNE %%%%%%%%%%%%%%%%%%%%%%%%%%%%%%%%%%%%
\subsubsection{\textproc{RecurAngSecTrace}: \textit{Tries to Generate a Recursive Angular-sector Trace}}
The function \textproc{RecurAngSecTrace} generates a recursive angular-sector trace if the trace crosses the collision point of the projected ray $\mray$.
The trace crosses the collision point if the current position $\mxtrace$ lies on the first $\msidetrace$-sided  corner from the collision point.

A $(-\msidetrace)$-sided $\mnun$ node is placed at the first $\msidetrace$-side corner from the collision point. The node ensures that the $(-\msidetrace)$-sided recursive trace progresses with respect to a target node at the initial corner traced.
The $\mnun$ node will be pruned at the initial corner if the resulting path is not taut.
A $\mntm$ node is placed at the current trace location, and is the target node of the $\mnun$ node.
Additionally the $\mnun$ node is unreachable because if a query from the recursive trace reaches the node, a cheaper path has to exist that can reach the $\mntm$ node.

% Fig. \ref{suppfig:recurangsectrace}
\begin{algorithm}[!ht]
\begin{algorithmic}[1]
\caption{\textproc{RecurAngSecTrace}: performs a recursive angular-sector trace if required.}
\label{suppalg:recurangsectrace}
\Function{RecurAngSecTrace}{$\mray, \mtrace = (\mxtrace, \msidetrace, \cdots)$, $\mnlet = (\mtlink, \cdots) $}
    \State $\mnode_S \gets \fnode(\flink(S, \mtlink))$
    \If {$\fxcol(\msidetrace, \mray) = \mxtrace$ \Or $\mnodepar\mdot\mntype = \mney$}
    \Comment{Discard if trace crossed the collision point of the sector-ray, or...}
        \State \Call{EraseTree}{$S, \mtlink$}
        \Comment{...parent source-tree node is $\mney$ (recur. trace has different side from $\mney$ node).}
        \State Remove $\mnlet$ from $\mtrace\mdot\mnlets_S$
    \Else   
        \Comment{Trace did not cross sector-ray's collision point. Recursive ang-sec. trace.}
        \State $\mtrace_\mnew \gets $ \Call{CreateTrace}{$\fxcol(-\msidetrace, \mray), -\msidetrace$}
        \State $\mnlet\mdot\mvprog \gets \mtrace_\mnew\mdot\mxtrace - \fx(\mnode_S)$
        
        \State $\mx_\mathrm{newUn} \gets \fxcol(\msidetrace, \mray)$ 
        \Comment{Create a $\mnun$ target-tree node at $\msidetrace$ corner of collision.}
        \If {$\mx_\mathrm{newUn} = \fxcol(-\msidetrace, \mray)$} 
            \Comment{Collision at corner instead of edge.}
            \State $\mx_\mathrm{newUn} \gets $ \Call{Trace}{$\mx_\mathrm{newUn}, \msidetrace$}
        \EndIf
        \State $\mnode_\mathrm{newUn} \gets $ \Call{GetNode}{$\mx_\mathrm{newUn}, \mnun, -\msidetrace, T$}
        \State $\mlink_\mathrm{newT} \gets $ \Call{CreateLink}{$\mnode_\mathrm{newUn}$}
        
        \State $\mnode_\mathrm{newTm} \gets$ \Call{GetNode}{$\mxtrace, \mntm, \msidetrace, T$} 
        \Comment{Create a $\mntm$ target-tree node at current corner at $\mxtrace$}
        \For {$\mnlet_T \in \mtrace\mdot\mnlets_T$}
            \State $\mlink_\mathrm{newTT} \gets $ \Call{CopyLink}{$\mnlet_T\mdot\mtlink, \mnode_\mathrm{newTm}, \{T\}$} 
             \Comment{Re-anchor target trace-links from current trace at $\mntm$ node.}
            \State $\mlink_\mathrm{newTT}\mdot\mcost \gets$ \Call{Cost}{$\mlink_\mathrm{newTT}$}
            \State \Call{Connect}{$T$, $\mlink_\mathrm{newT}, \mlink_\mathrm{newTT}$}
        \EndFor
        \State $\mlink_\mathrm{newT}\mdot\mcost \gets$ \Call{Cost}{$\mlink_\mathrm{newT}$}

        \State $\mtlink_\mathrm{newT} \gets $ \Call{CreateLink}{$\mtrace_\mnew\mdot\mtnode_T$} 
        \State \Call{Connect}{$T, \mtlink_\mathrm{newT}, \mlink_\mathrm{newT}$}
        \State \Call{CreateNodelet}{$\mtlink_\mathrm{newT}, \mtrace_\mnew\mdot\mxtrace - \mx_\mathrm{newUn}, \mfront, \mtrace_\mnew\mdot\mnlets_T$}

        \State \Call{Tracer}{$\mtrace_\mnew$}
    \EndIf
\EndFunction
\end{algorithmic}
\end{algorithm}

%%%%%%%%%%%%%%%%%%%%%%%%%%%%%%%%% ALG: INTERRUPT RULE  %%%%%%%%%%%%%%%%%%%%%%%%%%%%%%%%%%%%%
\clearpage
\subsection{Interrupt Rule} \label{suppsec:interrupt}
Function \textproc{InterruptRule} (Alg. \ref{suppalg:interrupt}) implements the interrupt rule, which interrupts and queues a trace when a number of corners are traced and if the trace is progressed with respect to all source-tree and target-tree parent nodes.

The number of corners to interrupt $numInterrupt$ is arbitrary. 
The larger $numInterrupt$ is, the slower \rtwop{} may get for simple queries with few turning points as the tracing queries spend more time on non-convex contours. 
The smaller $numInterrupt$ is, the slower \rtwop{} may be for more complex queries with many turning points due to frequent open-list queuing. The default value is $numInterrupt = 10$.
\begin{algorithm}[!ht]
\begin{algorithmic}[1]
\caption{\textproc{InterruptRule}: implements the interrupt rule.}
\label{suppalg:interrupt}
\Function{InterruptRule}{$\mtrace = (\mxtrace, \msidetrace, \cdots)$}
    
    \Comment{(A) Return if trace has only checked a few corners, and trace is not prog. w.r.t. all nodes.}
    \State $allProgS \gets $ $\mnlet_S \mdot \mcprog = 0 $ for all $ \mnlet_S \in \mtrace\mdot\mnlets_S$
    \State $allProgT \gets $ $\mnlet_T \mdot \mcprog = 0 $ for all $ \mnlet_T \in \mtrace\mdot\mnlets_T$
    \If{$\mtrace\mdot\mnumcrns < numInterrupt$ \Or $allProgS = \mfalse$ \Or $allProgT = \mfalse$}
        \State \Return $\mfalse$
    \EndIf

    \Comment{(B) Otherwise, interrupt and create nodes and re-anchor trace-links.}
    \State $\mnode_\mathrm{newSVu} \gets$ \Call{GetNode}{$\mxtrace, \mnvu, \msidetrace, S$}
    \State $\mlink_\mathrm{newS} \gets$ $\fnlet(S, \mtrace)\mdot\mtlink$ 
    \State \Call{Anchor}{$\mlink_\mathrm{newS}, \mnode_\mathrm{newSVu}$}
    \State $\mlink_\mathrm{newS}\mdot\mcost \gets$ \Call{Cost}{$\mlink_\mathrm{newS}$}
    
    \State $\mnode_\mathrm{newTTm} \gets$ \Call{GetNode}{$\mxtrace, \mntm, \msidetrace, T$}
    \For{$\mnlet_T \in \mtrace\mdot\mnlets_T$}
        \State $\mlink_\mathrm{newT} \gets \mnlet_T\mdot\mtlink$
        \State \Call{Anchor}{$\mlink_\mathrm{newT}, \mnode_\mathrm{newTTm}$}
        \State $\mlink_\mathrm{newT}\mdot\mcost \gets$ \Call{Cost}{$\mlink_\mathrm{newT}$}
        \State \Call{Connect}{$T, \mlink_\mathrm{newS}, \mlink_\mathrm{newT}$}
    \EndFor

    \Comment{(C) Mark for overlap-rule check, or queue a tracing query}
    \If {$\mtrace\mdot\moverlap = \mtrue$}
        \State \Call{PushOverlap}{\Call{GetPos}($\mxtrace$)}
    \Else
        \State $f \gets \mlink_\mathrm{newS}\mdot\mcost + $ \Call{GetMinCost}{$T, \mlink_\mathrm{newS}$}
        \State \Call{Queue}{$\mqtrace, f, \mlink_\mathrm{newS} $}
    \EndIf
    \State \Return $\mtrue$
\EndFunction
\end{algorithmic}
\end{algorithm}

%%%%%%%%%%%%%%%%%%%%%%%%%%%%%%%%% ALG: PLACERULE  %%%%%%%%%%%%%%%%%%%%%%%%%%%%%%%%%%%%%
\clearpage
\subsection{\textproc{PlaceRule}: Places Points and Checks Castability}
\textproc{PlaceRule} implements the placement rule and tries to place a turning point or phantom point.
The function exits after a phantom point is placed, or if no point can be placed.

If a turning point is placed, the function examines if the trace has crossed a path from a different query.
If a different path is crossed, the overlap rule will check the placed links after the trace ends.
The trace will end with the placement rule if all target nodes can be cast to.
% If there are other links, the trace has crossed a the trace is marked for an overlap-rule check that engages after all target nodes become castable.
% The rule subsequently tries to cast to each target node, queuing a casting query for each castable node.

The function is aided by four helper functions, \textproc{IsRev} (Alg. \ref{suppalg:isrev}), \textproc{IsVis} (Alg. \ref{suppalg:isvis}), \textproc{PlaceNode} (Alg. \ref{suppalg:placenode}), and \textproc{CastFromTrace} (Alg. \ref{suppalg:castfromtrace}).

\begin{algorithm}[!ht]
\begin{algorithmic}[1]
\caption{\textproc{PlaceRule}: implements the placement rule and queues a cast if needed.}
\label{suppalg:placerule}
\Function{PlaceRule}{$\mtrace = (\mxtrace, \msidetrace, \cdots)$}
    \State $\mtdirpar \gets S$ if corner at $\mxtrace$ is convex, $T$ otherwise

    \State $\mnlet_\mnew \gets $ \Call{PlaceNode}{$\mtdirpar, \mtrace$}

    \If {$\mnlet_\mnew = \varnothing$ \Or $\mtdirpar = T$}
        \State \Return $\mfalse$
        \Comment{Turning point not placed. Nothing else to do.}
    \ElsIf {$\sum \lvert \mnode\mdot\mlinks_\mnode \rvert > 1$ for all $\mnode \in $ \Call{GetPos}{$\mxtrace$}$\mdot\mnodes$ }
        \State $\mtrace\mdot\moverlap \gets \mtrue$
        \Comment{Mark for overlap rule if multiple links are anchored at $\mxtrace$.}
    \EndIf

    \If {$\mnlet_\mnew \ne \varnothing$ \An $\mtdirpar = S$}
        \Comment{Try casting if a turning point is placed.}
        \State \Call{CastFromTrace}{$\mtrace, \mnlet_\mnew$}
    \EndIf

    \State \Return $\mtrace\mdot\mnlets_T = \{\}$ 
    \Comment{Return $\mtrue$ if no more target trace-nodes.}
\EndFunction
\end{algorithmic}
\end{algorithm}

%%%%%%%%%%%%%%%%%%%%%%%%%%%%%%%%% ALG: ISREV  %%%%%%%%%%%%%%%%%%%%%%%%%%%%%%%%%%%%%
\subsubsection{\textproc{IsRev}: \textit{Checks if Angular Progression Will Reverse}}
The helper function \textproc{IsRev} (Alg.\ref{suppalg:isrev}) returns $\mtrue$ if tracing the next edge from the current corner at $\mxtrace$ causes the angular progression to reverse with respect to the parent node.
\begin{algorithm}[!ht]
\begin{algorithmic}[1]
\caption{\textproc{IsRev}: checks if a trace's angular progression will reverse at the next edge of a corner.}
\label{suppalg:isrev}
\Function{IsRev}{$\mtdirpar, \msidetrace, \mvpar, \mvnext$}
    \State \Return $\mtdirpar \msidetrace (\mvpar \times \mvnext) < 0$
\EndFunction
\end{algorithmic}
\end{algorithm}

%%%%%%%%%%%%%%%%%%%%%%%%%%%%%%%%% ALG: ISVIS %%%%%%%%%%%%%%%%%%%%%%%%%%%%%%%%%%%%%
\subsubsection{\textproc{IsVis}: \textit{Checks if a Target Node is Castable}}
The helper function \textproc{IsVis} (Alg. \ref{suppalg:isvis}) returns $\mtrue$ if a target-tree node is potentially visible from the traced position and can be cast to.
\begin{algorithm}[!ht]
\begin{algorithmic}[1]
\caption{\textproc{IsVis}: checks if a target node is potentially visible.}
\label{suppalg:isvis}
\Function{IsVis}{$\msidetrace, \mvpar, \mvnext$}  
    \Comment{Par. node is target-tree node.}
    \State \Return $\msidetrace (\mvpar \times \mvnext) \le 0$ \Comment{Assumes that trace has progressed w.r.t. target-tree node.}
\EndFunction
\end{algorithmic}
\end{algorithm}

%%%%%%%%%%%%%%%%%%%%%%%%%%%%%%%%% ALG: PLACENODE  %%%%%%%%%%%%%%%%%%%%%%%%%%%%%%%%%%%%%
\subsubsection{\textproc{PlaceNode}: \textit{Tries to Place a Node}}
The helper function \textproc{PlaceNode} (Alg. \ref{suppalg:placenode}) tries to place a turning point or phantom point.
A turning point ($\mnvu$ or $\mneu$-node) is placed if the current corner is convex, and the angular progression will reverse with respect to the source node.
A phantom point ($\mntm$-node) is placed if the current corner is non-convex, and the angular progression reverses with respect to at least one target node.
\begin{algorithm}[!ht]
\begin{algorithmic}[1]
\caption{\textproc{PlaceNode}: places a $\mntm$, $\mnvu$ or $\mneu$ node if possible.}
\label{suppalg:placenode}
\Function{PlaceNode}{$\mtdirpar, \mtrace = (\mxtrace, \msidetrace, \cdots)$}
    \State $\mvnext \gets $ \Call{GetEdge}{$\mxtrace, \msidetrace$}
    \State $\mnlet_\mnew = \varnothing$
    \For{$\mnlet \in \fnlets(\mtdirpar, \mtrace)$}
        % \State $(\sim, \sim, \mnodepar, \mvpar, \sim, \mvnext) \gets $\Call{TraceCalc}{$\mtrace, \mnlet$}
        \State $\mnodepar \gets \flink(\mnlet\mdot\mtlink)$
        \State $\mvpar \gets \mxtrace - \fx(\mnodepar)$
        
        \Comment{(A) Do not place if not prog. w.r.t. par. node, or ang. prog. increases at next edge.}
        \If {$\mcprog > 0$ \Or \Call{IsRev}{$\mtdirpar, \msidetrace, \mvpar, \mvnext$} = $\mfalse$}
            \State \Continue
        \EndIf

        \Comment{(B) Otherwise, place a new phantom ($\mntm$) or turning point ($\mneu$ or $\mnvu$).}
        \State $\mlink_\mathrm{newPar} \gets \mnlet\mdot\mtlink$
        \If {$\mnlet_\mnew = \varnothing$}
            \Comment{Create the new node and reuse current nodelet if new node not yet placed.}
            \State $\mnlet_\mnew \gets \mnlet$
            \State $\mntype_\mathrm{newPar} \gets \mnvu$
            \Comment{Determine the new node type.}
            \If {$\mtdirpar = T$}
                \State $\mntype_\mathrm{newPar} \gets \mntm$
            \ElsIf{$\mnodepar\mdot\mntype \in \{\mneu, \mney\}$}
                \State $\mntype_\mathrm{newPar} \gets \mneu$
            \EndIf
            \Comment{Create the new node and reuse current nodelet.}
            \State $\mnode_\mathrm{newPar} \gets $ \Call{GetNode}{$\mxtrace, \mntype_\mathrm{newPar}, \msidetrace, \mtdirpar$}
            \State $\mnlet_\mnew\mdot\mtlink \gets$ \Call{CreateLink}{$\ftnode(\mtdirpar, \mtrace)$}
            \State $\mnlet_\mnew\mdot\mvprog \gets \mvnext$
        \Else
            \Comment{Delete the nodelet if new node has been placed.}
            \State Remove $\mnlet$ from $\fnlets(\mtdirpar, \mtrace)$
        \EndIf

        \State \Call{Anchor}{$\mlink_\mathrm{newPar}, \mnode_\mathrm{newPar}$}
        \State $\mlink_\mathrm{newPar}\mdot c \gets$ \Call{Cost}{$\mlink_\mathrm{newPar}$}
        \State \Call{Connect}{$\mtdirpar, \mnlet_\mnew\mdot\mtlink, \mlink_\mathrm{newPar}$}
    \EndFor
    \State \Return $\mnlet_\mnew$
\EndFunction
\end{algorithmic}
\end{algorithm}

%%%%%%%%%%%%%%%%%%%%%%%%%%%%%%%%% ALG: CastFromTrace  %%%%%%%%%%%%%%%%%%%%%%%%%%%%%%%%%%%%%
\subsubsection{\textproc{CastFromTrace}: \textit{Tries to Cast From a Placed Turning Point.}}
The helper function \textproc{CastFromTrace} tries to cast to each target node after a turning point is placed at the current corner.
If castable, a casting query is queued for each target trace-link. The target trace-link is re-anchored on a target-tree $\mnvu$ node.
However, if the trace had crossed a path from a different query, it would have been marked for an overlap-rule check in \textproc{PlaceRule} (Alg. \ref{suppalg:placerule}). 
No new casting queries are queued by the trace, as the overlap-rule will queue a new casting query in the most recent source-tree node with cumulative visibility.
\begin{algorithm}[!ht]
\begin{algorithmic}[1]
\caption{\textproc{CastFromTrace}: tries to cast to all target nodes after placing a turning point.}
\label{suppalg:castfromtrace}
\Function{CastFromTrace}{$\mtrace=(\mxtrace, \msidetrace, \cdots), \mnlet_\mnew$}
    \State $\mvnext \gets $ \Call{GetEdge}{$\mxtrace, \msidetrace$}
    \State $\mlink_S \gets \flink(S, \mnlet_\mnew\mdot\mtlink)$
    \State $\mnode_S \gets \mnode(\mlink_S)$  
    \State $\mnode_\mathrm{newVu} \gets \varnothing$
    \For {$\mnlet_T \in \mtrace\mdot\mnlets_T$}

        \Comment{(A) For each target node, check if it is castable from new turning point at $\mx$.}
        % \State $(\sim, \sim, \mnodepar, \mvpar, \sim, \mvnext) \gets $\Call{TraceCalc}{$\mtrace, \mnlet_T$}
        \State $\mlink_\mathrm{newT} \gets \mnlet_T\mdot\mtlink$
        \State $\mnode_T \gets \fnode(\flink(T, \mlink_\mathrm{newT}))$
        \State $\mvpar \gets \mxtrace - \fx(\mnode_T)$
        % \If{$\mnlet_T\mdot\mcprog > 0$ \Or $\mnode_T\mdot\mntype = \mnph$ \Or \Call{IsVis}{$\msidetrace, \mvpar, \mvnext$} $= \mfalse$}
        %     \State \Continue 
        %     \Comment{Ignore target-tree node if not prog. w.r.t. node, node is $\mnph$, or node is not visible.}
        % \EndIf
        \If {\Call{IsVis}{$\msidetrace, \mvpar, \mvnext$} $= \mfalse$}
            \State \Continue 
            \Comment{Skip non-castable tgt node.}
        \EndIf
        
        \Comment{(B) Target node is castable, re-anchor target trace-link to target-tree $\mnvu$ node.}
        \If {$\mnode_\mathrm{newVu} = \varnothing$}
            \State $\mnode_\mathrm{newVu} \gets $ \Call{GetNode}{$\mxtrace, \mnvu, \msidetrace, T$}
        \EndIf
        \State \Call{Anchor}{$\mlink_\mathrm{newT}, \mnode_\mathrm{newVu}$}
        \State $\mlink_\mathrm{newT}\mdot\mcost \gets $ \Call{Cost}{$\mlink_\mathrm{newT}$}
        \State \Call{Connect}{$T, \mlink_S, \mlink_\mathrm{newT}$}

        \Comment{(C.1) Mark for overlap-rule if source node is expensive or trace crossed paths with other queries.}
        \If {$\mtrace\mdot\moverlap = \mtrue$ \Or $\mnode_S\mdot\mntype = \mneu$}
            \State $\mtrace\mdot\moverlap \gets \mfalse$
            \State \Call{PushOverlap}{\textproc{GetPos}($\mxtrace$)}
        
        \Comment{(C.2) Otherwise, queue a casting query.}
        \Else
            \State $f \gets \mlink_S\mdot\mcost + \mlink_\mathrm{newT}\mdot\mcost$ 
            \State \Call{Queue}{$\mqcast, f, \mlink_T'$}
        \EndIf
        \State Remove $\mnlet_T$ from $\mtrace\mdot\mnlets_T$
    \EndFor
\EndFunction

\end{algorithmic}
\end{algorithm}
